# Supplementary material for: How good are recent density functionals for ground and excited states of one-electron systems?
Source: arXiv:2208.06482 ancillary file (2022-11-08)
Supplement: Supplementary file 1 [file supplemental.pdf]

# Supplementary material: How good are recent density functionals for ground and excited one-electron systems?

Sebastian Schwalbe,[1, a)] Kai Trepte,[2, b)] and Susi Lehtola[3, c)]
[1)] *Institute of Theoretical Physics, TU Bergakademie Freiberg, D-09599 Freiberg, Germany*
[2)] *Taiwan Semiconductor Manufacturing Company North America, San Jose, CA 95134, USA*
[3)] *Molecular Sciences Software Institute, Blacksburg, VA 24061, USA*

(Dated: 8 November 2022)

## I. BASIS SET TRUNCATION ERRORS (BSTE)

We carried out fully numerical[1] Hartree–Fock and density functional calculations for the $1s$ state of various ions with the finite element method (FEM) using the HelFEM program[2–4]. The calculations employed 5 radial elements, affording $nE_\mathrm{h}$ level accuracy even for $\mathrm{Kr}^{35+}$. The basis set truncation error (BSTE) in the AHGBSP3-9 basis set, defined as the difference of the energy from the Gaussian-basis calculation with PySCF to that of the FEM calculation with HelFEM,

$$\Delta_n^{\mathrm{method/basis}} = E_n^{\mathrm{method/basis}} - E_n^{\mathrm{method/FEM}} \geq 0 \quad (1)$$

was determined for the $1s$ ground state of $Z^{(Z-1)+}$ for $Z \in [1, 36]$. The BSTE was determined for unrestricted Hartree–Fock (UHF) as well as the SPW92 and PBEsol functionals; the results are shown in figure S1. The average BSTE is similar for all three methods, i.e., $6.1 \times 10^{-7} E_\mathrm{h}$ for UHF, $6.0 \times 10^{-7} E_\mathrm{h}$ for SPW92, and $6.9 \times 10^{-7} E_\mathrm{h}$ for PBEsol, and the BSTE increases with increasing $Z$. Clearly, all the errors are below the aimed accuracy threshold of $5 \times 10^{-5} E_\mathrm{h}$.

The BSTEs for the $1s$, $2p$, and $3d$ states are studied at the UHF level of theory in figure S2. These results clearly show that the AHGBSP3-9 basis set used in all calculations of this work has uniform accuracy for all states.

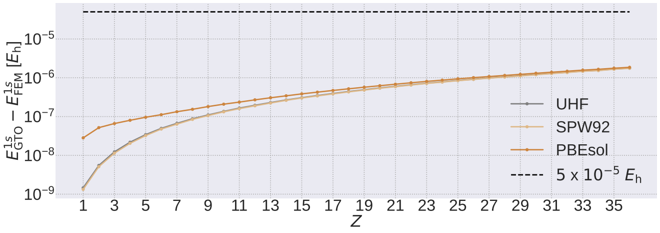


Figure S1. Basis set truncation error $E^{1s}_{\mathrm{GTO}} - E^{1s}_{\mathrm{FEM}}$ in the AHGBSP3-9 basis set for the $1s$ state in calculations performed with UHF compared to the SPW92 and PBEsol functionals. The UHF and SPW92 data are on top of each other.

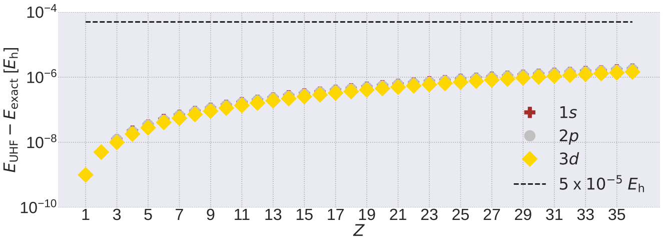


Figure S2. Basis set truncation errors $E_{\mathrm{UHF}} - E_{\mathrm{exact}}$ for the AHGBSP3-9 basis set for the $1s$, $2p$, and $3d$ states.

## II. FUNCTIONAL RANKINGS AND BAR CHARTS

A ranking of the functionals from best (lowest mean state error, MSE) to worst (largest MSE) for $1s$ states is given in table S1, for $2p$ states in table S2, and for $3d$ states in table S3. The ranking for the overall error (OE) is shown in table S4. The best performing functionals for the $1s$, $2s$, and $3d$ states as well as overall are summarized in table S5. To facilitate the visual interpretation of the MSEs, bar charts for the $1s$, $2s$, and $3d$ states are provided in figure S3: see figure 3(a) for $1s$, figure 3(b) for $2p$ and figure 3(c) for $3d$. A bar chart of the OE is given in figure S4.

## III. COMPARISON TO LITERATURE DATA FOR $1s$ STATES

A comparison to the results of Lonsdale and Goerigk[5] for the $1s$ state is shown table S6. As the study of Lonsdale and Goerigk[5] did not include K and Ca (see notes in Figs. 3 and 10 in Ref. 5), we exclude them for this comparison. Even though Lonsdale and Goerigk[5] used a different basis set and quadrature grid, our values are in reasonable agreement, with relative differences of only some percent for most functionals. The sole exception is the M11-L functional, for which the functional error reported in Lonsdale and Goerigk[5] is 13% smaller than what we find in this study.

Further study into this issue shows that the difference for M11-L is caused by the basis set: the unc-aug-cc-pVQZ basis was used in Ref. 5 while this work uses the AHGBSP3-9 basis set. The basis set dependence is studied in table S7 for HF and the PBE, TPSS, revTPSS, M06-L, M11-L, and B97M-V functionals using various

---

[a)]Electronic mail: schwalbe@physik.tu-freiberg.de
[b)]Electronic mail: kai.trepte1987@gmail.com
[c)]Electronic mail: susi.lehtola@alumni.helsinki.fi

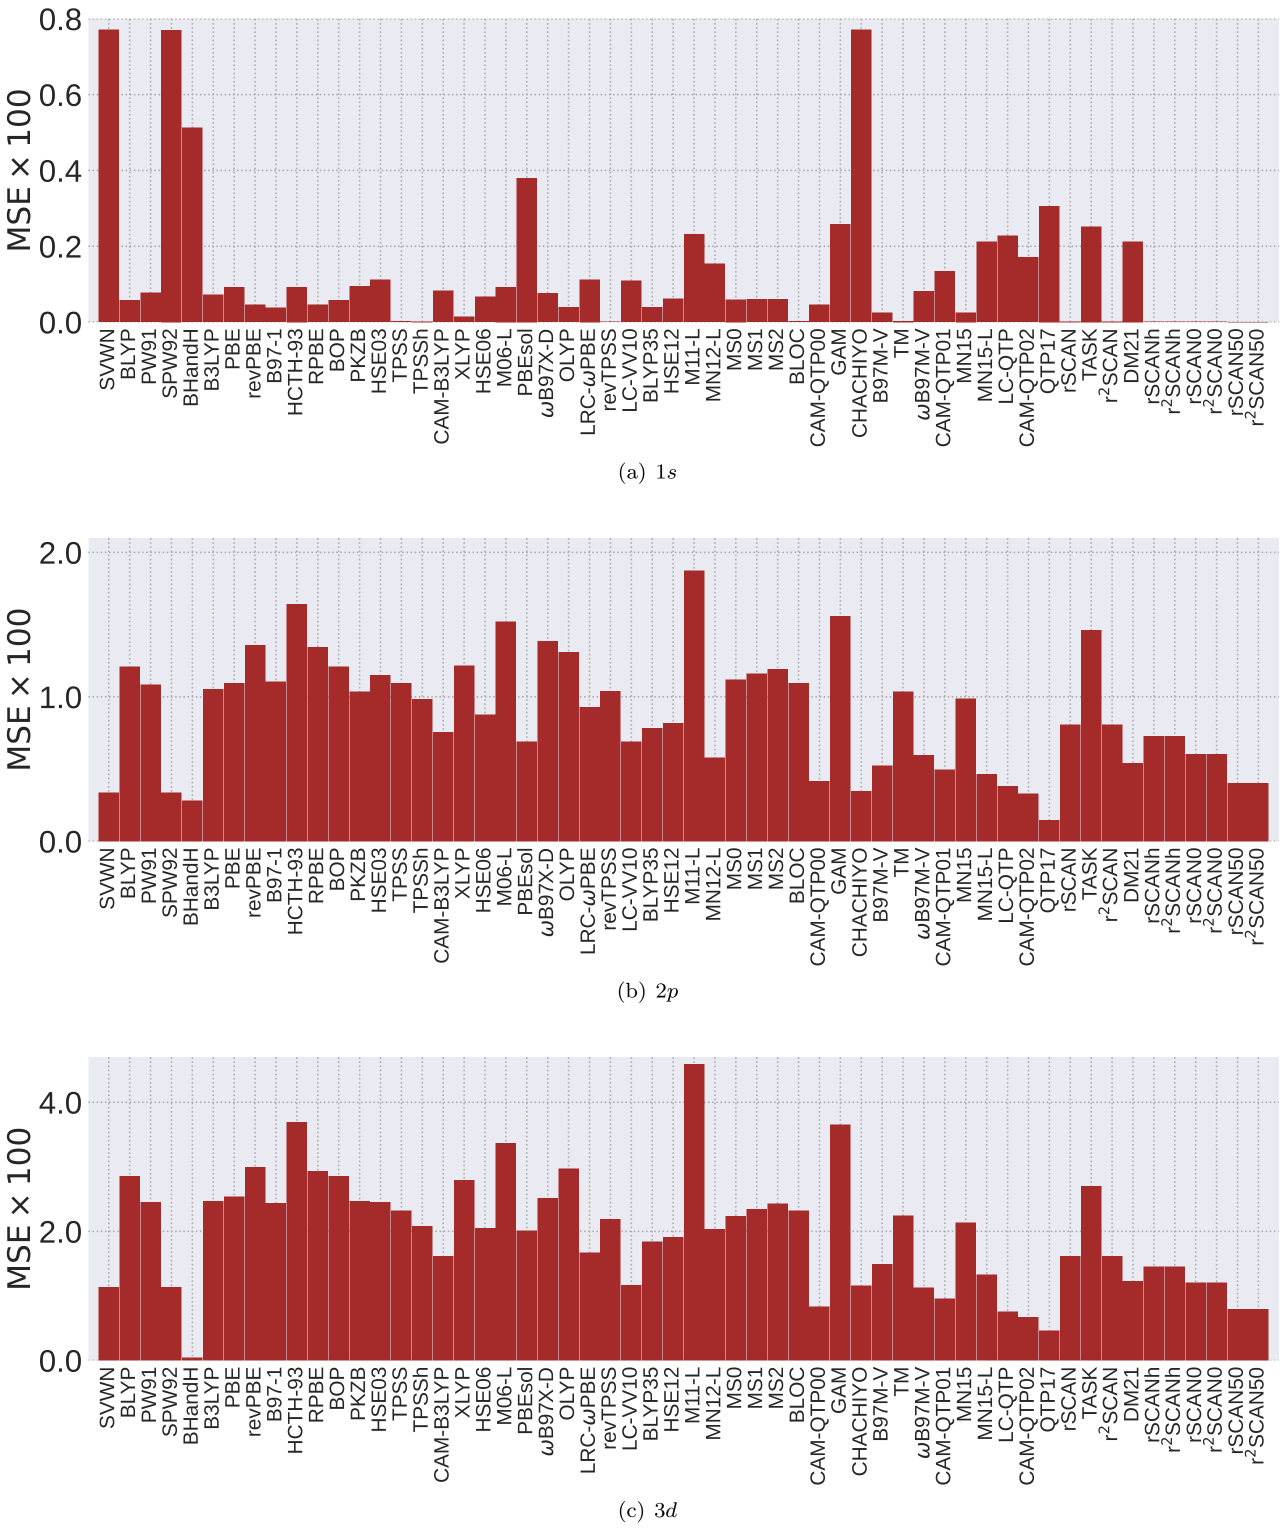


Figure S3. MSE for the $1s$, $2p$, and $3d$ states for 56 functionals.

augmented correlation consistent basis sets[6,7] in their uncontracted form (unc-aug-cc-pVXZ), augmented polarization consistent basis sets[8,9] in uncontracted form (unc-aug-pc-n) and the hydrogenic Gaussian basis set series[10] used in this work in both augmented and non-augmented form. For comparison, values computed with FEM[1–4] are also included for most functionals. FEM data is not available for M11-L as the calculations failed

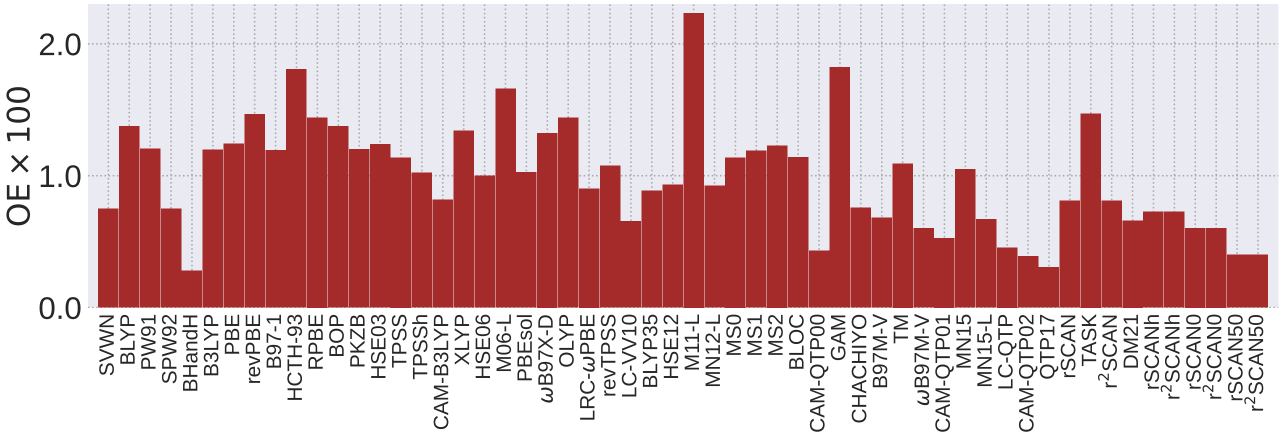


Figure S4. OE for 56 functionals.

to converge with this functional, nor for B97M-V which includes non-local correlation that is not available at the moment in HelFEM.

In all cases, the hydrogenic basis sets yield the lowest energies out of the Gaussian basis sets. Furthermore, the AHGBSP3-9 values are very close to FEM values except for M06-L, confirming the usefulness of the hydrogenic Gaussian basis sets for benchmark calculations.

The values from unc-aug-cc-pVQZ used by Lonsdale and Goerigk[5] and the AHGBSP3-9 basis used in this work differ by 51.7$\mu E_\mathrm{h}$ for HF, 56.0$\mu E_\mathrm{h}$ for PBE, 83.0$\mu E_\mathrm{h}$ for TPSS, and 70.8$\mu E_\mathrm{h}$ for revTPSS, with the values of this work being more converged to the basis set limit. The remaining three functionals are more basis set dependent: the values differ by 0.64$mE_\mathrm{h}$ for M06-L, 4.78$mE_\mathrm{h}$ for M11-L and 0.22$mE_\mathrm{h}$ for B97M-V. Because the density functionals already yield total energies that are too negative, the improvement in the accuracy of the basis set directly affect the error metric for the functionals.

M06-L and M11-L appear to be pathologically grid dependent, which is further supported by the FEM calculations: we were unable to converge M11-L with FEM, while M06-L shows an unexpectedly large difference of 0.29$mE_\mathrm{h}$ between the AHGBSP3-9 value and the FEM value.

Table S1. Functional ranking for the $1s$ state.

| Rank | name | MSE |
|---|---|---|
| 1 | rSCAN50 | $3.50360 \times 10^{-6}$ |
| 2 | r$^2$SCAN50 | $3.50360 \times 10^{-6}$ |
| 3 | rSCAN0 | $8.17282 \times 10^{-6}$ |
| 4 | r$^2$SCAN0 | $8.17282 \times 10^{-6}$ |
| 5 | rSCANh | $1.19764 \times 10^{-5}$ |
| 6 | r$^2$SCANh | $1.19764 \times 10^{-5}$ |
| 7 | revTPSS | $1.30215 \times 10^{-5}$ |
| 8 | rSCAN | $1.49476 \times 10^{-5}$ |
| 9 | r$^2$SCAN | $1.49476 \times 10^{-5}$ |
| 10 | TPSSh | $1.63969 \times 10^{-5}$ |
| 11 | TPSS | $2.04593 \times 10^{-5}$ |
| 12 | BLOC | $2.04593 \times 10^{-5}$ |
| 13 | TM | $2.97239 \times 10^{-5}$ |
| 14 | XLYP | $1.36933 \times 10^{-4}$ |
| 15 | B97M-V | $2.46572 \times 10^{-4}$ |
| 16 | MN15 | $2.53236 \times 10^{-4}$ |
| 17 | B97-1 | $3.75601 \times 10^{-4}$ |
| 18 | BLYP35 | $3.90195 \times 10^{-4}$ |
| 19 | OLYP | $3.93428 \times 10^{-4}$ |
| 20 | CAM-QTP00 | $4.57156 \times 10^{-4}$ |
| 21 | revPBE | $4.57184 \times 10^{-4}$ |
| 22 | RPBE | $4.57620 \times 10^{-4}$ |
| 23 | BOP | $5.78937 \times 10^{-4}$ |
| 24 | BLYP | $5.79016 \times 10^{-4}$ |
| 25 | MS0 | $5.97349 \times 10^{-4}$ |
| 26 | MS1 | $6.01296 \times 10^{-4}$ |
| 27 | MS2 | $6.03852 \times 10^{-4}$ |
| 28 | HSE12 | $6.18713 \times 10^{-4}$ |
| 29 | HSE06 | $6.65866 \times 10^{-4}$ |
| 30 | B3LYP | $7.20302 \times 10^{-4}$ |
| 31 | $\omega$B97X-D | $7.64133 \times 10^{-4}$ |
| 32 | PW91 | $7.77107 \times 10^{-4}$ |
| 33 | $\omega$B97M-V | $8.10571 \times 10^{-4}$ |
| 34 | CAM-B3LYP | $8.28601 \times 10^{-4}$ |
| 35 | PBE | $9.19590 \times 10^{-4}$ |
| 36 | M06-L | $9.24187 \times 10^{-4}$ |
| 37 | HCTH-93 | $9.25245 \times 10^{-4}$ |
| 38 | PKZB | $9.40815 \times 10^{-4}$ |
| 39 | LC-VV10 | $1.08863 \times 10^{-3}$ |
| 40 | HSE03 | $1.11584 \times 10^{-3}$ |
| 41 | LRC-$\omega$PBE | $1.12097 \times 10^{-3}$ |
| 42 | CAM-QTP01 | $1.33940 \times 10^{-3}$ |
| 43 | MN12-L | $1.54139 \times 10^{-3}$ |
| 44 | CAM-QTP02 | $1.71415 \times 10^{-3}$ |
| 45 | MN15-L | $2.11814 \times 10^{-3}$ |
| 46 | DM21 | $2.12615 \times 10^{-3}$ |
| 47 | LC-QTP | $2.27592 \times 10^{-3}$ |
| 48 | M11-L | $2.31957 \times 10^{-3}$ |
| 49 | TASK | $2.52305 \times 10^{-3}$ |
| 50 | GAM | $2.58402 \times 10^{-3}$ |
| 51 | QTP17 | $3.05967 \times 10^{-3}$ |
| 52 | PBEsol | $3.79913 \times 10^{-3}$ |
| 53 | BHandH | $5.12204 \times 10^{-3}$ |
| 54 | SPW92 | $7.70213 \times 10^{-3}$ |
| 55 | SVWN | $7.70663 \times 10^{-3}$ |
| 56 | CHACHIYO | $7.71101 \times 10^{-3}$ |

Table S2. Functional ranking for the $2p$ state.

| Rank | name | MSE |
|---|---|---|
| 1 | QTP17 | $1.48308 \times 10^{-3}$ |
| 2 | BHandH | $2.82212 \times 10^{-3}$ |
| 3 | CAM-QTP02 | $3.30177 \times 10^{-3}$ |
| 4 | SVWN | $3.39048 \times 10^{-3}$ |
| 5 | SPW92 | $3.39158 \times 10^{-3}$ |
| 6 | CHACHIYO | $3.47628 \times 10^{-3}$ |
| 7 | LC-QTP | $3.81790 \times 10^{-3}$ |
| 8 | rSCAN50 | $4.02520 \times 10^{-3}$ |
| 9 | r$^2$SCAN50 | $4.02520 \times 10^{-3}$ |
| 10 | CAM-QTP00 | $4.18668 \times 10^{-3}$ |
| 11 | MN15-L | $4.67326 \times 10^{-3}$ |
| 12 | CAM-QTP01 | $4.96132 \times 10^{-3}$ |
| 13 | B97M-V | $5.25842 \times 10^{-3}$ |
| 14 | DM21 | $5.43481 \times 10^{-3}$ |
| 15 | MN12-L | $5.79566 \times 10^{-3}$ |
| 16 | $\omega$B97M-V | $5.98667 \times 10^{-3}$ |
| 17 | r$^2$SCAN0 | $6.05130 \times 10^{-3}$ |
| 18 | rSCAN0 | $6.05130 \times 10^{-3}$ |
| 19 | LC-VV10 | $6.90531 \times 10^{-3}$ |
| 20 | PBEsol | $6.91813 \times 10^{-3}$ |
| 21 | rSCANh | $7.27136 \times 10^{-3}$ |
| 22 | r$^2$SCANh | $7.27136 \times 10^{-3}$ |
| 23 | CAM-B3LYP | $7.56898 \times 10^{-3}$ |
| 24 | BLYP35 | $7.82388 \times 10^{-3}$ |
| 25 | r$^2$SCAN | $8.08660 \times 10^{-3}$ |
| 26 | rSCAN | $8.08663 \times 10^{-3}$ |
| 27 | HSE12 | $8.20083 \times 10^{-3}$ |
| 28 | HSE06 | $8.78457 \times 10^{-3}$ |
| 29 | LRC-$\omega$PBE | $9.29420 \times 10^{-3}$ |
| 30 | TPSSh | $9.83474 \times 10^{-3}$ |
| 31 | MN15 | $9.86682 \times 10^{-3}$ |
| 32 | TM | $1.03542 \times 10^{-2}$ |
| 33 | PKZB | $1.03849 \times 10^{-2}$ |
| 34 | revTPSS | $1.04006 \times 10^{-2}$ |
| 35 | B3LYP | $1.05487 \times 10^{-2}$ |
| 36 | PW91 | $1.08639 \times 10^{-2}$ |
| 37 | TPSS | $1.09411 \times 10^{-2}$ |
| 38 | BLOC | $1.09412 \times 10^{-2}$ |
| 39 | PBE | $1.09609 \times 10^{-2}$ |
| 40 | B97-1 | $1.10771 \times 10^{-2}$ |
| 41 | MS0 | $1.12102 \times 10^{-2}$ |
| 42 | HSE03 | $1.15003 \times 10^{-2}$ |
| 43 | MS1 | $1.16142 \times 10^{-2}$ |
| 44 | MS2 | $1.19325 \times 10^{-2}$ |
| 45 | BLYP | $1.20855 \times 10^{-2}$ |
| 46 | BOP | $1.20858 \times 10^{-2}$ |
| 47 | XLYP | $1.21677 \times 10^{-2}$ |
| 48 | OLYP | $1.30932 \times 10^{-2}$ |
| 49 | RPBE | $1.34634 \times 10^{-2}$ |
| 50 | revPBE | $1.35781 \times 10^{-2}$ |
| 51 | $\omega$B97X-D | $1.38525 \times 10^{-2}$ |
| 52 | TASK | $1.46303 \times 10^{-2}$ |
| 53 | M06-L | $1.52055 \times 10^{-2}$ |
| 54 | GAM | $1.56102 \times 10^{-2}$ |
| 55 | HCTH-93 | $1.64193 \times 10^{-2}$ |
| 56 | M11-L | $1.87587 \times 10^{-2}$ |

Table S3. Functional ranking for the $3d$ state.

| Rank | name | MSE |
|---|---|---|
| 1 | BHandH | $4.34067 \times 10^{-4}$ |
| 2 | QTP17 | $4.61151 \times 10^{-3}$ |
| 3 | CAM-QTP02 | $6.67966 \times 10^{-3}$ |
| 4 | LC-QTP | $7.59034 \times 10^{-3}$ |
| 5 | r$^2$SCAN50 | $7.97455 \times 10^{-3}$ |
| 6 | rSCAN50 | $7.97462 \times 10^{-3}$ |
| 7 | CAM-QTP00 | $8.30036 \times 10^{-3}$ |
| 8 | CAM-QTP01 | $9.54244 \times 10^{-3}$ |
| 9 | $\omega$B97M-V | $1.12842 \times 10^{-2}$ |
| 10 | SVWN | $1.13776 \times 10^{-2}$ |
| 11 | SPW92 | $1.13776 \times 10^{-2}$ |
| 12 | CHACHIYO | $1.15484 \times 10^{-2}$ |
| 13 | LC-VV10 | $1.16636 \times 10^{-2}$ |
| 14 | rSCAN0 | $1.20440 \times 10^{-2}$ |
| 15 | r$^2$SCAN0 | $1.20440 \times 10^{-2}$ |
| 16 | DM21 | $1.22576 \times 10^{-2}$ |
| 17 | MN15-L | $1.32741 \times 10^{-2}$ |
| 18 | rSCANh | $1.45137 \times 10^{-2}$ |
| 19 | r$^2$SCANh | $1.45137 \times 10^{-2}$ |
| 20 | B97M-V | $1.49072 \times 10^{-2}$ |
| 21 | CAM-B3LYP | $1.61660 \times 10^{-2}$ |
| 22 | r$^2$SCAN | $1.61722 \times 10^{-2}$ |
| 23 | rSCAN | $1.61723 \times 10^{-2}$ |
| 24 | LRC-$\omega$PBE | $1.66828 \times 10^{-2}$ |
| 25 | BLYP35 | $1.83694 \times 10^{-2}$ |
| 26 | HSE12 | $1.91080 \times 10^{-2}$ |
| 27 | PBEsol | $2.00980 \times 10^{-2}$ |
| 28 | MN12-L | $2.03637 \times 10^{-2}$ |
| 29 | HSE06 | $2.05180 \times 10^{-2}$ |
| 30 | TPSSh | $2.07984 \times 10^{-2}$ |
| 31 | MN15 | $2.13324 \times 10^{-2}$ |
| 32 | revTPSS | $2.18584 \times 10^{-2}$ |
| 33 | MS0 | $2.23280 \times 10^{-2}$ |
| 34 | TM | $2.23954 \times 10^{-2}$ |
| 35 | TPSS | $2.31835 \times 10^{-2}$ |
| 36 | BLOC | $2.32046 \times 10^{-2}$ |
| 37 | MS1 | $2.34581 \times 10^{-2}$ |
| 38 | MS2 | $2.43222 \times 10^{-2}$ |
| 39 | B97-1 | $2.43628 \times 10^{-2}$ |
| 40 | PW91 | $2.44853 \times 10^{-2}$ |
| 41 | HSE03 | $2.45339 \times 10^{-2}$ |
| 42 | B3LYP | $2.46448 \times 10^{-2}$ |
| 43 | PKZB | $2.47013 \times 10^{-2}$ |
| 44 | $\omega$B97X-D | $2.51154 \times 10^{-2}$ |
| 45 | PBE | $2.53799 \times 10^{-2}$ |
| 46 | TASK | $2.69819 \times 10^{-2}$ |
| 47 | XLYP | $2.79232 \times 10^{-2}$ |
| 48 | BLYP | $2.85655 \times 10^{-2}$ |
| 49 | BOP | $2.85677 \times 10^{-2}$ |
| 50 | RPBE | $2.93201 \times 10^{-2}$ |
| 51 | OLYP | $2.97062 \times 10^{-2}$ |
| 52 | revPBE | $2.99502 \times 10^{-2}$ |
| 53 | M06-L | $3.36828 \times 10^{-2}$ |
| 54 | GAM | $3.64957 \times 10^{-2}$ |
| 55 | HCTH-93 | $3.68895 \times 10^{-2}$ |
| 56 | M11-L | $4.59323 \times 10^{-2}$ |

Table S4. Functional ranking for the overall error.

| Rank | name | OE |
|---|---|---|
| 1 | BHandH | $2.79274 \times 10^{-3}$ |
| 2 | QTP17 | $3.05142 \times 10^{-3}$ |
| 3 | CAM-QTP02 | $3.89853 \times 10^{-3}$ |
| 4 | r$^2$SCAN50 | $4.00108 \times 10^{-3}$ |
| 5 | rSCAN50 | $4.00111 \times 10^{-3}$ |
| 6 | CAM-QTP00 | $4.31473 \times 10^{-3}$ |
| 7 | LC-QTP | $4.56139 \times 10^{-3}$ |
| 8 | CAM-QTP01 | $5.28105 \times 10^{-3}$ |
| 9 | $\omega$B97M-V | $6.02715 \times 10^{-3}$ |
| 10 | rSCAN0 | $6.03450 \times 10^{-3}$ |
| 11 | r$^2$SCAN0 | $6.03450 \times 10^{-3}$ |
| 12 | LC-VV10 | $6.55252 \times 10^{-3}$ |
| 13 | DM21 | $6.60619 \times 10^{-3}$ |
| 14 | MN15-L | $6.68850 \times 10^{-3}$ |
| 15 | B97M-V | $6.80408 \times 10^{-3}$ |
| 16 | rSCANh | $7.26567 \times 10^{-3}$ |
| 17 | r$^2$SCANh | $7.26568 \times 10^{-3}$ |
| 18 | SPW92 | $7.49045 \times 10^{-3}$ |
| 19 | SVWN | $7.49158 \times 10^{-3}$ |
| 20 | CHACHIYO | $7.57857 \times 10^{-3}$ |
| 21 | r$^2$SCAN | $8.09124 \times 10^{-3}$ |
| 22 | rSCAN | $8.09128 \times 10^{-3}$ |
| 23 | CAM-B3LYP | $8.18785 \times 10^{-3}$ |
| 24 | BLYP35 | $8.86117 \times 10^{-3}$ |
| 25 | LRC-$\omega$PBE | $9.03267 \times 10^{-3}$ |
| 26 | MN12-L | $9.23357 \times 10^{-3}$ |
| 27 | HSE12 | $9.30918 \times 10^{-3}$ |
| 28 | HSE06 | $9.98947 \times 10^{-3}$ |
| 29 | TPSSh | $1.02165 \times 10^{-2}$ |
| 30 | PBEsol | $1.02717 \times 10^{-2}$ |
| 31 | MN15 | $1.04841 \times 10^{-2}$ |
| 32 | revTPSS | $1.07573 \times 10^{-2}$ |
| 33 | TM | $1.09264 \times 10^{-2}$ |
| 34 | MS0 | $1.13785 \times 10^{-2}$ |
| 35 | TPSS | $1.13817 \times 10^{-2}$ |
| 36 | BLOC | $1.13887 \times 10^{-2}$ |
| 37 | MS1 | $1.18912 \times 10^{-2}$ |
| 38 | B97-1 | $1.19385 \times 10^{-2}$ |
| 39 | B3LYP | $1.19713 \times 10^{-2}$ |
| 40 | PKZB | $1.20090 \times 10^{-2}$ |
| 41 | PW91 | $1.20421 \times 10^{-2}$ |
| 42 | MS2 | $1.22862 \times 10^{-2}$ |
| 43 | HSE03 | $1.23833 \times 10^{-2}$ |
| 44 | PBE | $1.24201 \times 10^{-2}$ |
| 45 | $\omega$B97X-D | $1.32440 \times 10^{-2}$ |
| 46 | XLYP | $1.34093 \times 10^{-2}$ |
| 47 | BLYP | $1.37433 \times 10^{-2}$ |
| 48 | BOP | $1.37442 \times 10^{-2}$ |
| 49 | OLYP | $1.43976 \times 10^{-2}$ |
| 50 | RPBE | $1.44137 \times 10^{-2}$ |
| 51 | revPBE | $1.46618 \times 10^{-2}$ |
| 52 | TASK | $1.47118 \times 10^{-2}$ |
| 53 | M06-L | $1.66042 \times 10^{-2}$ |
| 54 | HCTH-93 | $1.80780 \times 10^{-2}$ |
| 55 | GAM | $1.82300 \times 10^{-2}$ |
| 56 | M11-L | $2.23369 \times 10^{-2}$ |

Table S5. Best performing functionals on various rungs of Jacob's ladder for the $1s$, $2s$, and $3d$ states as well as for the overall error.

| Rung | $1s$ | $2p$ | $3d$ | OE |
|---|---|---|---|---|
| LDA | SPW92 | SVWN | SVWN | SPW92 |
| GGA | XLYP | PBEsol | PBEsol | PBEsol |
| mGGA | revTPSS | MN15-L | MN15-L | MN15-L |
| HYB | rSCAN50 | QTP17 | BHandH | BHandH |
| best | rSCAN50 | QTP17 | BHandH | BHandH |

Table S6. Comparison of results for the $1s$ state of the present work (PW) with the corresponding values of Lonsdale and Goerigk (LG) from Ref. 5. Note that we used our MSE definition for PW and LG, which is unitless. In addition, the absolute percentage error APE = $|((\mathrm{LG}-\mathrm{PW})/\mathrm{PW})| \times 100\%$ is reported.

| Name | PW | LG | APE [%] |
|---|---|---|---|
| $\omega$B97M-V | $8.38819 \times 10^{-4}$ | $8.45138 \times 10^{-4}$ | $7.53297 \times 10^{-1}$ |
| B3LYP | $7.34235 \times 10^{-4}$ | $7.33884 \times 10^{-4}$ | $4.78058 \times 10^{-2}$ |
| B97M-V | $2.51475 \times 10^{-4}$ | $2.40834 \times 10^{-4}$ | $4.23138 \times 10^{+0}$ |
| BLYP | $5.96690 \times 10^{-4}$ | $5.97700 \times 10^{-4}$ | $1.69320 \times 10^{-1}$ |
| BOP | $5.96606 \times 10^{-4}$ | $5.97700 \times 10^{-4}$ | $1.83362 \times 10^{-1}$ |
| CAM-B3LYP | $8.57296 \times 10^{-4}$ | $8.59052 \times 10^{-4}$ | $2.04817 \times 10^{-1}$ |
| CAM-QTP01 | $1.39300 \times 10^{-3}$ | $1.39894 \times 10^{-3}$ | $4.26966 \times 10^{-1}$ |
| LC-VV10 | $1.11388 \times 10^{-3}$ | $1.11421 \times 10^{-3}$ | $2.94155 \times 10^{-2}$ |
| M06-L | $9.56792 \times 10^{-4}$ | $8.96672 \times 10^{-4}$ | $6.28347 \times 10^{+0}$ |
| M11-L | $2.38770 \times 10^{-3}$ | $2.07624 \times 10^{-3}$ | $1.30443 \times 10^{+1}$ |
| MN12-L | $1.58625 \times 10^{-3}$ | $1.59771 \times 10^{-3}$ | $7.22445 \times 10^{-1}$ |
| MN15 | $2.65522 \times 10^{-4}$ | $2.68544 \times 10^{-4}$ | $1.13808 \times 10^{+0}$ |
| MN15-L | $2.11663 \times 10^{-3}$ | $2.12399 \times 10^{-3}$ | $3.47704 \times 10^{-1}$ |
| OLYP | $4.05202 \times 10^{-4}$ | $4.08339 \times 10^{-4}$ | $7.74255 \times 10^{-1}$ |
| PBE | $9.36214 \times 10^{-4}$ | $9.37613 \times 10^{-4}$ | $1.49389 \times 10^{-1}$ |
| PW91 | $7.92250 \times 10^{-4}$ | $7.89482 \times 10^{-4}$ | $3.49454 \times 10^{-1}$ |
| RPBE | $4.78756 \times 10^{-4}$ | $4.74266 \times 10^{-4}$ | $9.37818 \times 10^{-1}$ |
| SPW92 | $7.90560 \times 10^{-3}$ | $8.04315 \times 10^{-3}$ | $1.73997 \times 10^{+0}$ |
| SVWN | $7.91033 \times 10^{-3}$ | $8.04820 \times 10^{-3}$ | $1.74285 \times 10^{+0}$ |
| TPSS | $2.15980 \times 10^{-5}$ | $2.01696 \times 10^{-5}$ | $6.61361 \times 10^{+0}$ |
| TPSSh | $1.73088 \times 10^{-5}$ | $1.62511 \times 10^{-5}$ | $6.11062 \times 10^{+0}$ |
| revPBE | $4.74206 \times 10^{-4}$ | $4.71561 \times 10^{-4}$ | $5.57747 \times 10^{-1}$ |
| revTPSS | $1.37720 \times 10^{-5}$ | $1.29575 \times 10^{-5}$ | $5.91392 \times 10^{+0}$ |

Table S7. Total energies for the H atom in $E_\mathrm{h}$ with various functionals and basis sets. N/C denotes no convergence, N/A denotes data that is unavailable.

| Basis | HF | PBE | TPSS | revTPSS | M06-L | M11-L | B97M-V |
|---|---|---|---|---|---|---|---|
| unc-aug-cc-pVDZ | −0.4993370 | −0.4993541 | −0.4996426 | −0.4995471 | −0.5016969 | −0.5047850 | −0.5002878 |
| unc-aug-cc-pVTZ | −0.4998213 | −0.4998045 | −0.5000336 | −0.4999786 | −0.5037034 | −0.5065771 | −0.5011197 |
| unc-aug-cc-pVQZ | −0.4999483 | −0.4999343 | −0.5001523 | −0.5000867 | −0.5040585 | −0.5055703 | −0.5013528 |
| unc-aug-cc-pV5Z | −0.4999948 | −0.4999851 | −0.5002286 | −0.5001484 | −0.5041979 | −0.5083504 | −0.5015100 |
| unc-aug-cc-pV6Z | −0.4999993 | −0.4999891 | −0.5002296 | −0.5001547 | −0.5042778 | −0.5094547 | −0.5015454 |
| unc-aug-pc-1 | −0.4990825 | −0.4992426 | −0.4995182 | −0.4993989 | −0.5011977 | −0.5046313 | −0.5001773 |
| unc-aug-pc-2 | −0.4999230 | −0.4999238 | −0.5001450 | −0.5000745 | −0.5040151 | −0.5057888 | −0.5013461 |
| unc-aug-pc-3 | −0.4999974 | −0.4999862 | −0.5002260 | −0.5001535 | −0.5040242 | −0.5083743 | −0.5014725 |
| unc-aug-pc-4 | −0.4999996 | −0.4999898 | −0.5002315 | −0.5001537 | −0.5041838 | −0.5084006 | −0.5015613 |
| HGBSP3-5 | −0.4999890 | −0.4999538 | −0.5001914 | −0.5001127 | −0.5042079 | −0.5091005 | −0.5015337 |
| HGBSP3-7 | −0.4999999 | −0.4999890 | −0.5002324 | −0.5001554 | −0.5044240 | −0.5098696 | −0.5015681 |
| HGBSP3-9 | −0.5000000 | −0.4999903 | −0.5002352 | −0.5001574 | −0.5046958 | −0.5103216 | −0.5015712 |
| AHGBSP3-5 | −0.4999898 | −0.4999815 | −0.5002193 | −0.5001407 | −0.5043017 | −0.5092270 | −0.5015443 |
| AHGBSP3-7 | −0.4999999 | −0.4999900 | −0.5002328 | −0.5001558 | −0.5044442 | −0.5099261 | −0.5015715 |
| AHGBSP3-9 | −0.5000000 | −0.4999903 | −0.5002353 | −0.5001575 | −0.5046959 | −0.5103507 | −0.5015714 |
| FEM | −0.5000000 | −0.4999904 | −0.5002355 | −0.5001577 | −0.5049877 | N/C | N/A |

## IV. TOTAL ENERGIES

The total energies for all methods, atoms and states computed in the AHGBSP3-9 basis set are shown in tables; see the list of tables below.

## LIST OF TABLES


S1 Functional ranking for the 1$s$ state. . . . . . . . 4
S2 Functional ranking for the 2$p$ state. . . . . . . . 4
S3 Functional ranking for the 3$d$ state. . . . . . . . 5
S4 Functional ranking for the overall error. . . . 5
S5 Best performing functionals . . . . . . . . . . . . . . 6
S6 1$s$ state literature comparison . . . . . . . . . . . . 6
S7 Total energies for the H atom . . . . . . . . . . . . 7
S8 Total energies for SVWN . . . . . . . . . . . . . . . . 9
S9 Total energies for BLYP . . . . . . . . . . . . . . . . . 10
S10 Total energies for PW91 . . . . . . . . . . . . . . . . 11
S11 Total energies for SPW92 . . . . . . . . . . . . . . . 12
S12 Total energies for BHandH . . . . . . . . . . . . . . 13
S13 Total energies for B3LYP . . . . . . . . . . . . . . . 14
S14 Total energies for PBE . . . . . . . . . . . . . . . . . 15
S15 Total energies for revPBE . . . . . . . . . . . . . . . 16
S16 Total energies for B97-1 . . . . . . . . . . . . . . . . 17
S17 Total energies for HCTH-93 . . . . . . . . . . . . . 18
S18 Total energies for RPBE . . . . . . . . . . . . . . . . 19
S19 Total energies for BOP . . . . . . . . . . . . . . . . . 20
S20 Total energies for PKZB . . . . . . . . . . . . . . . . 21
S21 Total energies for HSE03 . . . . . . . . . . . . . . . 22
S22 Total energies for TPSS . . . . . . . . . . . . . . . . 23
S23 Total energies for TPSSh . . . . . . . . . . . . . . . 24
S24 Total energies for CAM-B3LYP . . . . . . . . . . 25
S25 Total energies for XLYP . . . . . . . . . . . . . . . . 26
S26 Total energies for HSE06 . . . . . . . . . . . . . . . 27
S27 Total energies for M06-L . . . . . . . . . . . . . . . 28
S28 Total energies for PBEsol . . . . . . . . . . . . . . . 29
S29 Total energies for $\omega$B97X-D . . . . . . . . . . . . . 30
S30 Total energies for OLYP . . . . . . . . . . . . . . . 31
S31 Total energies for LRC-$\omega$PBE . . . . . . . . . . . . 32
S32 Total energies for revTPSS . . . . . . . . . . . . . 33
S33 Total energies for LC-VV10 . . . . . . . . . . . . . 34
S34 Total energies for BLYP35 . . . . . . . . . . . . . . 35
S35 Total energies for HSE12 . . . . . . . . . . . . . . . 36
S36 Total energies for M11-L . . . . . . . . . . . . . . . 37
S37 Total energies for MN12-L . . . . . . . . . . . . . . 38
S38 Total energies for MS0 . . . . . . . . . . . . . . . . . 39
S39 Total energies for MS1 . . . . . . . . . . . . . . . . . 40
S40 Total energies for MS2 . . . . . . . . . . . . . . . . . 41
S41 Total energies for BLOC . . . . . . . . . . . . . . . . 42
S42 Total energies for CAM-QTP00 . . . . . . . . . . 43
S43 Total energies for GAM . . . . . . . . . . . . . . . . 44
S44 Total energies for CHACHIYO . . . . . . . . . . . 45
S45 Total energies for B97M-V . . . . . . . . . . . . . . 46
S46 Total energies for TM . . . . . . . . . . . . . . . . . . 47
S47 Total energies for $\omega$B97M-V . . . . . . . . . . . . 48
S48 Total energies for CAM-QTP01 . . . . . . . . . . 49
S49 Total energies for MN15 . . . . . . . . . . . . . . . . 50
S50 Total energies for MN15-L . . . . . . . . . . . . . . 51
S51 Total energies for LC-QTP . . . . . . . . . . . . . . 52
S52 Total energies for CAM-QTP02 . . . . . . . . . . 53
S53 Total energies for QTP17 . . . . . . . . . . . . . . . 54
S54 Total energies for rSCAN . . . . . . . . . . . . . . . 55
S55 Total energies for TASK . . . . . . . . . . . . . . . . 56
S56 Total energies for r$^2$SCAN . . . . . . . . . . . . . . 57
S57 Total energies for DM21 . . . . . . . . . . . . . . . . 58
S58 Total energies for rSCANh . . . . . . . . . . . . . . 59
S59 Total energies for r$^2$SCANh . . . . . . . . . . . . . 60
S60 Total energies for rSCAN0 . . . . . . . . . . . . . . 61
S61 Total energies for r$^2$SCAN0 . . . . . . . . . . . . . 62
S62 Total energies for rSCAN50 . . . . . . . . . . . . . 63
S63 Total energies for r$^2$SCAN50 . . . . . . . . . . . . 64
S64 Total energies for UHF . . . . . . . . . . . . . . . . . 65



[1] S. Lehtola, "A review on non-relativistic, fully numerical electronic structure calculations on atoms and diatomic molecules," Int. J. Quantum Chem. **119**, e25968 (2019), arXiv:1902.01431.
[2] S. Lehtola. HelFEM – Helsinki Finite Element Suite for atoms and diatomic molecules, "`https://github.com/susilehtola/HelFEM`," (2018).
[3] S. Lehtola, "Fully numerical Hartree–Fock and density functional calculations. I. Atoms," Int. J. Quantum Chem. **119**, e25945 (2019), arXiv:1810.11651.
[4] S. Lehtola, "Fully numerical calculations on atoms with fractional occupations and range-separated exchange functionals," Phys. Rev. A **101**, 012516 (2020), arXiv:1908.02528.
[5] D. R. Lonsdale and L. Goerigk, "The one-electron self-interaction error in 74 density functional approximations: a case study on hydrogenic mono- and dinuclear systems," Phys. Chem. Chem. Phys. **22**, 15805–15830 (2020).
[6] T. H. Dunning, "Gaussian basis sets for use in correlated molecular calculations. I. The atoms boron through neon and hydrogen," J. Chem. Phys. **90**, 1007 (1989).
[7] R. A. Kendall, T. H. Dunning, and R. J. Harrison, "Electron affinities of the first-row atoms revisited. Systematic basis sets and wave functions," J. Chem. Phys. **96**, 6796 (1992).
[8] F. Jensen, "Polarization consistent basis sets: Principles," J. Chem. Phys. **115**, 9113–9125 (2001).
[9] F. Jensen, "Polarization consistent basis sets. III. The importance of diffuse functions," J. Chem. Phys. **117**, 9234–9240 (2002).
[10] S. Lehtola, "Polarized Gaussian basis sets from one-electron ions," J. Chem. Phys. **152**, 134108 (2020), arXiv:2001.04224.

Table S8. Total energies for SVWN for the $1s$, $2p$, and $3d$ states calculated with PySCF using exponents from the AHGBSP3-9 basis set.

| System | $E_{\mathrm{tot}}^{1s}$ [$E_{\mathrm{h}}$] | $E_{\mathrm{tot}}^{2p}$ [$E_{\mathrm{h}}$] | $E_{\mathrm{tot}}^{3d}$ [$E_{\mathrm{h}}$] |
|---|---|---|---|
| $H^{0}$ | -0.4786708 | -0.1321379 | -0.0653143 |
| $He^{+}$ | -1.9417028 | -0.5066166 | -0.2366249 |
| $Li^{2+}$ | -4.4020529 | -1.1293424 | -0.5179029 |
| $Be^{3+}$ | -7.8611726 | -2.0011983 | -0.9096469 |
| $B^{4+}$ | -12.3195752 | -3.1225135 | -1.4120976 |
| $C^{5+}$ | -17.7775052 | -4.4934633 | -2.0253764 |
| $N^{6+}$ | -24.2350992 | -6.1141484 | -2.7495551 |
| $O^{7+}$ | -31.6924414 | -7.9846310 | -3.5846781 |
| $F^{8+}$ | -40.1495877 | -10.1049539 | -4.5307815 |
| $Ne^{9+}$ | -49.6065772 | -12.4751490 | -5.5782056 |
| $Na^{10+}$ | -60.0634381 | -15.0952381 | -6.7560229 |
| $Mg^{11+}$ | -71.5201916 | -17.9652313 | -8.0352304 |
| $Al^{12+}$ | -83.9768540 | -21.0851516 | -9.4254110 |
| $Si^{13+}$ | -97.4334383 | -24.4549860 | -10.9266527 |
| $P^{14+}$ | -111.8899546 | -28.0747908 | -12.5389749 |
| $S^{15+}$ | -127.3464115 | -31.9445370 | -14.2623733 |
| $Cl^{16+}$ | -143.8028157 | -36.0642325 | -16.0968348 |
| $Ar^{17+}$ | -161.2591730 | -40.4338871 | -18.0423843 |
| $K^{18+}$ | -179.7154883 | -45.0535404 | -20.0990552 |
| $Ca^{19+}$ | -199.1717657 | -49.9230800 | -22.2667663 |
| $Sc^{20+}$ | -219.6280088 | -55.0426327 | -24.5454842 |
| $Ti^{21+}$ | -241.0842206 | -60.4121433 | -26.9353793 |
| $V^{22+}$ | -263.5404039 | -66.0316704 | -29.4363116 |
| $Cr^{23+}$ | -286.9965609 | -71.9011427 | -32.0483966 |
| $Mn^{24+}$ | -311.4526937 | -78.0206037 | -34.7715298 |
| $Fe^{25+}$ | -336.9088042 | -84.3900249 | -37.6057355 |
| $Co^{26+}$ | -363.3648940 | -91.0094498 | -40.5510935 |
| $Ni^{27+}$ | -390.8209646 | -97.8788565 | -43.6075181 |
| $Cu^{28+}$ | -419.2770172 | -104.9982059 | -46.7749980 |
| $Zn^{29+}$ | -448.7330530 | -112.3675992 | -50.0536681 |
| $Ga^{30+}$ | -479.1890730 | -119.9869628 | -53.4433492 |
| $Ge^{31+}$ | -510.6450784 | -127.8563037 | -56.9441900 |
| $As^{32+}$ | -543.1010699 | -135.9756319 | -60.5561053 |
| $Se^{33+}$ | -576.5570483 | -144.3449482 | -64.2790861 |
| $Br^{34+}$ | -611.0130144 | -152.9642532 | -68.1132117 |
| $Kr^{35+}$ | -646.4689688 | -161.8335384 | -72.0584554 |

Table S9. Total energies for BLYP for the 1$s$, 2$p$, and 3$d$ states calculated with PySCF using exponents from the AHGBSP3-9 basis set.

| System | $E^{1s}_{\mathrm{tot}}$ [$E_\mathrm{h}$] | $E^{2p}_{\mathrm{tot}}$ [$E_\mathrm{h}$] | $E^{3d}_{\mathrm{tot}}$ [$E_\mathrm{h}$] |
|---|---|---|---|
| $H^{0}$ | -0.4979143 | -0.1382596 | -0.0699032 |
| $He^{+}$ | -1.9951314 | -0.5261199 | -0.2498920 |
| $Li^{2+}$ | -4.4923754 | -1.1640612 | -0.5409449 |
| $Be^{3+}$ | -7.9896254 | -2.0519227 | -0.9431694 |
| $B^{4+}$ | -12.4868776 | -3.1897948 | -1.4564914 |
| $C^{5+}$ | -17.9841310 | -4.5776958 | -2.0809189 |
| $N^{6+}$ | -24.4813850 | -6.2155895 | -2.8164458 |
| $O^{7+}$ | -31.9786394 | -8.1034644 | -3.6631130 |
| $F^{8+}$ | -40.4758941 | -10.2413516 | -4.6209083 |
| $Ne^{9+}$ | -49.9731489 | -12.6292240 | -5.6781892 |
| $Na^{10+}$ | -60.4704039 | -15.2669316 | -6.8697049 |
| $Mg^{11+}$ | -71.9676589 | -18.1550058 | -8.1607900 |
| $Al^{12+}$ | -84.4649140 | -21.2926643 | -9.5629858 |
| $Si^{13+}$ | -97.9621692 | -24.6808653 | -11.0763066 |
| $P^{14+}$ | -112.4594244 | -28.3185941 | -12.7007478 |
| $S^{15+}$ | -127.9566797 | -32.2062675 | -14.4363263 |
| $Cl^{16+}$ | -144.4539350 | -36.3441352 | -16.2831359 |
| $Ar^{17+}$ | -161.9511903 | -40.7320029 | -18.2407106 |
| $K^{18+}$ | -180.4484456 | -45.3703218 | -20.3098785 |
| $Ca^{19+}$ | -199.9457010 | -50.2580634 | -22.4897061 |
| $Sc^{20+}$ | -220.4429563 | -55.3959541 | -24.7806880 |
| $Ti^{21+}$ | -241.9402117 | -60.7839968 | -27.1820828 |
| $V^{22+}$ | -264.4374671 | -66.4213414 | -29.6962773 |
| $Cr^{23+}$ | -287.9347225 | -72.3096285 | -32.3209711 |
| $Mn^{24+}$ | -312.4319779 | -78.4470768 | -35.0552597 |
| $Fe^{25+}$ | -337.9292333 | -84.8353966 | -37.9032381 |
| $Co^{26+}$ | -364.4264887 | -91.4731777 | -40.8596000 |
| $Ni^{27+}$ | -391.9237441 | -98.3606799 | -43.9284368 |
| $Cu^{28+}$ | -420.4209995 | -105.4992367 | -47.1093714 |
| $Zn^{29+}$ | -449.9182549 | -112.8871278 | -50.4003880 |
| $Ga^{30+}$ | -480.4155103 | -120.5242830 | -53.8028639 |
| $Ge^{31+}$ | -511.9127657 | -128.4121507 | -57.3148951 |
| $As^{32+}$ | -544.4100211 | -136.5500184 | -60.9392874 |
| $Se^{33+}$ | -577.9072766 | -144.9378861 | -64.6759113 |
| $Br^{34+}$ | -612.4045320 | -153.5757538 | -68.5226543 |
| $Kr^{35+}$ | -647.9017874 | -162.4639900 | -72.4791311 |

Table S10. Total energies for PW91 for the $1s$, $2p$, and $3d$ states calculated with PySCF using exponents from the AHGBSP3-9 basis set.

| System | $E_{\mathrm{tot}}^{1s}$ $[E_{\mathrm{h}}]$ | $E_{\mathrm{tot}}^{2p}$ $[E_{\mathrm{h}}]$ | $E_{\mathrm{tot}}^{3d}$ $[E_{\mathrm{h}}]$ |
|---|---|---|---|
| $H^{0}$ | -0.5015561 | -0.1397375 | -0.0697031 |
| $He^{+}$ | -1.9967832 | -0.5251521 | -0.2470939 |
| $Li^{2+}$ | -4.4916267 | -1.1600637 | -0.5352141 |
| $Be^{3+}$ | -7.9863361 | -2.0447957 | -0.9343043 |
| $B^{4+}$ | -12.4809763 | -3.1794210 | -1.4444206 |
| $C^{5+}$ | -17.9755739 | -4.5639747 | -2.0656085 |
| $N^{6+}$ | -24.4701419 | -6.1985064 | -2.7978906 |
| $O^{7+}$ | -31.9646882 | -8.0830086 | -3.6412308 |
| $F^{8+}$ | -40.4592175 | -10.2174735 | -4.5957739 |
| $Ne^{9+}$ | -49.9537333 | -12.6019372 | -5.6493844 |
| $Na^{10+}$ | -60.4482378 | -15.2363879 | -6.8378136 |
| $Mg^{11+}$ | -71.9427331 | -18.1208299 | -8.1259282 |
| $Al^{12+}$ | -84.4372202 | -21.2552550 | -9.5243817 |
| $Si^{13+}$ | -97.9317003 | -24.6397408 | -11.0343907 |
| $P^{14+}$ | -112.4261745 | -28.2741008 | -12.6553158 |
| $S^{15+}$ | -127.9206432 | -32.1585043 | -14.3880080 |
| $Cl^{16+}$ | -144.4151070 | -36.2929106 | -16.2311060 |
| $Ar^{17+}$ | -161.9095666 | -40.6773128 | -18.1851255 |
| $K^{18+}$ | -180.4040223 | -45.3116662 | -20.2510939 |
| $Ca^{19+}$ | -199.8984743 | -50.1961011 | -22.4273890 |
| $Sc^{20+}$ | -220.3929233 | -55.3305095 | -24.7147963 |
| $Ti^{21+}$ | -241.8873692 | -60.7149888 | -27.1137191 |
| $V^{22+}$ | -264.3818123 | -66.3492763 | -29.6235557 |
| $Cr^{23+}$ | -287.8762530 | -72.2336453 | -32.2451898 |
| $Mn^{24+}$ | -312.3706913 | -78.3680445 | -34.9767805 |
| $Fe^{25+}$ | -337.8651274 | -84.7523927 | -37.8199767 |
| $Co^{26+}$ | -364.3595614 | -91.3868186 | -40.7743689 |
| $Ni^{27+}$ | -391.8539936 | -98.2711830 | -43.8398277 |
| $Cu^{28+}$ | -420.3484240 | -105.4056908 | -47.0162164 |
| $Zn^{29+}$ | -449.8428526 | -112.7900702 | -50.3044450 |
| $Ga^{30+}$ | -480.3372797 | -120.4243077 | -53.7027039 |
| $Ge^{31+}$ | -511.8317053 | -128.3086801 | -57.2127623 |
| $As^{32+}$ | -544.3261294 | -136.4430512 | -60.8337712 |
| $Se^{33+}$ | -577.8205524 | -144.8274212 | -64.5657330 |
| $Br^{34+}$ | -612.3149738 | -153.4617902 | -68.4089250 |
| $Kr^{35+}$ | -647.8093942 | -162.3461761 | -72.3634593 |

Table S11. Total energies for SPW92 for the $1s$, $2p$, and $3d$ states calculated with PySCF using exponents from the AHGBSP3-9 basis set.

| System | $E_{\rm tot}^{1s}$ [$E_{\rm h}$] | $E_{\rm tot}^{2p}$ [$E_{\rm h}$] | $E_{\rm tot}^{3d}$ [$E_{\rm h}$] |
|---|---|---|---|
| $H^{0}$ | -0.4787108 | -0.1321399 | -0.0652987 |
| $He^{+}$ | -1.9417607 | -0.5066465 | -0.2366282 |
| $Li^{2+}$ | -4.4021173 | -1.1293867 | -0.5179229 |
| $Be^{3+}$ | -7.8612408 | -2.0012504 | -0.9096786 |
| $B^{4+}$ | -12.3196462 | -3.1225706 | -1.4121376 |
| $C^{5+}$ | -17.7775784 | -4.4935234 | -2.0254223 |
| $N^{6+}$ | -24.2351742 | -6.1142108 | -2.7496053 |
| $O^{7+}$ | -31.6925180 | -7.9846952 | -3.5847315 |
| $F^{8+}$ | -40.1496657 | -10.1050197 | -4.5308359 |
| $Ne^{9+}$ | -49.6066563 | -12.4752162 | -5.5782629 |
| $Na^{10+}$ | -60.0635182 | -15.0953063 | -6.7560916 |
| $Mg^{11+}$ | -71.5202726 | -17.9653005 | -8.0352913 |
| $Al^{12+}$ | -83.9769359 | -21.0852218 | -9.4254731 |
| $Si^{13+}$ | -97.4335208 | -24.4550570 | -10.9267295 |
| $P^{14+}$ | -111.8900378 | -28.0748626 | -12.5390428 |
| $S^{15+}$ | -127.3464952 | -31.9446096 | -14.2624381 |
| $Cl^{16+}$ | -143.8028999 | -36.0643058 | -16.0969004 |
| $Ar^{17+}$ | -161.2592576 | -40.4339611 | -18.0424506 |
| $K^{18+}$ | -179.7155733 | -45.0536150 | -20.0991221 |
| $Ca^{19+}$ | -199.1718511 | -49.9231553 | -22.2668339 |
| $Sc^{20+}$ | -219.6280945 | -55.0427086 | -24.5455523 |
| $Ti^{21+}$ | -241.0843066 | -60.4122197 | -26.9354480 |
| $V^{22+}$ | -263.5404901 | -66.0317473 | -29.4363807 |
| $Cr^{23+}$ | -286.9966473 | -71.9012201 | -32.0484662 |
| $Mn^{24+}$ | -311.4527803 | -78.0206816 | -34.7716000 |
| $Fe^{25+}$ | -336.9088910 | -84.3901032 | -37.6058060 |
| $Co^{26+}$ | -363.3649809 | -91.0095285 | -40.5511645 |
| $Ni^{27+}$ | -390.8210516 | -97.8789357 | -43.6075895 |
| $Cu^{28+}$ | -419.2771043 | -104.9982855 | -46.7750701 |
| $Zn^{29+}$ | -448.7331402 | -112.3676792 | -50.0537147 |
| $Ga^{30+}$ | -479.1891604 | -119.9870431 | -53.4434191 |
| $Ge^{31+}$ | -510.6451658 | -127.8563843 | -56.9442630 |
| $As^{32+}$ | -543.1011573 | -135.9757128 | -60.5561787 |
| $Se^{33+}$ | -576.5571358 | -144.3450294 | -64.2791598 |
| $Br^{34+}$ | -611.0131019 | -152.9643348 | -68.1132841 |
| $Kr^{35+}$ | -646.4690564 | -161.8336203 | -72.0585298 |

Table S12. Total energies for BHandH for the 1$s$, 2$p$, and 3$d$ states calculated with PySCF using exponents from the AHGBSP3-9 basis set.

| System | $E_{\mathrm{tot}}^{1s}$ [$E_{\mathrm{h}}$] | $E_{\mathrm{tot}}^{2p}$ [$E_{\mathrm{h}}$] | $E_{\mathrm{tot}}^{3d}$ [$E_{\mathrm{h}}$] |
|---|---|---|---|
| $H^{0}$ | -0.4781468 | -0.1219713 | -0.0557732 |
| $He^{+}$ | -1.9559124 | -0.4939208 | -0.2226362 |
| $Li^{2+}$ | -4.4336801 | -1.1158686 | -0.5006170 |
| $Be^{3+}$ | -7.9114484 | -1.9878196 | -0.8897043 |
| $B^{4+}$ | -12.3892169 | -3.1097688 | -1.3899031 |
| $C^{5+}$ | -17.8669854 | -4.4817176 | -2.0012135 |
| $N^{6+}$ | -24.3447540 | -6.1036669 | -2.7236351 |
| $O^{7+}$ | -31.8225226 | -7.9756169 | -3.5571706 |
| $F^{8+}$ | -40.3002913 | -10.0975658 | -4.5018089 |
| $Ne^{9+}$ | -49.7780599 | -12.4695164 | -5.5528822 |
| $Na^{10+}$ | -60.2558286 | -15.0914672 | -6.7244354 |
| $Mg^{11+}$ | -71.7335973 | -17.9634158 | -8.0024285 |
| $Al^{12+}$ | -84.2113660 | -21.0853664 | -9.3915027 |
| $Si^{13+}$ | -97.6891346 | -24.4573080 | -10.8917007 |
| $P^{14+}$ | -112.1669033 | -28.0792633 | -12.5030030 |
| $S^{15+}$ | -127.6446720 | -31.9512152 | -14.2254278 |
| $Cl^{16+}$ | -144.1224407 | -36.0731648 | -16.0589556 |
| $Ar^{17+}$ | -161.6002094 | -40.4451144 | -18.0036056 |
| $K^{18+}$ | -180.0779781 | -45.0670812 | -20.0593875 |
| $Ca^{19+}$ | -199.5557467 | -49.9390092 | -22.2262560 |
| $Sc^{20+}$ | -220.0335154 | -55.0609582 | -24.5042055 |
| $Ti^{21+}$ | -241.5112841 | -60.4329001 | -26.8933058 |
| $V^{22+}$ | -263.9890528 | -66.0548623 | -29.3934929 |
| $Cr^{23+}$ | -287.4668214 | -71.9268095 | -32.0048015 |
| $Mn^{24+}$ | -311.9445901 | -78.0487615 | -34.7272390 |
| $Fe^{25+}$ | -337.4223588 | -84.4207040 | -37.5607582 |
| $Co^{26+}$ | -363.9001275 | -91.0426569 | -40.5054168 |
| $Ni^{27+}$ | -391.3778961 | -97.9146102 | -43.5611723 |
| $Cu^{28+}$ | -419.8556648 | -105.0365431 | -46.7280190 |
| $Zn^{29+}$ | -449.3334335 | -112.4085047 | -50.0060092 |
| $Ga^{30+}$ | -479.8112021 | -120.0304588 | -53.3950942 |
| $Ge^{31+}$ | -511.2889708 | -127.9024084 | -56.8953055 |
| $As^{32+}$ | -543.7667394 | -136.0243579 | -60.5066166 |
| $Se^{33+}$ | -577.2445081 | -144.3963075 | -64.2290218 |
| $Br^{34+}$ | -611.7222767 | -153.0182570 | -68.0625589 |
| $Kr^{35+}$ | -647.2000454 | -161.8902021 | -72.0072165 |

Table S13. Total energies for B3LYP for the $1s$, $2p$, and $3d$ states calculated with PySCF using exponents from the AHGBSP3-9 basis set.

| System | $E_{\rm tot}^{1s}$ [$E_{\rm h}$] | $E_{\rm tot}^{2p}$ [$E_{\rm h}$] | $E_{\rm tot}^{3d}$ [$E_{\rm h}$] |
|---|---|---|---|
| $H^{0}$ | -0.5024433 | -0.1393023 | -0.0698970 |
| $He^{+}$ | -1.9986515 | -0.5245709 | -0.2473975 |
| $Li^{2+}$ | -4.4941883 | -1.1593325 | -0.5356462 |
| $Be^{3+}$ | -7.9894325 | -2.0437943 | -0.9348059 |
| $B^{4+}$ | -12.4845110 | -3.1781526 | -1.4449442 |
| $C^{5+}$ | -17.9794828 | -4.5624219 | -2.0661060 |
| $N^{6+}$ | -24.4743797 | -6.1966196 | -2.7983171 |
| $O^{7+}$ | -31.9692212 | -8.0807540 | -3.6415842 |
| $F^{8+}$ | -40.4640200 | -10.2148585 | -4.5959689 |
| $Ne^{9+}$ | -49.9587850 | -12.5989215 | -5.6522925 |
| $Na^{10+}$ | -60.4535224 | -15.2328413 | -6.8380120 |
| $Mg^{11+}$ | -71.9482369 | -18.1169705 | -8.1256985 |
| $Al^{12+}$ | -84.4429321 | -21.2508476 | -9.5242539 |
| $Si^{13+}$ | -97.9376108 | -24.6350657 | -11.0341215 |
| $P^{14+}$ | -112.4322753 | -28.2689336 | -12.6549944 |
| $S^{15+}$ | -127.9269273 | -32.1527490 | -14.3870885 |
| $Cl^{16+}$ | -144.4215683 | -36.2866936 | -16.2302624 |
| $Ar^{17+}$ | -161.9161996 | -40.6706290 | -18.1843460 |
| $K^{18+}$ | -180.4108221 | -45.3048789 | -20.2498436 |
| $Ca^{19+}$ | -199.9054369 | -50.1887092 | -22.4261876 |
| $Sc^{20+}$ | -220.4000445 | -55.3226387 | -24.7136407 |
| $Ti^{21+}$ | -241.8946457 | -60.7066703 | -27.1116964 |
| $V^{22+}$ | -264.3892411 | -66.3401976 | -29.6219096 |
| $Cr^{23+}$ | -287.8838311 | -72.2243942 | -32.2430983 |
| $Mn^{24+}$ | -312.3784161 | -78.3579856 | -34.9741612 |
| $Fe^{25+}$ | -337.8729966 | -84.7421969 | -37.7942257 |
| $Co^{26+}$ | -364.3675728 | -91.3760183 | -40.7713387 |
| $Ni^{27+}$ | -391.8621452 | -98.2596355 | -43.8365886 |
| $Cu^{28+}$ | -420.3567139 | -105.3940045 | -47.0136722 |
| $Zn^{29+}$ | -449.8512792 | -112.7777129 | -50.3010766 |
| $Ga^{30+}$ | -480.3458413 | -120.4112539 | -53.6997671 |
| $Ge^{31+}$ | -511.8404004 | -128.2951207 | -57.2086683 |
| $As^{32+}$ | -544.3349567 | -136.4289848 | -60.8294591 |
| $Se^{33+}$ | -577.8295104 | -144.8128464 | -64.5621591 |
| $Br^{34+}$ | -612.3240616 | -153.4467055 | -68.4052604 |
| $Kr^{35+}$ | -647.8186104 | -162.3308268 | -72.3584842 |

Table S14. Total energies for PBE for the $1s$, $2p$, and $3d$ states calculated with PySCF using exponents from the AHGBSP3-9 basis set.

| System | $E_{\mathrm{tot}}^{1s}$ [$E_{\mathrm{h}}$] | $E_{\mathrm{tot}}^{2p}$ [$E_{\mathrm{h}}$] | $E_{\mathrm{tot}}^{3d}$ [$E_{\mathrm{h}}$] |
|---|---|---|---|
| $H^{0}$ | -0.4999903 | -0.1398279 | -0.0701565 |
| $He^{+}$ | -1.9937720 | -0.5253068 | -0.2479176 |
| $Li^{2+}$ | -4.4872911 | -1.1602995 | -0.5364792 |
| $Be^{3+}$ | -7.9807506 | -2.0451198 | -0.9359826 |
| $B^{4+}$ | -12.4741911 | -3.1798498 | -1.4465168 |
| $C^{5+}$ | -17.9676247 | -4.5645315 | -2.0681448 |
| $N^{6+}$ | -24.4610557 | -6.1991860 | -2.8007929 |
| $O^{7+}$ | -31.9544860 | -8.0838257 | -3.6445697 |
| $F^{8+}$ | -40.4479164 | -10.2184453 | -4.5994142 |
| $Ne^{9+}$ | -49.9413471 | -12.6030637 | -5.6535858 |
| $Na^{10+}$ | -60.4347783 | -15.2376762 | -6.8424524 |
| $Mg^{11+}$ | -71.9282101 | -18.1222754 | -8.1306914 |
| $Al^{12+}$ | -84.4216425 | -21.2568783 | -9.5299104 |
| $Si^{13+}$ | -97.9150754 | -24.6414452 | -11.0402773 |
| $P^{14+}$ | -112.4085088 | -28.2760597 | -12.6617422 |
| $S^{15+}$ | -127.9019427 | -32.1606598 | -14.3943491 |
| $Cl^{16+}$ | -144.3953770 | -36.2952500 | -16.2380544 |
| $Ar^{17+}$ | -161.8888117 | -40.6798389 | -18.1928904 |
| $K^{18+}$ | -180.3822467 | -45.3144888 | -20.2589028 |
| $Ca^{19+}$ | -199.8756820 | -50.1990025 | -22.4359649 |
| $Sc^{20+}$ | -220.3691177 | -55.3335818 | -24.7239964 |
| $Ti^{21+}$ | -241.8625536 | -60.7181397 | -27.1232956 |
| $V^{22+}$ | -264.3559897 | -66.3527704 | -29.6336154 |
| $Cr^{23+}$ | -287.8494261 | -72.2373460 | -32.2551480 |
| $Mn^{24+}$ | -312.3428627 | -78.3719390 | -34.9877289 |
| $Fe^{25+}$ | -337.8362995 | -84.7564972 | -37.8313824 |
| $Co^{26+}$ | -364.3297365 | -91.3910941 | -40.7862368 |
| $Ni^{27+}$ | -391.8231736 | -98.2756894 | -43.8521566 |
| $Cu^{28+}$ | -420.3166109 | -105.4102122 | -47.0291137 |
| $Zn^{29+}$ | -449.8100483 | -112.7948387 | -50.3173486 |
| $Ga^{30+}$ | -480.3034859 | -120.4294376 | -53.7165395 |
| $Ge^{31+}$ | -511.7969236 | -128.3140200 | -57.2269431 |
| $As^{32+}$ | -544.2903614 | -136.4486023 | -60.8484167 |
| $Se^{33+}$ | -577.7837993 | -144.8331844 | -64.5809373 |
| $Br^{34+}$ | -612.2772373 | -153.4677664 | -68.4246473 |
| $Kr^{35+}$ | -647.7706754 | -162.3523323 | -72.3795027 |

Table S15. Total energies for revPBE for the 1$s$, 2$p$, and 3$d$ states calculated with PySCF using exponents from the AHGBSP3-9 basis set.

| System | $E_{\mathrm{tot}}^{1s}$ [$E_\mathrm{h}$] | $E_{\mathrm{tot}}^{2p}$ [$E_\mathrm{h}$] | $E_{\mathrm{tot}}^{3d}$ [$E_\mathrm{h}$] |
|---|---|---|---|
| $H^{0}$ | -0.5045260 | -0.1427564 | -0.0725627 |
| $He^{+}$ | -2.0028719 | -0.5309782 | -0.2524003 |
| $Li^{2+}$ | -4.5009619 | -1.1687203 | -0.5430601 |
| $Be^{3+}$ | -7.9989942 | -2.0563005 | -0.9446614 |
| $B^{4+}$ | -12.4970081 | -3.1937874 | -1.4572954 |
| $C^{5+}$ | -17.9950155 | -4.5812265 | -2.0810302 |
| $N^{6+}$ | -24.4930204 | -6.2186390 | -2.8157744 |
| $O^{7+}$ | -31.9910249 | -8.1060380 | -3.6616561 |
| $F^{8+}$ | -40.4890294 | -10.2434152 | -4.6185995 |
| $Ne^{9+}$ | -49.9870344 | -12.6307932 | -5.6746117 |
| $Na^{10+}$ | -60.4850399 | -15.2681656 | -6.8658528 |
| $Mg^{11+}$ | -71.9830461 | -18.1555228 | -8.1561888 |
| $Al^{12+}$ | -84.4810528 | -21.2928855 | -9.5575096 |
| $Si^{13+}$ | -97.9790601 | -24.6802044 | -11.0700232 |
| $P^{14+}$ | -112.4770679 | -28.3175828 | -12.6935551 |
| $S^{15+}$ | -127.9750762 | -32.2049439 | -14.4282514 |
| $Cl^{16+}$ | -144.4730849 | -36.3422931 | -16.2740588 |
| $Ar^{17+}$ | -161.9710941 | -40.7296411 | -18.2310019 |
| $K^{18+}$ | -180.4691035 | -45.3670651 | -20.2991329 |
| $Ca^{19+}$ | -199.9671133 | -50.2543143 | -22.4541736 |
| $Sc^{20+}$ | -220.4651234 | -55.3916566 | -24.7684162 |
| $Ti^{21+}$ | -241.9631338 | -60.7789669 | -27.1698282 |
| $V^{22+}$ | -264.4611445 | -66.4163678 | -29.6822413 |
| $Cr^{23+}$ | -287.9591553 | -72.3037004 | -32.3058981 |
| $Mn^{24+}$ | -312.4571664 | -78.4410546 | -35.0405718 |
| $Fe^{25+}$ | -337.9551777 | -84.8283656 | -37.8551528 |
| $Co^{26+}$ | -364.4531891 | -91.4657249 | -40.8432866 |
| $Ni^{27+}$ | -391.9512007 | -98.3530822 | -43.9113099 |
| $Cu^{28+}$ | -420.4492125 | -105.4903494 | -47.0903540 |
| $Zn^{29+}$ | -449.9472244 | -112.8777458 | -50.3806917 |
| $Ga^{30+}$ | -480.4452365 | -120.5151077 | -53.7819934 |
| $Ge^{31+}$ | -511.9432487 | -128.4024492 | -57.2945102 |
| $As^{32+}$ | -544.4412610 | -136.5397906 | -60.9180873 |
| $Se^{33+}$ | -577.9392734 | -144.9271318 | -64.6526966 |
| $Br^{34+}$ | -612.4372859 | -153.5644729 | -68.4985162 |
| $Kr^{35+}$ | -647.9352985 | -162.4517939 | -72.4554837 |

Table S16. Total energies for B97-1 for the 1$s$, 2$p$, and 3$d$ states calculated with PySCF using exponents from the AHGBSP3-9 basis set.

| System | $E^{1s}_{\mathrm{tot}}$ [$E_\mathrm{h}$] | $E^{2p}_{\mathrm{tot}}$ [$E_\mathrm{h}$] | $E^{3d}_{\mathrm{tot}}$ [$E_\mathrm{h}$] |
|---|---|---|---|
| $H^{0}$ | -0.5029265 | -0.1387722 | -0.0686664 |
| $He^{+}$ | -2.0019689 | -0.5251436 | -0.2464845 |
| $Li^{2+}$ | -4.5004195 | -1.1611173 | -0.5352375 |
| $Be^{3+}$ | -7.9986020 | -2.0469078 | -0.9349757 |
| $B^{4+}$ | -12.4966295 | -3.1825717 | -1.4457522 |
| $C^{5+}$ | -17.9945556 | -4.5681539 | -2.0676187 |
| $N^{6+}$ | -24.4924101 | -6.2036798 | -2.8004973 |
| $O^{7+}$ | -31.9902111 | -8.0891659 | -3.6445093 |
| $F^{8+}$ | -40.4879708 | -10.2246091 | -4.5995657 |
| $Ne^{9+}$ | -49.9856974 | -12.6100291 | -5.6562533 |
| $Na^{10+}$ | -60.4833970 | -15.2454344 | -6.8430241 |
| $Mg^{11+}$ | -71.9810742 | -18.1308071 | -8.1314420 |
| $Al^{12+}$ | -84.4787323 | -21.2661716 | -9.5308341 |
| $Si^{13+}$ | -97.9763742 | -24.6514849 | -11.0414513 |
| $P^{14+}$ | -112.4740020 | -28.2868415 | -12.6630629 |
| $S^{15+}$ | -127.9716173 | -32.1721731 | -14.3958318 |
| $Cl^{16+}$ | -144.4692218 | -36.3074856 | -16.2397035 |
| $Ar^{17+}$ | -161.9668166 | -40.6927894 | -18.1947106 |
| $K^{18+}$ | -180.4644027 | -45.3281549 | -20.2608958 |
| $Ca^{19+}$ | -199.9619811 | -50.2133564 | -22.4192159 |
| $Sc^{20+}$ | -220.4595523 | -55.3486362 | -24.7262876 |
| $Ti^{21+}$ | -241.9571171 | -60.7338817 | -27.1257339 |
| $V^{22+}$ | -264.4546760 | -66.3692039 | -29.6362135 |
| $Cr^{23+}$ | -287.9522296 | -72.2544601 | -32.2578914 |
| $Mn^{24+}$ | -312.4497782 | -78.3897315 | -34.9906032 |
| $Fe^{25+}$ | -337.9473222 | -84.7749601 | -37.8099714 |
| $Co^{26+}$ | -364.4448620 | -91.4102286 | -40.7893891 |
| $Ni^{27+}$ | -391.9423978 | -98.2954917 | -43.8554446 |
| $Cu^{28+}$ | -420.4399300 | -105.4306705 | -47.0325457 |
| $Zn^{29+}$ | -449.9374587 | -112.8159627 | -50.3207800 |
| $Ga^{30+}$ | -480.4349843 | -120.4512210 | -53.7202161 |
| $Ge^{31+}$ | -511.9325068 | -128.3364582 | -57.2307544 |
| $As^{32+}$ | -544.4300265 | -136.4716928 | -60.8523544 |
| $Se^{33+}$ | -577.9275435 | -144.8569248 | -64.5850089 |
| $Br^{34+}$ | -612.4250581 | -153.4921545 | -68.4288455 |
| $Kr^{35+}$ | -647.9225703 | -162.3773639 | -72.3838105 |

Table S17. Total energies for HCTH-93 for the $1s$, $2p$, and $3d$ states calculated with PySCF using exponents from the AHGBSP3-9 basis set.

| System | $E_{\text{tot}}^{1s}$ [$E_{\text{h}}$] | $E_{\text{tot}}^{2p}$ [$E_{\text{h}}$] | $E_{\text{tot}}^{3d}$ [$E_{\text{h}}$] |
|---|---|---|---|
| $H^{0}$ | -0.5065443 | -0.1469024 | -0.0769954 |
| $He^{+}$ | -2.0040270 | -0.5384795 | -0.2601251 |
| $Li^{2+}$ | -4.4999600 | -1.1790542 | -0.5537784 |
| $Be^{3+}$ | -7.9951638 | -2.0691389 | -0.9581187 |
| $B^{4+}$ | -12.4899373 | -3.2088910 | -1.4733364 |
| $C^{5+}$ | -17.9844250 | -4.5984248 | -2.0994656 |
| $N^{6+}$ | -24.4787083 | -6.2378017 | -2.8365776 |
| $O^{7+}$ | -31.9728380 | -8.1270642 | -3.6847277 |
| $F^{8+}$ | -40.4668476 | -10.2662142 | -4.6438981 |
| $Ne^{9+}$ | -49.9607608 | -12.6553020 | -5.7027447 |
| $Na^{10+}$ | -60.4545948 | -15.2943257 | -6.8953295 |
| $Mg^{11+}$ | -71.9483627 | -18.1832763 | -8.1877420 |
| $Al^{12+}$ | -84.4420742 | -21.3221962 | -9.5910186 |
| $Si^{13+}$ | -97.9357373 | -24.7110100 | -11.1054465 |
| $P^{14+}$ | -112.4293584 | -28.3498839 | -12.7310470 |
| $S^{15+}$ | -127.9229426 | -32.2387037 | -14.4675685 |
| $Cl^{16+}$ | -144.4164941 | -36.3774782 | -16.3152302 |
| $Ar^{17+}$ | -161.9100164 | -40.7662273 | -18.2740921 |
| $K^{18+}$ | -180.4035126 | -45.4050718 | -20.3442166 |
| $Ca^{19+}$ | -199.8969852 | -50.2936364 | -22.5028289 |
| $Sc^{20+}$ | -220.3904365 | -55.4323088 | -24.8169694 |
| $Ti^{21+}$ | -241.8838683 | -60.8209273 | -27.2202122 |
| $V^{22+}$ | -264.3772822 | -66.4596695 | -29.7343700 |
| $Cr^{23+}$ | -287.8706798 | -72.3482903 | -32.3598734 |
| $Mn^{24+}$ | -312.3640623 | -78.4869347 | -35.0962712 |
| $Fe^{25+}$ | -337.8574308 | -84.8754946 | -37.9152131 |
| $Co^{26+}$ | -364.3507864 | -91.5141251 | -40.9024721 |
| $Ni^{27+}$ | -391.8441300 | -98.4027408 | -43.9722233 |
| $Cu^{28+}$ | -420.3374623 | -105.5412054 | -47.1528819 |
| $Zn^{29+}$ | -449.8307842 | -112.9298651 | -50.4450177 |
| $Ga^{30+}$ | -480.3240962 | -120.5684556 | -53.8479982 |
| $Ge^{31+}$ | -511.8173989 | -128.4570097 | -57.3622487 |
| $As^{32+}$ | -544.3106930 | -136.5955559 | -60.9875127 |
| $Se^{33+}$ | -577.8039790 | -144.9840948 | -64.7242159 |
| $Br^{34+}$ | -612.2972571 | -153.6226265 | -68.5712355 |
| $Kr^{35+}$ | -647.7905280 | -162.5111188 | -72.5299299 |

Table S18. Total energies for RPBE for the 1$s$, 2$p$, and 3$d$ states calculated with PySCF using exponents from the AHGBSP3-9 basis set.

| System | $E^{1s}_{\mathrm{tot}}$ [$E_{\mathrm{h}}$] | $E^{2p}_{\mathrm{tot}}$ [$E_{\mathrm{h}}$] | $E^{3d}_{\mathrm{tot}}$ [$E_{\mathrm{h}}$] |
|---|---|---|---|
| $H^{0}$ | -0.5052823 | -0.1426370 | -0.0722413 |
| $He^{+}$ | -2.0043006 | -0.5307346 | -0.2517953 |
| $Li^{2+}$ | -4.5030637 | -1.1683529 | -0.5421655 |
| $Be^{3+}$ | -8.0017689 | -2.0558045 | -0.9434807 |
| $B^{4+}$ | -12.5004559 | -3.1931636 | -1.4558172 |
| $C^{5+}$ | -17.9991362 | -4.5804779 | -2.0792781 |
| $N^{6+}$ | -24.4978140 | -6.2177616 | -2.8137354 |
| $O^{7+}$ | -31.9964913 | -8.1050312 | -3.6593142 |
| $F^{8+}$ | -40.4951687 | -10.2422830 | -4.6159737 |
| $Ne^{9+}$ | -49.9938465 | -12.6295282 | -5.6715160 |
| $Na^{10+}$ | -60.4925250 | -15.2667738 | -6.8626313 |
| $Mg^{11+}$ | -71.9912039 | -18.1540065 | -8.1527330 |
| $Al^{12+}$ | -84.4898836 | -21.2912377 | -9.5536850 |
| $Si^{13+}$ | -97.9885638 | -24.6784411 | -11.0659617 |
| $P^{14+}$ | -112.4872444 | -28.3156824 | -12.6891973 |
| $S^{15+}$ | -127.9859256 | -32.2029121 | -14.4235525 |
| $Cl^{16+}$ | -144.4846071 | -36.3401332 | -16.2691104 |
| $Ar^{17+}$ | -161.9832891 | -40.7273531 | -18.2257582 |
| $K^{18+}$ | -180.4819714 | -45.3646218 | -20.2935719 |
| $Ca^{19+}$ | -199.9806542 | -50.2517806 | -22.4480492 |
| $Sc^{20+}$ | -220.4793370 | -55.3889925 | -24.7623021 |
| $Ti^{21+}$ | -241.9780203 | -60.7761866 | -27.1634094 |
| $V^{22+}$ | -264.4767038 | -66.4134396 | -29.6755618 |
| $Cr^{23+}$ | -287.9753875 | -72.3006480 | -32.2988717 |
| $Mn^{24+}$ | -312.4740714 | -78.4378703 | -35.0332803 |
| $Fe^{25+}$ | -337.9727555 | -84.8250699 | -37.8471968 |
| $Co^{26+}$ | -364.4714399 | -91.4622899 | -40.8354132 |
| $Ni^{27+}$ | -391.9701242 | -98.3495137 | -43.9031455 |
| $Cu^{28+}$ | -420.4688088 | -105.4866789 | -47.0819442 |
| $Zn^{29+}$ | -449.9674936 | -112.8739208 | -50.3715394 |
| $Ga^{30+}$ | -480.4661786 | -120.5111551 | -53.7729989 |
| $Ge^{31+}$ | -511.9648636 | -128.3983685 | -57.2851821 |
| $As^{32+}$ | -544.4635488 | -136.5355818 | -60.9084682 |
| $Se^{33+}$ | -577.9622338 | -144.9227950 | -64.6427434 |
| $Br^{34+}$ | -612.4609194 | -153.5600080 | -68.4883290 |
| $Kr^{35+}$ | -647.9596048 | -162.4472081 | -72.4449917 |

Table S19. Total energies for BOP for the 1$s$, 2$p$, and 3$d$ states calculated with PySCF using exponents from the AHGBSP3-9 basis set.

| System | $E_{\rm tot}^{1s}$ [$E_{\rm h}$] | $E_{\rm tot}^{2p}$ [$E_{\rm h}$] | $E_{\rm tot}^{3d}$ [$E_{\rm h}$] |
|---|---|---|---|
| $H^{0}$ | -0.4979152 | -0.1382605 | -0.0699043 |
| $He^{+}$ | -1.9951322 | -0.5261207 | -0.2498943 |
| $Li^{2+}$ | -4.4923763 | -1.1640621 | -0.5409459 |
| $Be^{3+}$ | -7.9896263 | -2.0519266 | -0.9431702 |
| $B^{4+}$ | -12.4868788 | -3.1897955 | -1.4564921 |
| $C^{5+}$ | -17.9841323 | -4.5776965 | -2.0809295 |
| $N^{6+}$ | -24.4813862 | -6.2155902 | -2.8164467 |
| $O^{7+}$ | -31.9786406 | -8.1034652 | -3.6631138 |
| $F^{8+}$ | -40.4758953 | -10.2413525 | -4.6209090 |
| $Ne^{9+}$ | -49.9731500 | -12.6292250 | -5.6781899 |
| $Na^{10+}$ | -60.4704049 | -15.2669326 | -6.8697055 |
| $Mg^{11+}$ | -71.9676598 | -18.1550064 | -8.1610063 |
| $Al^{12+}$ | -84.4649151 | -21.2926653 | -9.5630510 |
| $Si^{13+}$ | -97.9621701 | -24.6808664 | -11.0765447 |
| $P^{14+}$ | -112.4594252 | -28.3185952 | -12.7007486 |
| $S^{15+}$ | -127.9566805 | -32.2062686 | -14.4363269 |
| $Cl^{16+}$ | -144.4539357 | -36.3441364 | -16.2831368 |
| $Ar^{17+}$ | -161.9511909 | -40.7320041 | -18.2406496 |
| $K^{18+}$ | -180.4484462 | -45.3703230 | -20.3098795 |
| $Ca^{19+}$ | -199.9457015 | -50.2580647 | -22.4897014 |
| $Sc^{20+}$ | -220.4429569 | -55.3959553 | -24.7806890 |
| $Ti^{21+}$ | -241.9402121 | -60.7839979 | -27.1820837 |
| $V^{22+}$ | -264.4374676 | -66.4213425 | -29.6960620 |
| $Cr^{23+}$ | -287.9347228 | -72.3096296 | -32.3208457 |
| $Mn^{24+}$ | -312.4319783 | -78.4470780 | -35.0552607 |
| $Fe^{25+}$ | -337.9292336 | -84.8353977 | -37.9029402 |
| $Co^{26+}$ | -364.4264889 | -91.4731789 | -40.8596010 |
| $Ni^{27+}$ | -391.9237445 | -98.3606811 | -43.9284378 |
| $Cu^{28+}$ | -420.4209997 | -105.4992379 | -47.1093725 |
| $Zn^{29+}$ | -449.9182552 | -112.8871290 | -50.4003893 |
| $Ga^{30+}$ | -480.4155106 | -120.5242842 | -53.8031815 |
| $Ge^{31+}$ | -511.9127660 | -128.4121518 | -57.3148962 |
| $As^{32+}$ | -544.4100214 | -136.5500195 | -60.9392886 |
| $Se^{33+}$ | -577.9072768 | -144.9378872 | -64.6759125 |
| $Br^{34+}$ | -612.4045321 | -153.5757548 | -68.5226555 |
| $Kr^{35+}$ | -647.9017875 | -162.4639910 | -72.4791324 |

Table S20. Total energies for PKZB for the $1s$, $2p$, and $3d$ states calculated with PySCF using exponents from the AHGBSP3-9 basis set.

| System | $E^{1s}_{\mathrm{tot}}$ [$E_\mathrm{h}$] | $E^{2p}_{\mathrm{tot}}$ [$E_\mathrm{h}$] | $E^{3d}_{\mathrm{tot}}$ [$E_\mathrm{h}$] |
|---|---|---|---|
| $H^{0}$ | -0.4964487 | -0.1361827 | -0.0679631 |
| $He^{+}$ | -1.9920369 | -0.5226206 | -0.2460617 |
| $Li^{2+}$ | -4.4876616 | -1.1587454 | -0.5353288 |
| $Be^{3+}$ | -7.9832942 | -2.0448734 | -0.9356890 |
| $B^{4+}$ | -12.4789298 | -3.1809997 | -1.4471663 |
| $C^{5+}$ | -17.9745669 | -4.5671255 | -2.0698003 |
| $N^{6+}$ | -24.4702048 | -6.2032533 | -2.8034651 |
| $O^{7+}$ | -31.9658432 | -8.0893852 | -3.6482775 |
| $F^{8+}$ | -40.4614819 | -10.2255097 | -4.6041938 |
| $Ne^{9+}$ | -49.9571209 | -12.6116390 | -5.6713276 |
| $Na^{10+}$ | -60.4527601 | -15.2477759 | -6.8494059 |
| $Mg^{11+}$ | -71.9483993 | -18.1339010 | -8.1387542 |
| $Al^{12+}$ | -84.4440386 | -21.2700338 | -9.5390491 |
| $Si^{13+}$ | -97.9396781 | -24.6561347 | -11.0505166 |
| $P^{14+}$ | -112.4353176 | -28.2922826 | -12.6731007 |
| $S^{15+}$ | -127.9309571 | -32.1784209 | -14.4067849 |
| $Cl^{16+}$ | -144.4265967 | -36.3142200 | -16.2516000 |
| $Ar^{17+}$ | -161.9222363 | -40.7006789 | -18.2075519 |
| $K^{18+}$ | -180.4178759 | -45.3368673 | -20.2747113 |
| $Ca^{19+}$ | -199.9135156 | -50.2229211 | -22.4527343 |
| $Sc^{20+}$ | -220.4091553 | -55.3590478 | -24.7420076 |
| $Ti^{21+}$ | -241.9047949 | -60.7451509 | -27.1424328 |
| $V^{22+}$ | -264.4004347 | -66.3813240 | -29.6538686 |
| $Cr^{23+}$ | -287.8960743 | -72.2674440 | -32.2765413 |
| $Mn^{24+}$ | -312.3917141 | -78.4035821 | -35.0102238 |
| $Fe^{25+}$ | -337.8873538 | -84.7896851 | -37.8552424 |
| $Co^{26+}$ | -364.3829935 | -91.4258281 | -40.8109734 |
| $Ni^{27+}$ | -391.8786332 | -98.3119692 | -43.8780149 |
| $Cu^{28+}$ | -420.3742729 | -105.4480401 | -47.0560942 |
| $Zn^{29+}$ | -449.8699127 | -112.8342121 | -50.3454213 |
| $Ga^{30+}$ | -480.3655525 | -120.4703563 | -53.7457526 |
| $Ge^{31+}$ | -511.8611922 | -128.3564853 | -57.2572919 |
| $As^{32+}$ | -544.3568320 | -136.4926143 | -60.8798889 |
| $Se^{33+}$ | -577.8524716 | -144.8787433 | -64.6135265 |
| $Br^{34+}$ | -612.3481115 | -153.5148723 | -68.4583617 |
| $Kr^{35+}$ | -647.8437513 | -162.4009852 | -72.4143467 |

Table S21. Total energies for HSE03 for the 1$s$, 2$p$, and 3$d$ states calculated with PySCF using exponents from the AHGBSP3-9 basis set.

| System | $E^{1s}_{\rm tot}$ [$E_{\rm h}$] | $E^{2p}_{\rm tot}$ [$E_{\rm h}$] | $E^{3d}_{\rm tot}$ [$E_{\rm h}$] |
|---|---|---|---|
| $H^{0}$ | -0.5114319 | -0.1434797 | -0.0713572 |
| $He^{+}$ | -2.0085000 | -0.5295611 | -0.2494451 |
| $Li^{2+}$ | -4.5043121 | -1.1633603 | -0.5370854 |
| $Be^{3+}$ | -7.9998680 | -2.0463826 | -0.9349691 |
| $B^{4+}$ | -12.4953440 | -3.1790690 | -1.4435133 |
| $C^{5+}$ | -17.9907855 | -4.5615927 | -2.0629246 |
| $N^{6+}$ | -24.4862145 | -6.1940222 | -2.7932914 |
| $O^{7+}$ | -31.9816333 | -8.0764016 | -3.6346799 |
| $F^{8+}$ | -40.4770498 | -10.2087435 | -4.5871598 |
| $Ne^{9+}$ | -49.9724619 | -12.5910623 | -5.6417174 |
| $Na^{10+}$ | -60.4678770 | -15.2233714 | -6.8251995 |
| $Mg^{11+}$ | -71.9632825 | -18.1056552 | -8.1109488 |
| $Al^{12+}$ | -84.4587013 | -21.2379426 | -9.5076501 |
| $Si^{13+}$ | -97.9541107 | -24.6201946 | -11.0155372 |
| $P^{14+}$ | -112.4495180 | -28.2524770 | -12.6344425 |
| $S^{15+}$ | -127.9449344 | -32.1347510 | -14.3645091 |
| $Cl^{16+}$ | -144.4403383 | -36.2670124 | -16.2056724 |
| $Ar^{17+}$ | -161.9357529 | -40.6492717 | -18.1579673 |
| $K^{18+}$ | -180.4311669 | -45.2815542 | -20.2214989 |
| $Ca^{19+}$ | -199.9265803 | -50.1637711 | -22.3959942 |
| $Sc^{20+}$ | -220.4219929 | -55.2960145 | -24.6814364 |
| $Ti^{21+}$ | -241.9174046 | -60.6782535 | -27.0781495 |
| $V^{22+}$ | -264.4128155 | -66.3105396 | -29.5859433 |
| $Cr^{23+}$ | -287.9082253 | -72.1927763 | -32.2049586 |
| $Mn^{24+}$ | -312.4036340 | -78.3250391 | -34.9349203 |
| $Fe^{25+}$ | -337.8990627 | -84.7072717 | -37.7760410 |
| $Co^{26+}$ | -364.3944703 | -91.3395177 | -40.7283150 |
| $Ni^{27+}$ | -391.8898764 | -98.2217831 | -43.7916770 |
| $Cu^{28+}$ | -420.3853056 | -105.3539842 | -46.9661170 |
| $Zn^{29+}$ | -449.8807103 | -112.7362552 | -50.2517826 |
| $Ga^{30+}$ | -480.3761134 | -120.3685234 | -53.6484302 |
| $Ge^{31+}$ | -511.8715428 | -128.2507699 | -57.1562283 |
| $As^{32+}$ | -544.3669441 | -136.3830153 | -60.7751423 |
| $Se^{33+}$ | -577.8623737 | -144.7652598 | -64.5051983 |
| $Br^{34+}$ | -612.3577730 | -153.3975069 | -68.3462827 |
| $Kr^{35+}$ | -647.8532029 | -162.2797326 | -72.2985468 |

Table S22. Total energies for TPSS for the $1s$, $2p$, and $3d$ states calculated with PySCF using exponents from the AHGBSP3-9 basis set.

| System | $E_{\mathrm{tot}}^{1s}$ [$E_\mathrm{h}$] | $E_{\mathrm{tot}}^{2p}$ [$E_\mathrm{h}$] | $E_{\mathrm{tot}}^{3d}$ [$E_\mathrm{h}$] |
|---|---|---|---|
| $H^{0}$ | -0.5002353 | -0.1370240 | -0.0672643 |
| $He^{+}$ | -2.0002197 | -0.5236688 | -0.2447033 |
| $Li^{2+}$ | -4.5002152 | -1.1603118 | -0.5333050 |
| $Be^{3+}$ | -8.0002130 | -2.0469672 | -0.9330047 |
| $B^{4+}$ | -12.5002118 | -3.1836160 | -1.4438194 |
| $C^{5+}$ | -18.0002111 | -4.5702644 | -2.0657821 |
| $N^{6+}$ | -24.5002105 | -6.2069145 | -2.7987910 |
| $O^{7+}$ | -32.0002101 | -8.0935647 | -3.6429439 |
| $F^{8+}$ | -40.5002098 | -10.2302157 | -4.5981991 |
| $Ne^{9+}$ | -50.0002095 | -12.6168707 | -5.6533367 |
| $Na^{10+}$ | -60.5002094 | -15.2535266 | -6.8420809 |
| $Mg^{11+}$ | -72.0002092 | -18.1401741 | -8.1307444 |
| $Al^{12+}$ | -84.5002091 | -21.2768293 | -9.5303956 |
| $Si^{13+}$ | -98.0002091 | -24.6634516 | -11.0412450 |
| $P^{14+}$ | -112.5002089 | -28.3001228 | -12.6631806 |
| $S^{15+}$ | -128.0002089 | -32.1867834 | -14.3961556 |
| $Cl^{16+}$ | -144.5002088 | -36.3234343 | -16.2403080 |
| $Ar^{17+}$ | -162.0002088 | -40.7100862 | -18.1955950 |
| $K^{18+}$ | -180.5002087 | -45.3467995 | -20.2620685 |
| $Ca^{19+}$ | -200.0002087 | -50.2333732 | -22.4171851 |
| $Sc^{20+}$ | -220.5002087 | -55.3700222 | -24.7280587 |
| $Ti^{21+}$ | -242.0002086 | -60.7566461 | -27.1278141 |
| $V^{22+}$ | -264.5002086 | -66.3933431 | -29.6385870 |
| $Cr^{23+}$ | -288.0002086 | -72.2799856 | -32.2605893 |
| $Mn^{24+}$ | -312.5002086 | -78.4166459 | -34.9936166 |
| $Fe^{25+}$ | -338.0002085 | -84.8032717 | -37.8088042 |
| $Co^{26+}$ | -364.5002085 | -91.4399366 | -40.7930405 |
| $Ni^{27+}$ | -392.0002084 | -98.3266000 | -43.8594192 |
| $Cu^{28+}$ | -420.5002084 | -105.4631914 | -47.0368346 |
| $Zn^{29+}$ | -450.0002084 | -112.8498865 | -50.3255312 |
| $Ga^{30+}$ | -480.5002084 | -120.4865542 | -53.7251748 |
| $Ge^{31+}$ | -512.0002083 | -128.3732056 | -57.2360449 |
| $As^{32+}$ | -544.5002083 | -136.5098569 | -60.8579791 |
| $Se^{33+}$ | -578.0002082 | -144.8965083 | -64.5909603 |
| $Br^{34+}$ | -612.5002083 | -153.5331597 | -68.4351106 |
| $Kr^{35+}$ | -648.0002082 | -162.4197950 | -72.3904484 |

Table S23. Total energies for TPSSh for the $1s$, $2p$, and $3d$ states calculated with PySCF using exponents from the AHGBSP3-9 basis set.

| System | $E_{\text{tot}}^{1s}$ [$E_\text{h}$] | $E_{\text{tot}}^{2p}$ [$E_\text{h}$] | $E_{\text{tot}}^{3d}$ [$E_\text{h}$] |
|---|---|---|---|
| $H^{0}$ | -0.5001879 | -0.1357870 | -0.0660076 |
| $He^{+}$ | -2.0001768 | -0.5212684 | -0.2423762 |
| $Li^{2+}$ | -4.5001736 | -1.1567475 | -0.5298973 |
| $Be^{3+}$ | -8.0001721 | -2.0422376 | -0.9285170 |
| $B^{4+}$ | -12.5001712 | -3.1777214 | -1.4382509 |
| $C^{5+}$ | -18.0001706 | -4.5632052 | -2.0591288 |
| $N^{6+}$ | -24.5001702 | -6.1986904 | -2.7910594 |
| $O^{7+}$ | -32.0001700 | -8.0841757 | -3.6341386 |
| $F^{8+}$ | -40.5001697 | -10.2196616 | -4.5883044 |
| $Ne^{9+}$ | -50.0001696 | -12.6051480 | -5.6434960 |
| $Na^{10+}$ | -60.5001695 | -15.2406414 | -6.8300075 |
| $Mg^{11+}$ | -72.0001693 | -18.1261242 | -8.1175962 |
| $Al^{12+}$ | -84.5001693 | -21.2616138 | -9.5161710 |
| $Si^{13+}$ | -98.0001692 | -24.6470739 | -11.0259353 |
| $P^{14+}$ | -112.5001692 | -28.2825784 | -12.6467187 |
| $S^{15+}$ | -128.0001691 | -32.1680725 | -14.3786885 |
| $Cl^{16+}$ | -144.5001691 | -36.3035584 | -16.2217602 |
| $Ar^{17+}$ | -162.0001691 | -40.6890450 | -18.1759618 |
| $K^{18+}$ | -180.5001690 | -45.3245870 | -20.2413435 |
| $Ca^{19+}$ | -200.0001690 | -50.2100034 | -22.3976267 |
| $Sc^{20+}$ | -220.5001690 | -55.3454875 | -24.7051792 |
| $Ti^{21+}$ | -242.0001689 | -60.7309490 | -27.1038479 |
| $V^{22+}$ | -264.5001689 | -66.3664763 | -29.6135436 |
| $Cr^{23+}$ | -288.0001689 | -72.2519546 | -32.2344557 |
| $Mn^{24+}$ | -312.5001689 | -78.3874488 | -34.9664036 |
| $Fe^{25+}$ | -338.0001688 | -84.7729120 | -37.7834182 |
| $Co^{26+}$ | -364.5001688 | -91.4084078 | -40.7636629 |
| $Ni^{27+}$ | -392.0001688 | -98.2939075 | -43.8289593 |
| $Cu^{28+}$ | -420.5001687 | -105.4293397 | -47.0053025 |
| $Zn^{29+}$ | -450.0001687 | -112.8148653 | -50.2929045 |
| $Ga^{30+}$ | -480.5001687 | -120.4503662 | -53.6914727 |
| $Ge^{31+}$ | -512.0001686 | -128.3358525 | -57.2012558 |
| $As^{32+}$ | -544.5001686 | -136.4713387 | -60.8221077 |
| $Se^{33+}$ | -578.0001685 | -144.8568249 | -64.5540129 |
| $Br^{34+}$ | -612.5001686 | -153.4923112 | -68.3970978 |
| $Kr^{35+}$ | -648.0001685 | -162.3777829 | -72.3513301 |

Table S24. Total energies for CAM-B3LYP for the $1s$, $2p$, and $3d$ states calculated with PySCF using exponents from the AHGBSP3-9 basis set.

| System | $E_{\text{tot}}^{1s}$ [$E_{\text{h}}$] | $E_{\text{tot}}^{2p}$ [$E_{\text{h}}$] | $E_{\text{tot}}^{3d}$ [$E_{\text{h}}$] |
|---|---|---|---|
| $H^{0}$ | -0.4990948 | -0.1328067 | -0.0622342 |
| $He^{+}$ | -1.9899259 | -0.5159359 | -0.2358566 |
| $Li^{2+}$ | -4.4830296 | -1.1485579 | -0.5218518 |
| $Be^{3+}$ | -7.9778463 | -2.0309394 | -0.9194301 |
| $B^{4+}$ | -12.4736404 | -3.1635587 | -1.4281794 |
| $C^{5+}$ | -17.9700186 | -4.5465342 | -2.0479957 |
| $N^{6+}$ | -24.4667682 | -6.1798571 | -2.7789399 |
| $O^{7+}$ | -31.9637668 | -8.0634796 | -3.6210775 |
| $F^{8+}$ | -40.4609395 | -10.1973624 | -4.5744158 |
| $Ne^{9+}$ | -49.9582385 | -12.5814520 | -5.6300873 |
| $Na^{10+}$ | -60.4556314 | -15.2156594 | -6.8148177 |
| $Mg^{11+}$ | -71.9530961 | -18.1001242 | -8.1019108 |
| $Al^{12+}$ | -84.4506166 | -21.2345965 | -9.5001380 |
| $Si^{13+}$ | -97.9481813 | -24.6193148 | -11.0096540 |
| $P^{14+}$ | -112.4457814 | -28.2540101 | -12.6303483 |
| $S^{15+}$ | -127.9434103 | -32.1387389 | -14.3622596 |
| $Cl^{16+}$ | -144.4410630 | -36.2735946 | -16.2053607 |
| $Ar^{17+}$ | -161.9387354 | -40.6585053 | -18.1596314 |
| $K^{18+}$ | -180.4364242 | -45.2935599 | -20.2250945 |
| $Ca^{19+}$ | -199.9341270 | -50.1785572 | -22.4016919 |
| $Sc^{20+}$ | -220.4318415 | -55.3135950 | -24.6895151 |
| $Ti^{21+}$ | -241.9295662 | -60.6986743 | -27.0882163 |
| $V^{22+}$ | -264.4272995 | -66.3336694 | -29.5985290 |
| $Cr^{23+}$ | -287.9250403 | -72.2188808 | -32.2198444 |
| $Mn^{24+}$ | -312.4227877 | -78.3539410 | -34.9519811 |
| $Fe^{25+}$ | -337.9205407 | -84.7392109 | -37.7957668 |
| $Co^{26+}$ | -364.4182987 | -91.3743921 | -40.7502264 |
| $Ni^{27+}$ | -391.9160610 | -98.2594990 | -43.8160610 |
| $Cu^{28+}$ | -420.4138272 | -105.3948430 | -46.9932853 |
| $Zn^{29+}$ | -449.9115968 | -112.7800795 | -50.2812955 |
| $Ga^{30+}$ | -480.4093693 | -120.4151955 | -53.6806361 |
| $Ge^{31+}$ | -511.9071445 | -128.3004523 | -57.1907610 |
| $As^{32+}$ | -544.4049221 | -136.4357198 | -60.8122673 |
| $Se^{33+}$ | -577.9027018 | -144.8209969 | -64.5451685 |
| $Br^{34+}$ | -612.4004833 | -153.4562830 | -68.3889666 |
| $Kr^{35+}$ | -647.8982665 | -162.3416475 | -72.3435580 |

Table S25. Total energies for XLYP for the $1s$, $2p$, and $3d$ states calculated with PySCF using exponents from the AHGBSP3-9 basis set.

| System | $E_{\mathrm{tot}}^{1s}$ [$E_{\mathrm{h}}$] | $E_{\mathrm{tot}}^{2p}$ [$E_{\mathrm{h}}$] | $E_{\mathrm{tot}}^{3d}$ [$E_{\mathrm{h}}$] |
|---|---|---|---|
| $H^{0}$ | -0.4998682 | -0.1383660 | -0.0695971 |
| $He^{+}$ | -1.9989582 | -0.5263231 | -0.2492802 |
| $Li^{2+}$ | -4.4980783 | -1.1643090 | -0.5400121 |
| $Be^{3+}$ | -7.9972051 | -2.0522349 | -0.9419638 |
| $B^{4+}$ | -12.4963344 | -3.1902013 | -1.4549346 |
| $C^{5+}$ | -17.9954650 | -4.5781703 | -2.0790222 |
| $N^{6+}$ | -24.4945963 | -6.2161399 | -2.8142953 |
| $O^{7+}$ | -31.9937280 | -8.1040936 | -3.6606305 |
| $F^{8+}$ | -40.4928600 | -10.2420534 | -4.6181347 |
| $Ne^{9+}$ | -49.9919923 | -12.6300062 | -5.6748214 |
| $Na^{10+}$ | -60.4911246 | -15.2678396 | -6.8663084 |
| $Mg^{11+}$ | -71.9902571 | -18.1559308 | -8.1573878 |
| $Al^{12+}$ | -84.4893896 | -21.2937339 | -9.5589748 |
| $Si^{13+}$ | -97.9885222 | -24.6819355 | -11.0720641 |
| $P^{14+}$ | -112.4876549 | -28.3197716 | -12.6961153 |
| $S^{15+}$ | -127.9867876 | -32.2075785 | -14.4315019 |
| $Cl^{16+}$ | -144.4859203 | -36.3455268 | -16.2779139 |
| $Ar^{17+}$ | -161.9850531 | -40.7334750 | -18.2351479 |
| $K^{18+}$ | -180.4841859 | -45.3717662 | -20.3041032 |
| $Ca^{19+}$ | -199.9833187 | -50.2596049 | -22.4834831 |
| $Sc^{20+}$ | -220.4824515 | -55.3975738 | -24.7741845 |
| $Ti^{21+}$ | -241.9815843 | -60.7856655 | -27.1755325 |
| $V^{22+}$ | -264.4807171 | -66.4232161 | -29.6889888 |
| $Cr^{23+}$ | -287.9798500 | -72.3114622 | -32.3132564 |
| $Mn^{24+}$ | -312.4789828 | -78.4491125 | -35.0478182 |
| $Fe^{25+}$ | -337.9781157 | -84.8373767 | -37.8949184 |
| $Co^{26+}$ | -364.4772486 | -91.4752770 | -40.8515643 |
| $Ni^{27+}$ | -391.9763814 | -98.3629572 | -43.9201040 |
| $Cu^{28+}$ | -420.4755143 | -105.5014292 | -47.1004338 |
| $Zn^{29+}$ | -449.9746472 | -112.8893953 | -50.3903366 |
| $Ga^{30+}$ | -480.4737801 | -120.5268018 | -53.7931025 |
| $Ge^{31+}$ | -511.9729129 | -128.4147501 | -57.3053739 |
| $As^{32+}$ | -544.4720458 | -136.5526983 | -60.9294692 |
| $Se^{33+}$ | -577.9711787 | -144.9406465 | -64.6654354 |
| $Br^{34+}$ | -612.4703116 | -153.5785947 | -68.5118481 |
| $Kr^{35+}$ | -647.9694444 | -162.4668132 | -72.4684217 |

Table S26. Total energies for HSE06 for the 1$s$, 2$p$, and 3$d$ states calculated with PySCF using exponents from the AHGBSP3-9 basis set.

| System | $E_{\text{tot}}^{1s}$ [$E_\text{h}$] | $E_{\text{tot}}^{2p}$ [$E_\text{h}$] | $E_{\text{tot}}^{3d}$ [$E_\text{h}$] |
|---|---|---|---|
| $H^{0}$ | -0.5015080 | -0.1375469 | -0.0685364 |
| $He^{+}$ | -1.9973664 | -0.5204822 | -0.2430832 |
| $Li^{2+}$ | -4.4928868 | -1.1531214 | -0.5287490 |
| $Be^{3+}$ | -7.9883307 | -2.0356118 | -0.9255540 |
| $B^{4+}$ | -12.4837522 | -3.1680130 | -1.4334658 |
| $C^{5+}$ | -17.9791632 | -4.5503663 | -2.0524689 |
| $N^{6+}$ | -24.4745734 | -6.1826858 | -2.7825637 |
| $O^{7+}$ | -31.9699797 | -8.0649899 | -3.6237627 |
| $F^{8+}$ | -40.4653877 | -10.1972781 | -4.5761023 |
| $Ne^{9+}$ | -49.9607936 | -12.5795572 | -5.6305958 |
| $Na^{10+}$ | -60.4562040 | -15.2118360 | -6.8139581 |
| $Mg^{11+}$ | -71.9516060 | -18.0940962 | -8.0996433 |
| $Al^{12+}$ | -84.4470220 | -21.2263650 | -9.4962940 |
| $Si^{13+}$ | -97.9424292 | -24.6086021 | -11.0041407 |
| $P^{14+}$ | -112.4378347 | -28.2408721 | -12.6230112 |
| $S^{15+}$ | -127.9332496 | -32.1231358 | -14.3530489 |
| $Cl^{16+}$ | -144.4286523 | -36.2553886 | -16.1941749 |
| $Ar^{17+}$ | -161.9240659 | -40.6376406 | -18.1464618 |
| $K^{18+}$ | -180.4194790 | -45.2699168 | -20.2099757 |
| $Ca^{19+}$ | -199.9148916 | -50.1521285 | -22.3844557 |
| $Sc^{20+}$ | -220.4103036 | -55.2843672 | -24.6698848 |
| $Ti^{21+}$ | -241.9057148 | -60.6666022 | -27.0665860 |
| $V^{22+}$ | -264.4011251 | -66.2988847 | -29.5743697 |
| $Cr^{23+}$ | -287.8965345 | -72.1811182 | -32.1933758 |
| $Mn^{24+}$ | -312.3919429 | -78.3133782 | -34.9233291 |
| $Fe^{25+}$ | -337.8873713 | -84.6956083 | -37.7644429 |
| $Co^{26+}$ | -364.3827785 | -91.3278521 | -40.7167101 |
| $Ni^{27+}$ | -391.8781844 | -98.2101154 | -43.7800662 |
| $Cu^{28+}$ | -420.3736133 | -105.3423148 | -46.9544997 |
| $Zn^{29+}$ | -449.8690178 | -112.7245837 | -50.2401733 |
| $Ga^{30+}$ | -480.3644207 | -120.3568508 | -53.6368051 |
| $Ge^{31+}$ | -511.8598500 | -128.2390959 | -57.1445988 |
| $As^{32+}$ | -544.3552511 | -136.3713400 | -60.7635091 |
| $Se^{33+}$ | -577.8506806 | -144.7535834 | -64.4935621 |
| $Br^{34+}$ | -612.3460797 | -153.3858295 | -68.3346430 |
| $Kr^{35+}$ | -647.8415094 | -162.2680543 | -72.2869043 |

Table S27. Total energies for M06-L for the 1$s$, 2$p$, and 3$d$ states calculated with PySCF using exponents from the AHGBSP3-9 basis set.

| System | $E^{1s}_{\mathrm{tot}}$ [$E_\mathrm{h}$] | $E^{2p}_{\mathrm{tot}}$ [$E_\mathrm{h}$] | $E^{3d}_{\mathrm{tot}}$ [$E_\mathrm{h}$] |
|---|---|---|---|
| $H^{0}$ | -0.5046959 | -0.1420240 | -0.0728534 |
| $He^{+}$ | -2.0082099 | -0.5330235 | -0.2547781 |
| $Li^{2+}$ | -4.5117345 | -1.1740675 | -0.5481649 |
| $Be^{3+}$ | -8.0152695 | -2.0649959 | -0.9520977 |
| $B^{4+}$ | -12.5188132 | -3.2059711 | -1.4674653 |
| $C^{5+}$ | -18.0223610 | -4.5969452 | -2.0939874 |
| $N^{6+}$ | -24.5259029 | -6.2379468 | -2.8315508 |
| $O^{7+}$ | -32.0294541 | -8.1289233 | -3.6811950 |
| $F^{8+}$ | -40.5329976 | -10.2698904 | -4.6396049 |
| $Ne^{9+}$ | -50.0365480 | -12.6608918 | -5.7119265 |
| $Na^{10+}$ | -60.5401002 | -15.3018977 | -6.8944977 |
| $Mg^{11+}$ | -72.0436459 | -18.1928701 | -8.1867892 |
| $Al^{12+}$ | -84.5471973 | -21.3338695 | -9.5904083 |
| $Si^{13+}$ | -98.0507521 | -24.7247075 | -11.1067146 |
| $P^{14+}$ | -112.5543003 | -28.3658043 | -12.7341121 |
| $S^{15+}$ | -128.0578513 | -32.2568278 | -14.4715018 |
| $Cl^{16+}$ | -144.5614015 | -36.3978111 | -16.3202854 |
| $Ar^{17+}$ | -162.0649546 | -40.7888003 | -18.2802923 |
| $K^{18+}$ | -180.5685047 | -45.4301111 | -20.3507713 |
| $Ca^{19+}$ | -200.0720597 | -50.3207230 | -22.5334899 |
| $Sc^{20+}$ | -220.5756068 | -55.4616791 | -24.8272033 |
| $Ti^{21+}$ | -242.0791588 | -60.8525135 | -27.2318602 |
| $V^{22+}$ | -264.5827116 | -66.4937316 | -29.7464681 |
| $Cr^{23+}$ | -288.0862611 | -72.3846810 | -32.3732341 |
| $Mn^{24+}$ | -312.5898132 | -78.5257045 | -35.1117485 |
| $Fe^{25+}$ | -338.0933622 | -84.9165823 | -37.9597286 |
| $Co^{26+}$ | -364.5969165 | -91.5576233 | -40.9205631 |
| $Ni^{27+}$ | -392.1004639 | -98.4486637 | -43.9916371 |
| $Cu^{28+}$ | -420.6040137 | -105.5893444 | -47.1728430 |
| $Zn^{29+}$ | -450.1075664 | -112.9805383 | -50.4657863 |
| $Ga^{30+}$ | -480.6111200 | -120.6216228 | -53.8704889 |
| $Ge^{31+}$ | -512.1146705 | -128.5126091 | -57.3870444 |
| $As^{32+}$ | -544.6182253 | -136.6535956 | -61.0136740 |
| $Se^{33+}$ | -578.1217682 | -145.0445819 | -64.7506462 |
| $Br^{34+}$ | -612.6253287 | -153.6855684 | -68.5998918 |
| $Kr^{35+}$ | -648.1288803 | -162.5764831 | -72.5602296 |

Table S28. Total energies for PBEsol for the $1s$, $2p$, and $3d$ states calculated with PySCF using exponents from the AHGBSP3-9 basis set.

| System | $E_{\mathrm{tot}}^{1s}$ $[E_{\mathrm{h}}]$ | $E_{\mathrm{tot}}^{2p}$ $[E_{\mathrm{h}}]$ | $E_{\mathrm{tot}}^{3d}$ $[E_{\mathrm{h}}]$ |
|---|---|---|---|
| $H^{0}$ | -0.4887153 | -0.1359361 | -0.0678028 |
| $He^{+}$ | -1.9695717 | -0.5169910 | -0.2430880 |
| $Li^{2+}$ | -4.4499692 | -1.1473820 | -0.5290541 |
| $Be^{3+}$ | -7.9302463 | -2.0275294 | -0.9259040 |
| $B^{4+}$ | -12.4104782 | -3.1575433 | -1.4337510 |
| $C^{5+}$ | -17.8906897 | -4.5374843 | -2.0526687 |
| $N^{6+}$ | -24.3708909 | -6.1673820 | -2.7825939 |
| $O^{7+}$ | -31.8510867 | -8.0472537 | -3.6236366 |
| $F^{8+}$ | -40.3312793 | -10.1770972 | -4.5757413 |
| $Ne^{9+}$ | -49.8114702 | -12.5569334 | -5.6280781 |
| $Na^{10+}$ | -60.2916601 | -15.1867592 | -6.8132825 |
| $Mg^{11+}$ | -71.7718495 | -18.0665680 | -8.0987465 |
| $Al^{12+}$ | -84.2520386 | -21.1963776 | -9.4952153 |
| $Si^{13+}$ | -97.7322276 | -24.5761491 | -11.0028199 |
| $P^{14+}$ | -112.2124166 | -28.2059659 | -12.6215260 |
| $S^{15+}$ | -127.6926056 | -32.0857668 | -14.3513619 |
| $Cl^{16+}$ | -144.1727948 | -36.2155565 | -16.1922981 |
| $Ar^{17+}$ | -161.6529841 | -40.5953437 | -18.1443646 |
| $K^{18+}$ | -180.1331736 | -45.2251905 | -20.2076044 |
| $Ca^{19+}$ | -199.6133632 | -50.1048965 | -22.3818922 |
| $Sc^{20+}$ | -220.0935529 | -55.2346760 | -24.6671549 |
| $Ti^{21+}$ | -241.5737428 | -60.6144293 | -27.0636798 |
| $V^{22+}$ | -264.0539329 | -66.2442542 | -29.5712272 |
| $Cr^{23+}$ | -287.5341231 | -72.1240239 | -32.1899908 |
| $Mn^{24+}$ | -312.0143135 | -78.2538104 | -34.9197891 |
| $Fe^{25+}$ | -337.4945040 | -84.6335618 | -37.7606682 |
| $Co^{26+}$ | -363.9746946 | -91.2633391 | -40.7127450 |
| $Ni^{27+}$ | -391.4548853 | -98.1431392 | -43.7758882 |
| $Cu^{28+}$ | -419.9350762 | -105.2728544 | -46.9500699 |
| $Zn^{29+}$ | -449.4152671 | -112.6526728 | -50.2355075 |
| $Ga^{30+}$ | -479.8954582 | -120.2824632 | -53.6319395 |
| $Ge^{31+}$ | -511.3756493 | -128.1622371 | -57.1395648 |
| $As^{32+}$ | -543.8558406 | -136.2920106 | -60.7582602 |
| $Se^{33+}$ | -577.3360319 | -144.6717838 | -64.4880046 |
| $Br^{34+}$ | -611.8162233 | -153.3015567 | -68.3289361 |
| $Kr^{35+}$ | -647.2964148 | -162.1813133 | -72.2810104 |

Table S29. Total energies for ωB97X-D for the $1s$, $2p$, and $3d$ states calculated with PySCF using exponents from the AHGBSP3-9 basis set.

| System | $E_{\mathrm{tot}}^{1s}$ [$E_\mathrm{h}$] | $E_{\mathrm{tot}}^{2p}$ [$E_\mathrm{h}$] | $E_{\mathrm{tot}}^{3d}$ [$E_\mathrm{h}$] |
|---|---|---|---|
| $H^{0}$ | -0.5029573 | -0.1365196 | -0.0618589 |
| $He^{+}$ | -2.0013626 | -0.5257864 | -0.2402518 |
| $Li^{2+}$ | -4.5040873 | -1.1658718 | -0.5325461 |
| $Be^{3+}$ | -8.0085475 | -2.0572735 | -0.9369332 |
| $B^{4+}$ | -12.5137923 | -3.1997185 | -1.4531158 |
| $C^{5+}$ | -18.0194389 | -4.5928909 | -2.0810695 |
| $N^{6+}$ | -24.5253093 | -6.2365799 | -2.8205633 |
| $O^{7+}$ | -32.0313125 | -8.1306375 | -3.6716713 |
| $F^{8+}$ | -40.5373969 | -10.2749311 | -4.6262774 |
| $Ne^{9+}$ | -50.0435334 | -12.6694297 | -5.6992959 |
| $Na^{10+}$ | -60.5497036 | -15.3140970 | -6.8934980 |
| $Mg^{11+}$ | -72.0558943 | -18.2088330 | -8.1901650 |
| $Al^{12+}$ | -84.5620994 | -21.3536821 | -9.5979436 |
| $Si^{13+}$ | -98.0683134 | -24.7484741 | -11.1172221 |
| $P^{14+}$ | -112.5745315 | -28.3935056 | -12.7473517 |
| $S^{15+}$ | -128.0807522 | -32.2885341 | -14.4892184 |
| $Cl^{16+}$ | -144.5869735 | -36.4335652 | -16.3415905 |
| $Ar^{17+}$ | -162.0931946 | -40.8286245 | -18.3053989 |
| $K^{18+}$ | -180.5994139 | -45.4739510 | -20.3809104 |
| $Ca^{19+}$ | -200.1056318 | -50.3687417 | -22.5490162 |
| $Sc^{20+}$ | -220.6118463 | -55.5138488 | -24.8639572 |
| $Ti^{21+}$ | -242.1180586 | -60.9088727 | -27.2725391 |
| $V^{22+}$ | -264.6242682 | -66.5542000 | -29.7919859 |
| $Cr^{23+}$ | -288.1304743 | -72.4493136 | -32.4018708 |
| $Mn^{24+}$ | -312.6366777 | -78.5945116 | -35.1648534 |
| $Fe^{25+}$ | -338.1428775 | -84.9895605 | -37.9951572 |
| $Co^{26+}$ | -364.6490751 | -91.6347978 | -40.9820614 |
| $Ni^{27+}$ | -392.1552685 | -98.5300273 | -44.0573578 |
| $Cu^{28+}$ | -420.6614592 | -105.6749595 | -47.2436298 |
| $Zn^{29+}$ | -450.1676476 | -113.0703422 | -50.5417213 |
| $Ga^{30+}$ | -480.6738334 | -120.7155808 | -53.9498509 |
| $Ge^{31+}$ | -512.1800157 | -128.6107708 | -57.4697863 |
| $As^{32+}$ | -544.6861961 | -136.7559629 | -61.1006978 |
| $Se^{33+}$ | -578.1923713 | -145.1511566 | -64.8435445 |
| $Br^{34+}$ | -612.6985480 | -153.7963519 | -68.6956592 |
| $Kr^{35+}$ | -648.2047201 | -162.6914763 | -72.6601470 |

Table S30. Total energies for OLYP for the $1s$, $2p$, and $3d$ states calculated with PySCF using exponents from the AHGBSP3-9 basis set.

| System | $E_{\rm tot}^{1s}$ $[E_{\rm h}]$ | $E_{\rm tot}^{2p}$ $[E_{\rm h}]$ | $E_{\rm tot}^{3d}$ $[E_{\rm h}]$ |
|---|---|---|---|
| $H^{0}$ | -0.4986598 | -0.1394531 | -0.0706339 |
| $He^{+}$ | -1.9967093 | -0.5283445 | -0.2510341 |
| $Li^{2+}$ | -4.4947886 | -1.1672359 | -0.5426154 |
| $Be^{3+}$ | -7.9928741 | -2.0561457 | -0.9452911 |
| $B^{4+}$ | -12.4909621 | -3.1950465 | -1.4590826 |
| $C^{5+}$ | -17.9890512 | -4.5839461 | -2.0840318 |
| $N^{6+}$ | -24.4871409 | -6.2228485 | -2.8200118 |
| $O^{7+}$ | -31.9852310 | -8.1117569 | -3.6671574 |
| $F^{8+}$ | -40.4833214 | -10.2506549 | -4.6253769 |
| $Ne^{9+}$ | -49.9814120 | -12.6395644 | -5.6828993 |
| $Na^{10+}$ | -60.4795027 | -15.2784751 | -6.8752199 |
| $Mg^{11+}$ | -71.9775935 | -18.1673739 | -8.1668743 |
| $Al^{12+}$ | -84.4756844 | -21.3062836 | -9.5694603 |
| $Si^{13+}$ | -97.9737754 | -24.6951461 | -11.0833316 |
| $P^{14+}$ | -112.4718663 | -28.3340802 | -12.7081796 |
| $S^{15+}$ | -127.9699573 | -32.2229966 | -14.4441818 |
| $Cl^{16+}$ | -144.4680484 | -36.3619009 | -16.2913147 |
| $Ar^{17+}$ | -161.9661395 | -40.7508053 | -18.2495861 |
| $K^{18+}$ | -180.4642305 | -45.3897990 | -20.3190568 |
| $Ca^{19+}$ | -199.9623217 | -50.2785913 | -22.4759832 |
| $Sc^{20+}$ | -220.4604128 | -55.4174923 | -24.7909867 |
| $Ti^{21+}$ | -241.9585039 | -60.8063570 | -27.1937381 |
| $V^{22+}$ | -264.4565951 | -66.4453270 | -29.7074751 |
| $Cr^{23+}$ | -287.9546862 | -72.3342187 | -32.3324759 |
| $Mn^{24+}$ | -312.4527773 | -78.4731357 | -35.0684807 |
| $Fe^{25+}$ | -337.9508685 | -84.8620034 | -37.8851611 |
| $Co^{26+}$ | -364.4489597 | -91.5009271 | -40.8738647 |
| $Ni^{27+}$ | -391.9470508 | -98.3898488 | -43.9432234 |
| $Cu^{28+}$ | -420.4451419 | -105.5286666 | -47.1235928 |
| $Zn^{29+}$ | -449.9432331 | -112.9176339 | -50.4153017 |
| $Ga^{30+}$ | -480.4413243 | -120.5565619 | -53.8179064 |
| $Ge^{31+}$ | -511.9394155 | -128.4454662 | -57.3317693 |
| $As^{32+}$ | -544.4375067 | -136.5843706 | -60.9566836 |
| $Se^{33+}$ | -577.9355978 | -144.9732750 | -64.6926138 |
| $Br^{34+}$ | -612.4336891 | -153.6121793 | -68.5397845 |
| $Kr^{35+}$ | -647.9317803 | -162.5010606 | -72.4980930 |

Table S31. Total energies for LRC-$\omega$PBE for the $1s$, $2p$, and $3d$ states calculated with PySCF using exponents from the AHGBSP3-9 basis set.

| System | $E_{\mathrm{tot}}^{1s}$ [$E_\mathrm{h}$] | $E_{\mathrm{tot}}^{2p}$ [$E_\mathrm{h}$] | $E_{\mathrm{tot}}^{3d}$ [$E_\mathrm{h}$] |
|---|---|---|---|
| $H^{0}$ | -0.5046907 | -0.1333184 | -0.0593609 |
| $He^{+}$ | -1.9966504 | -0.5215719 | -0.2329566 |
| $Li^{2+}$ | -4.4890083 | -1.1590354 | -0.5229881 |
| $Be^{3+}$ | -7.9818682 | -2.0450204 | -0.9254382 |
| $B^{4+}$ | -12.4749728 | -3.1802430 | -1.4386347 |
| $C^{5+}$ | -17.9682019 | -4.5651124 | -2.0622731 |
| $N^{6+}$ | -24.4615000 | -6.1998210 | -2.7964450 |
| $O^{7+}$ | -31.9548394 | -8.0844521 | -3.6412965 |
| $F^{8+}$ | -40.4482049 | -10.2190428 | -4.5969311 |
| $Ne^{9+}$ | -49.9415880 | -12.6036175 | -5.6522940 |
| $Na^{10+}$ | -60.4349833 | -15.2381896 | -6.8409709 |
| $Mg^{11+}$ | -71.9283873 | -18.1227486 | -8.1295145 |
| $Al^{12+}$ | -84.4217978 | -21.2573130 | -9.5289891 |
| $Si^{13+}$ | -97.9152133 | -24.6418479 | -11.0395803 |
| $P^{14+}$ | -112.4086326 | -28.2764294 | -12.6611716 |
| $S^{15+}$ | -127.9020550 | -32.1610005 | -14.3938828 |
| $Cl^{16+}$ | -144.3954797 | -36.2955655 | -16.2376797 |
| $Ar^{17+}$ | -161.8889065 | -40.6801318 | -18.1925876 |
| $K^{18+}$ | -180.3823349 | -45.3147561 | -20.2586567 |
| $Ca^{19+}$ | -199.8757647 | -50.1992523 | -22.4357636 |
| $Sc^{20+}$ | -220.3691957 | -55.3338194 | -24.7238440 |
| $Ti^{21+}$ | -241.8626276 | -60.7183645 | -27.1231702 |
| $V^{22+}$ | -264.3560604 | -66.3529801 | -29.6335197 |
| $Cr^{23+}$ | -287.8494940 | -72.2375428 | -32.2550811 |
| $Mn^{24+}$ | -312.3429281 | -78.3721256 | -34.9876727 |
| $Fe^{25+}$ | -337.8363628 | -84.7566711 | -37.8313388 |
| $Co^{26+}$ | -364.3297981 | -91.3912611 | -40.7862099 |
| $Ni^{27+}$ | -391.8232337 | -98.2758486 | -43.8521411 |
| $Cu^{28+}$ | -420.3166698 | -105.4103652 | -47.0291104 |
| $Zn^{29+}$ | -449.8101062 | -112.7949861 | -50.3172046 |
| $Ga^{30+}$ | -480.3035429 | -120.4295759 | -53.7165483 |
| $Ge^{31+}$ | -511.7969799 | -128.3141524 | -57.2269583 |
| $As^{32+}$ | -544.2904171 | -136.4487292 | -60.8484370 |
| $Se^{33+}$ | -577.7838546 | -144.8333064 | -64.5809648 |
| $Br^{34+}$ | -612.2772923 | -153.4678838 | -68.4246673 |
| $Kr^{35+}$ | -647.7707302 | -162.3524442 | -72.3795342 |

Table S32. Total energies for revTPSS for the 1$s$, 2$p$, and 3$d$ states calculated with PySCF using exponents from the AHGBSP3-9 basis set.

| System | $E_{\text{tot}}^{1s}$ [$E_\text{h}$] | $E_{\text{tot}}^{2p}$ [$E_\text{h}$] | $E_{\text{tot}}^{3d}$ [$E_\text{h}$] |
|---|---|---|---|
| $H^{0}$ | -0.5001575 | -0.1364150 | -0.0665764 |
| $He^{+}$ | -2.0001425 | -0.5224983 | -0.2433980 |
| $Li^{2+}$ | -4.5001346 | -1.1585738 | -0.5313792 |
| $Be^{3+}$ | -8.0001283 | -2.0446618 | -0.9304604 |
| $B^{4+}$ | -12.5001226 | -3.1807432 | -1.4406559 |
| $C^{5+}$ | -18.0001172 | -4.5668240 | -2.0619950 |
| $N^{6+}$ | -24.5001119 | -6.2029066 | -2.7943895 |
| $O^{7+}$ | -32.0001067 | -8.0889933 | -3.6379327 |
| $F^{8+}$ | -40.5001016 | -10.2250729 | -4.5925604 |
| $Ne^{9+}$ | -50.0000965 | -12.6111570 | -5.6472841 |
| $Na^{10+}$ | -60.5000915 | -15.2472487 | -6.8351858 |
| $Mg^{11+}$ | -72.0000865 | -18.1333288 | -8.1232337 |
| $Al^{12+}$ | -84.5000815 | -21.2694164 | -9.5222521 |
| $Si^{13+}$ | -98.0000765 | -24.6554711 | -11.0325012 |
| $P^{14+}$ | -112.5000716 | -28.2915753 | -12.6537740 |
| $S^{15+}$ | -128.0000666 | -32.1776679 | -14.3861811 |
| $Cl^{16+}$ | -144.5000616 | -36.3137515 | -16.2297160 |
| $Ar^{17+}$ | -162.0000567 | -40.6998357 | -18.1843803 |
| $K^{18+}$ | -180.5000517 | -45.3359818 | -20.2502166 |
| $Ca^{19+}$ | -200.0000468 | -50.2219922 | -22.4051266 |
| $Sc^{20+}$ | -220.5000418 | -55.3580692 | -24.7149851 |
| $Ti^{21+}$ | -242.0000369 | -60.7441254 | -27.1141191 |
| $V^{22+}$ | -264.5000320 | -66.3802550 | -29.6242766 |
| $Cr^{23+}$ | -288.0000270 | -72.2663301 | -32.2456491 |
| $Mn^{24+}$ | -312.5000221 | -78.4024228 | -34.9780631 |
| $Fe^{25+}$ | -338.0000171 | -84.7884811 | -37.8215494 |
| $Co^{26+}$ | -364.5000122 | -91.4245784 | -40.7762481 |
| $Ni^{27+}$ | -392.0000072 | -98.3106744 | -43.8420072 |
| $Cu^{28+}$ | -420.5000022 | -105.4466980 | -47.0188084 |
| $Zn^{29+}$ | -449.9999973 | -112.8328256 | -50.3068200 |
| $Ga^{30+}$ | -480.4999924 | -120.4689260 | -53.7059035 |
| $Ge^{31+}$ | -511.9999874 | -128.3550098 | -57.2161549 |
| $As^{32+}$ | -544.4999824 | -136.4910937 | -60.8374696 |
| $Se^{33+}$ | -577.9999775 | -144.8771775 | -64.5698262 |
| $Br^{34+}$ | -612.4999725 | -153.5132614 | -68.4133858 |
| $Kr^{35+}$ | -647.9999676 | -162.3993292 | -72.3680804 |

Table S33. Total energies for LC-VV10 for the 1$s$, 2$p$, and 3$d$ states calculated with PySCF using exponents from the AHGBSP3-9 basis set.

| System | $E_{\rm tot}^{1s}$ [$E_{\rm h}$] | $E_{\rm tot}^{2p}$ [$E_{\rm h}$] | $E_{\rm tot}^{3d}$ [$E_{\rm h}$] |
|---|---|---|---|
| $H^{0}$ | -0.5027569 | -0.1272593 | -0.0551720 |
| $He^{+}$ | -1.9956088 | -0.5121425 | -0.2246466 |
| $Li^{2+}$ | -4.4871670 | -1.1503101 | -0.5099565 |
| $Be^{3+}$ | -7.9793162 | -2.0378310 | -0.9102066 |
| $B^{4+}$ | -12.4719280 | -3.1742733 | -1.4232638 |
| $C^{5+}$ | -17.9648204 | -4.5599486 | -2.0477960 |
| $N^{6+}$ | -24.4578829 | -6.1951595 | -2.7832201 |
| $O^{7+}$ | -31.9510525 | -8.0800918 | -3.6293469 |
| $F^{8+}$ | -40.4442923 | -10.2148616 | -4.5861518 |
| $Ne^{9+}$ | -49.9375797 | -12.5995386 | -5.6434370 |
| $Na^{10+}$ | -60.4309007 | -15.2341636 | -6.8320374 |
| $Mg^{11+}$ | -71.9242460 | -18.1187485 | -8.1212753 |
| $Al^{12+}$ | -84.4176092 | -21.2533183 | -9.5213414 |
| $Si^{13+}$ | -97.9109861 | -24.6378512 | -11.0324028 |
| $P^{14+}$ | -112.4043735 | -28.2724188 | -12.6544173 |
| $S^{15+}$ | -127.8977692 | -32.1569724 | -14.3874540 |
| $Cl^{16+}$ | -144.3911714 | -36.2915190 | -16.2315276 |
| $Ar^{17+}$ | -161.8845790 | -40.6760659 | -18.1866649 |
| $K^{18+}$ | -180.3779909 | -45.3106678 | -20.2529225 |
| $Ca^{19+}$ | -199.8714064 | -50.1951487 | -22.4301905 |
| $Sc^{20+}$ | -220.3648249 | -55.3296970 | -24.7184151 |
| $Ti^{21+}$ | -241.8582460 | -60.7142245 | -27.1178617 |
| $V^{22+}$ | -264.3516691 | -66.3488209 | -29.6283205 |
| $Cr^{23+}$ | -287.8450941 | -72.2333680 | -32.2499650 |
| $Mn^{24+}$ | -312.3385207 | -78.3679345 | -34.9826315 |
| $Fe^{25+}$ | -337.8319486 | -84.7524665 | -37.8263692 |
| $Co^{26+}$ | -364.3253778 | -91.3870423 | -40.7812923 |
| $Ni^{27+}$ | -391.8188079 | -98.2716161 | -43.8472736 |
| $Cu^{28+}$ | -420.3122390 | -105.4061219 | -47.0242932 |
| $Zn^{29+}$ | -449.8056709 | -112.7907305 | -50.3125622 |
| $Ga^{30+}$ | -480.2991035 | -120.4253089 | -53.7117997 |
| $Ge^{31+}$ | -511.7925367 | -128.3098753 | -57.2222366 |
| $As^{32+}$ | -544.2859705 | -136.4444426 | -60.8437416 |
| $Se^{33+}$ | -577.7794049 | -144.8290107 | -64.5762948 |
| $Br^{34+}$ | -612.2728396 | -153.4635796 | -68.4200292 |
| $Kr^{35+}$ | -647.7662749 | -162.3481326 | -72.3749012 |

Table S34. Total energies for BLYP35 for the $1s$, $2p$, and $3d$ states calculated with PySCF using exponents from the AHGBSP3-9 basis set.

| System | $E_{\mathrm{tot}}^{1s}$ $[E_{\mathrm{h}}]$ | $E_{\mathrm{tot}}^{2p}$ $[E_{\mathrm{h}}]$ | $E_{\mathrm{tot}}^{3d}$ $[E_{\mathrm{h}}]$ |
|---|---|---|---|
| $H^{0}$ | -0.4984828 | -0.1335281 | -0.0646263 |
| $He^{+}$ | -1.9966892 | -0.5169048 | -0.2399785 |
| $Li^{2+}$ | -4.4949022 | -1.1503014 | -0.5263777 |
| $Be^{3+}$ | -7.9931168 | -2.0336480 | -0.9239362 |
| $B^{4+}$ | -12.4913321 | -3.1670288 | -1.4325919 |
| $C^{5+}$ | -17.9895476 | -4.5504144 | -2.0523650 |
| $N^{6+}$ | -24.4877633 | -6.1837954 | -2.7832348 |
| $O^{7+}$ | -31.9859791 | -8.0671641 | -3.6252672 |
| $F^{8+}$ | -40.4841949 | -10.2005409 | -4.5783337 |
| $Ne^{9+}$ | -49.9824108 | -12.5839080 | -5.6350695 |
| $Na^{10+}$ | -60.4806267 | -15.2171683 | -6.8179143 |
| $Mg^{11+}$ | -71.9788427 | -18.1006374 | -8.1044225 |
| $Al^{12+}$ | -84.4770587 | -21.2338944 | -9.5018398 |
| $Si^{13+}$ | -97.9752746 | -24.6174748 | -11.0106286 |
| $P^{14+}$ | -112.4734906 | -28.2507487 | -12.6302564 |
| $S^{15+}$ | -127.9717066 | -32.1339865 | -14.3612081 |
| $Cl^{16+}$ | -144.4699227 | -36.2673505 | -16.2032515 |
| $Ar^{17+}$ | -161.9681387 | -40.6507145 | -18.1562311 |
| $K^{18+}$ | -180.4663547 | -45.2843715 | -20.2205897 |
| $Ca^{19+}$ | -199.9645707 | -50.1676536 | -22.3959264 |
| $Sc^{20+}$ | -220.4627867 | -55.3010325 | -24.6821754 |
| $Ti^{21+}$ | -241.9610027 | -60.6845102 | -27.0792359 |
| $V^{22+}$ | -264.4592188 | -66.3175345 | -29.5883211 |
| $Cr^{23+}$ | -287.9574348 | -72.2009819 | -32.2084001 |
| $Mn^{24+}$ | -312.4556508 | -78.3342625 | -34.9384676 |
| $Fe^{25+}$ | -337.9538668 | -84.7179201 | -37.7810642 |
| $Co^{26+}$ | -364.4520828 | -91.3512278 | -40.7335110 |
| $Ni^{27+}$ | -391.9502989 | -98.2343544 | -43.7976994 |
| $Cu^{28+}$ | -420.4485149 | -105.3681660 | -46.9736385 |
| $Zn^{29+}$ | -449.9467309 | -112.7515443 | -50.2600217 |
| $Ga^{30+}$ | -480.4449469 | -120.3844463 | -53.6576616 |
| $Ge^{31+}$ | -511.9431629 | -128.2678103 | -57.1655639 |
| $As^{32+}$ | -544.4413789 | -136.4011743 | -60.7853078 |
| $Se^{33+}$ | -577.9395950 | -144.7845383 | -64.5168880 |
| $Br^{34+}$ | -612.4378110 | -153.4179022 | -68.3589397 |
| $Kr^{35+}$ | -647.9360270 | -162.3015056 | -72.3112062 |

Table S35. Total energies for HSE12 for the 1$s$, 2$p$, and 3$d$ states calculated with PySCF using exponents from the AHGBSP3-9 basis set.

| System | $E_{\text{tot}}^{1s}$ $[E_\text{h}]$ | $E_{\text{tot}}^{2p}$ $[E_\text{h}]$ | $E_{\text{tot}}^{3d}$ $[E_\text{h}]$ |
|---|---|---|---|
| $H^{0}$ | -0.5018396 | -0.1368696 | -0.0678529 |
| $He^{+}$ | -1.9980735 | -0.5192271 | -0.2416431 |
| $Li^{2+}$ | -4.4939743 | -1.1512728 | -0.5266730 |
| $Be^{3+}$ | -7.9898009 | -2.0331547 | -0.9228404 |
| $B^{4+}$ | -12.4856061 | -3.1649485 | -1.4301082 |
| $C^{5+}$ | -17.9814012 | -4.5466935 | -2.0484633 |
| $N^{6+}$ | -24.4771956 | -6.1784048 | -2.7779077 |
| $O^{7+}$ | -31.9729866 | -8.0600982 | -3.6184543 |
| $F^{8+}$ | -40.4687791 | -10.1917799 | -4.5701356 |
| $Ne^{9+}$ | -49.9645698 | -12.5734501 | -5.6247423 |
| $Na^{10+}$ | -60.4603648 | -15.2051200 | -6.8066875 |
| $Mg^{11+}$ | -71.9561521 | -18.0867721 | -8.0917134 |
| $Al^{12+}$ | -84.4519524 | -21.2184320 | -9.4877150 |
| $Si^{13+}$ | -97.9477446 | -24.6000622 | -10.9948967 |
| $P^{14+}$ | -112.4435353 | -28.2317225 | -12.6131253 |
| $S^{15+}$ | -127.9393347 | -32.1133769 | -14.3425088 |
| $Cl^{16+}$ | -144.4351230 | -36.2450212 | -16.1829840 |
| $Ar^{17+}$ | -161.9309212 | -40.6266647 | -18.1346076 |
| $K^{18+}$ | -180.4267191 | -45.2583302 | -20.1974579 |
| $Ca^{19+}$ | -199.9225166 | -50.1399366 | -22.3712816 |
| $Sc^{20+}$ | -220.4183134 | -55.2715677 | -24.6560701 |
| $Ti^{21+}$ | -241.9141097 | -60.6531952 | -27.0521159 |
| $V^{22+}$ | -264.4099051 | -66.2848662 | -29.5592465 |
| $Cr^{23+}$ | -287.9056998 | -72.1664924 | -32.1775887 |
| $Mn^{24+}$ | -312.4014934 | -78.2981427 | -34.9068947 |
| $Fe^{25+}$ | -337.8973055 | -84.6797658 | -37.7473552 |
| $Co^{26+}$ | -364.3930982 | -91.3114012 | -40.6989661 |
| $Ni^{27+}$ | -391.8888897 | -98.1930548 | -43.7616674 |
| $Cu^{28+}$ | -420.3847023 | -105.3246492 | -46.9354487 |
| $Zn^{29+}$ | -449.8804925 | -112.7063081 | -50.2202704 |
| $Ga^{30+}$ | -480.3762813 | -120.3379644 | -53.6164413 |
| $Ge^{31+}$ | -511.8720942 | -128.2196010 | -57.1235808 |
| $As^{32+}$ | -544.3678813 | -136.3512367 | -60.7418363 |
| $Se^{33+}$ | -577.8636945 | -144.7328717 | -64.4712313 |
| $Br^{34+}$ | -612.3594799 | -153.3645091 | -68.3116622 |
| $Kr^{35+}$ | -647.8552933 | -162.2461270 | -72.2632670 |

Table S36. Total energies for M11-L for the $1s$, $2p$, and $3d$ states calculated with PySCF using exponents from the AHGBSP3-9 basis set.

| System | $E_{\rm tot}^{1s}$ [$E_{\rm h}$] | $E_{\rm tot}^{2p}$ [$E_{\rm h}$] | $E_{\rm tot}^{3d}$ [$E_{\rm h}$] |
|---|---|---|---|
| $H^{0}$ | -0.5103506 | -0.1535856 | -0.0852478 |
| $He^{+}$ | -2.0141911 | -0.5434351 | -0.2740733 |
| $Li^{2+}$ | -4.5255961 | -1.1839485 | -0.5689698 |
| $Be^{3+}$ | -8.0371745 | -2.0739043 | -0.9745300 |
| $B^{4+}$ | -12.5486366 | -3.2138038 | -1.4902415 |
| $C^{5+}$ | -18.0600739 | -4.6035208 | -2.1167069 |
| $N^{6+}$ | -24.5715122 | -6.2433703 | -2.8540665 |
| $O^{7+}$ | -32.0830501 | -8.1330924 | -3.7011140 |
| $F^{8+}$ | -40.5946281 | -10.2727067 | -4.6610366 |
| $Ne^{9+}$ | -50.1063155 | -12.6624489 | -5.7322472 |
| $Na^{10+}$ | -60.6180913 | -15.3022472 | -6.9119530 |
| $Mg^{11+}$ | -72.1299103 | -18.1919581 | -8.2055154 |
| $Al^{12+}$ | -84.6418236 | -21.3317308 | -9.6073799 |
| $Si^{13+}$ | -98.1538179 | -24.7219200 | -11.1226758 |
| $P^{14+}$ | -112.6658449 | -28.3612507 | -12.7480349 |
| $S^{15+}$ | -128.1779368 | -32.2510728 | -14.4880840 |
| $Cl^{16+}$ | -144.6900773 | -36.3908855 | -16.3331746 |
| $Ar^{17+}$ | -162.2022790 | -40.7807134 | -18.2920806 |
| $K^{18+}$ | -180.7145121 | -45.4201711 | -20.3637273 |
| $Ca^{19+}$ | -200.2268066 | -50.3103788 | -22.5268832 |
| $Sc^{20+}$ | -220.7391073 | -55.4502842 | -24.8355430 |
| $Ti^{21+}$ | -242.2514637 | -60.8408583 | -27.2410768 |
| $V^{22+}$ | -264.7638576 | -66.4800638 | -29.7546168 |
| $Cr^{23+}$ | -288.2762642 | -72.3699016 | -32.3816719 |
| $Mn^{24+}$ | -312.7887142 | -78.5098916 | -35.1189131 |
| $Fe^{25+}$ | -338.3011767 | -84.8993739 | -37.9673791 |
| $Co^{26+}$ | -364.8136871 | -91.5397306 | -40.9264188 |
| $Ni^{27+}$ | -392.3261922 | -98.4297112 | -43.9968544 |
| $Cu^{28+}$ | -420.8387299 | -105.5705916 | -47.1758502 |
| $Zn^{29+}$ | -450.3513033 | -112.9605922 | -50.4706244 |
| $Ga^{30+}$ | -480.8638981 | -120.5996121 | -53.8730853 |
| $Ge^{31+}$ | -512.3765002 | -128.4895954 | -57.3898039 |
| $As^{32+}$ | -544.8891413 | -136.6295868 | -61.0158410 |
| $Se^{33+}$ | -578.4017420 | -145.0195848 | -64.7306202 |
| $Br^{34+}$ | -612.9144429 | -153.6595898 | -68.5979804 |
| $Kr^{35+}$ | -648.4271149 | -162.5495611 | -72.5606665 |

Table S37. Total energies for MN12-L for the $1s$, $2p$, and $3d$ states calculated with PySCF using exponents from the AHGBSP3-9 basis set.

| System | $E_{\text{tot}}^{1s}$ $[E_\text{h}]$ | $E_{\text{tot}}^{2p}$ $[E_\text{h}]$ | $E_{\text{tot}}^{3d}$ $[E_\text{h}]$ |
|---|---|---|---|
| $H^{0}$ | -0.4923219 | -0.1352393 | -0.0746339 |
| $He^{+}$ | -2.0051046 | -0.5041623 | -0.2470336 |
| $Li^{2+}$ | -4.5155145 | -1.1286799 | -0.5275863 |
| $Be^{3+}$ | -8.0248044 | -2.0006660 | -0.9171540 |
| $B^{4+}$ | -12.5338701 | -3.1204490 | -1.4162551 |
| $C^{5+}$ | -18.0428612 | -4.4883357 | -2.0244385 |
| $N^{6+}$ | -24.5517488 | -6.1047017 | -2.7418106 |
| $O^{7+}$ | -32.0604886 | -7.9698446 | -3.5689072 |
| $F^{8+}$ | -40.5690457 | -10.0839932 | -4.5056977 |
| $Ne^{9+}$ | -50.0774070 | -12.4473199 | -5.5443937 |
| $Na^{10+}$ | -60.5855675 | -15.0599555 | -6.7092062 |
| $Mg^{11+}$ | -72.0935281 | -17.9219826 | -7.9762594 |
| $Al^{12+}$ | -84.6013009 | -21.0335099 | -9.3533384 |
| $Si^{13+}$ | -98.1088960 | -24.3945883 | -10.8408774 |
| $P^{14+}$ | -112.6163204 | -28.0052431 | -12.4388424 |
| $S^{15+}$ | -128.1235900 | -31.8655562 | -14.1476663 |
| $Cl^{16+}$ | -144.6307145 | -35.9755453 | -15.9662851 |
| $Ar^{17+}$ | -162.1377069 | -40.3352435 | -17.8963865 |
| $K^{18+}$ | -180.6445742 | -44.9445967 | -19.9367224 |
| $Ca^{19+}$ | -200.1513302 | -49.8038758 | -22.0877343 |
| $Sc^{20+}$ | -220.6579766 | -54.9128501 | -24.3490810 |
| $Ti^{21+}$ | -242.1645286 | -60.2716708 | -26.7215577 |
| $V^{22+}$ | -264.6709914 | -65.8801852 | -29.2048537 |
| $Cr^{23+}$ | -288.1773689 | -71.7385910 | -31.7990215 |
| $Mn^{24+}$ | -312.6836712 | -77.8468317 | -34.5037883 |
| $Fe^{25+}$ | -338.1899000 | -84.2049505 | -37.3199433 |
| $Co^{26+}$ | -364.6960662 | -90.8128840 | -40.2461373 |
| $Ni^{27+}$ | -392.2021660 | -97.6706941 | -43.2836230 |
| $Cu^{28+}$ | -420.7082100 | -104.7785095 | -46.4319446 |
| $Zn^{29+}$ | -450.2142030 | -112.1360012 | -49.6940187 |
| $Ga^{30+}$ | -480.7201469 | -119.7434442 | -53.0615447 |
| $Ge^{31+}$ | -512.2260419 | -127.6008151 | -56.5426303 |
| $As^{32+}$ | -544.7318966 | -135.7080908 | -60.1347064 |
| $Se^{33+}$ | -578.2377008 | -144.0652757 | -63.8380607 |
| $Br^{34+}$ | -612.7434818 | -152.6723747 | -67.6518761 |
| $Kr^{35+}$ | -648.2492194 | -161.5294186 | -71.5766674 |

Table S38. Total energies for MS0 for the 1$s$, 2$p$, and 3$d$ states calculated with PySCF using exponents from the AHGBSP3-9 basis set.

| System | $E_{\mathrm{tot}}^{1s}$ [$E_\mathrm{h}$] | $E_{\mathrm{tot}}^{2p}$ [$E_\mathrm{h}$] | $E_{\mathrm{tot}}^{3d}$ [$E_\mathrm{h}$] |
|---|---|---|---|
| $H^{0}$ | -0.5066733 | -0.1406326 | -0.0690755 |
| $He^{+}$ | -2.0067343 | -0.5259646 | -0.2451509 |
| $Li^{2+}$ | -4.5066795 | -1.1608438 | -0.5319699 |
| $Be^{3+}$ | -8.0066194 | -2.0455811 | -0.9297373 |
| $B^{4+}$ | -12.5065653 | -3.1802548 | -1.4385449 |
| $C^{5+}$ | -18.0065180 | -4.5648965 | -2.0584252 |
| $N^{6+}$ | -24.5064763 | -6.1995214 | -2.7893932 |
| $O^{7+}$ | -32.0064392 | -8.0841381 | -3.6314638 |
| $F^{8+}$ | -40.5064058 | -10.2187424 | -4.5846153 |
| $Ne^{9+}$ | -50.0063753 | -12.6033475 | -5.6378432 |
| $Na^{10+}$ | -60.5063473 | -15.2379498 | -6.8242701 |
| $Mg^{11+}$ | -72.0063212 | -18.1225438 | -8.1107923 |
| $Al^{12+}$ | -84.5062969 | -21.2571413 | -9.5083452 |
| $Si^{13+}$ | -98.0062740 | -24.6417140 | -11.0170600 |
| $P^{14+}$ | -112.5062522 | -28.2763213 | -12.6368345 |
| $S^{15+}$ | -128.0062316 | -32.1609189 | -14.3677451 |
| $Cl^{16+}$ | -144.5062118 | -36.2955100 | -16.2097705 |
| $Ar^{17+}$ | -162.0061928 | -40.6801007 | -18.1629220 |
| $K^{18+}$ | -180.5061745 | -45.3147353 | -20.2272331 |
| $Ca^{19+}$ | -200.0061568 | -50.1992696 | -22.4026076 |
| $Sc^{20+}$ | -220.5061396 | -55.3338577 | -24.6889955 |
| $Ti^{21+}$ | -242.0061230 | -60.7184275 | -27.0866061 |
| $V^{22+}$ | -264.5061067 | -66.3530496 | -29.5952630 |
| $Cr^{23+}$ | -288.0060909 | -72.2376325 | -32.2151097 |
| $Mn^{24+}$ | -312.5060754 | -78.3722280 | -34.9460122 |
| $Fe^{25+}$ | -338.0060603 | -84.7567989 | -37.7879991 |
| $Co^{26+}$ | -364.5060454 | -91.3913976 | -40.7411704 |
| $Ni^{27+}$ | -392.0060308 | -98.2759953 | -43.8054159 |
| $Cu^{28+}$ | -420.5060164 | -105.4105413 | -46.9807188 |
| $Zn^{29+}$ | -450.0060023 | -112.7951616 | -50.2671996 |
| $Ga^{30+}$ | -480.5059884 | -120.4297623 | -53.6647887 |
| $Ge^{31+}$ | -512.0059746 | -128.3143512 | -57.1735075 |
| $As^{32+}$ | -544.5059610 | -136.4489402 | -60.7933080 |
| $Se^{33+}$ | -578.0059477 | -144.8335291 | -64.5241739 |
| $Br^{34+}$ | -612.5059344 | -153.4681181 | -68.3662090 |
| $Kr^{35+}$ | -648.0059213 | -162.3526956 | -72.3193754 |

Table S39. Total energies for MS1 for the $1s$, $2p$, and $3d$ states calculated with PySCF using exponents from the AHGBSP3-9 basis set.

| System | $E_{\text{tot}}^{1s}$ [$E_\text{h}$] | $E_{\text{tot}}^{2p}$ [$E_\text{h}$] | $E_{\text{tot}}^{3d}$ [$E_\text{h}$] |
|---|---|---|---|
| $H^{0}$ | -0.5067130 | -0.1410713 | -0.0696416 |
| $He^{+}$ | -2.0067807 | -0.5268392 | -0.2462409 |
| $Li^{2+}$ | -4.5067289 | -1.1621489 | -0.5335874 |
| $Be^{3+}$ | -8.0066706 | -2.0473233 | -0.9318814 |
| $B^{4+}$ | -12.5066180 | -3.1824301 | -1.4412155 |
| $C^{5+}$ | -18.0065717 | -4.5675046 | -2.0616461 |
| $N^{6+}$ | -24.5065310 | -6.2025622 | -2.7931174 |
| $O^{7+}$ | -32.0064948 | -8.0876118 | -3.6357154 |
| $F^{8+}$ | -40.5064622 | -10.2226485 | -4.5893903 |
| $Ne^{9+}$ | -50.0064325 | -12.6076838 | -5.6429920 |
| $Na^{10+}$ | -60.5064051 | -15.2427216 | -6.8300956 |
| $Mg^{11+}$ | -72.0063798 | -18.1277478 | -8.1171571 |
| $Al^{12+}$ | -84.5063561 | -21.2627781 | -9.5152303 |
| $Si^{13+}$ | -98.0063338 | -24.6477814 | -11.0244451 |
| $P^{14+}$ | -112.5063127 | -28.2828225 | -12.6448092 |
| $S^{15+}$ | -128.0062927 | -32.1678532 | -14.3762081 |
| $Cl^{16+}$ | -144.5062735 | -36.3028767 | -16.2187600 |
| $Ar^{17+}$ | -162.0062552 | -40.6878998 | -18.1724383 |
| $K^{18+}$ | -180.5062375 | -45.3229708 | -20.2372817 |
| $Ca^{19+}$ | -200.0062204 | -50.2079326 | -22.4131849 |
| $Sc^{20+}$ | -220.5062038 | -55.3429529 | -24.7000925 |
| $Ti^{21+}$ | -242.0061878 | -60.7279534 | -27.0982324 |
| $V^{22+}$ | -264.5061721 | -66.3630108 | -29.6074131 |
| $Cr^{23+}$ | -288.0061569 | -72.2480256 | -32.2277902 |
| $Mn^{24+}$ | -312.5061420 | -78.3830541 | -34.9592185 |
| $Fe^{25+}$ | -338.0061274 | -84.7680558 | -37.8017291 |
| $Co^{26+}$ | -364.5061131 | -91.4030877 | -40.7554301 |
| $Ni^{27+}$ | -392.0060991 | -98.2881186 | -43.8202022 |
| $Cu^{28+}$ | -420.5060853 | -105.4230931 | -46.9960300 |
| $Zn^{29+}$ | -450.0060718 | -112.8081486 | -50.2830657 |
| $Ga^{30+}$ | -480.5060584 | -120.4431827 | -53.6811526 |
| $Ge^{31+}$ | -512.0060452 | -128.3282041 | -57.1904006 |
| $As^{32+}$ | -544.5060322 | -136.4632255 | -60.8107277 |
| $Se^{33+}$ | -578.0060194 | -144.8482468 | -64.5421161 |
| $Br^{34+}$ | -612.5060067 | -153.4832682 | -68.3846798 |
| $Kr^{35+}$ | -648.0059942 | -162.3682770 | -72.3383751 |

Table S40. Total energies for MS2 for the 1$s$, 2$p$, and 3$d$ states calculated with PySCF using exponents from the AHGBSP3-9 basis set.

| System | $E_{\mathrm{tot}}^{1s}$ [$E_\mathrm{h}$] | $E_{\mathrm{tot}}^{2p}$ [$E_\mathrm{h}$] | $E_{\mathrm{tot}}^{3d}$ [$E_\mathrm{h}$] |
|---|---|---|---|
| $H^{0}$ | -0.5067391 | -0.1414206 | -0.0700785 |
| $He^{+}$ | -2.0068102 | -0.5275284 | -0.2470756 |
| $Li^{2+}$ | -4.5067601 | -1.1631772 | -0.5348228 |
| $Be^{3+}$ | -8.0067029 | -2.0486910 | -0.9335170 |
| $B^{4+}$ | -12.5066511 | -3.1841368 | -1.4432515 |
| $C^{5+}$ | -18.0066057 | -4.5695498 | -2.0640842 |
| $N^{6+}$ | -24.5065656 | -6.2049461 | -2.7959548 |
| $O^{7+}$ | -32.0065300 | -8.0903313 | -3.6389465 |
| $F^{8+}$ | -40.5064980 | -10.2257098 | -4.5930310 |
| $Ne^{9+}$ | -50.0064688 | -12.6110866 | -5.6469382 |
| $Na^{10+}$ | -60.5064421 | -15.2464606 | -6.8345359 |
| $Mg^{11+}$ | -72.0064173 | -18.1318253 | -8.1220016 |
| $Al^{12+}$ | -84.5063941 | -21.2671944 | -9.5204717 |
| $Si^{13+}$ | -98.0063724 | -24.6525348 | -11.0300842 |
| $P^{14+}$ | -112.5063518 | -28.2879156 | -12.6508013 |
| $S^{15+}$ | -128.0063323 | -32.1732854 | -14.3826498 |
| $Cl^{16+}$ | -144.5063136 | -36.3086475 | -16.2256022 |
| $Ar^{17+}$ | -162.0062958 | -40.6940092 | -18.1796830 |
| $K^{18+}$ | -180.5062786 | -45.3294222 | -20.2449298 |
| $Ca^{19+}$ | -200.0062620 | -50.2147183 | -22.4212352 |
| $Sc^{20+}$ | -220.5062460 | -55.3500772 | -24.7085379 |
| $Ti^{21+}$ | -242.0062304 | -60.7354147 | -27.1070805 |
| $V^{22+}$ | -264.5062153 | -66.3708132 | -29.6166594 |
| $Cr^{23+}$ | -288.0062005 | -72.2561661 | -32.2374404 |
| $Mn^{24+}$ | -312.5061861 | -78.3915337 | -34.9692685 |
| $Fe^{25+}$ | -338.0061720 | -84.7768725 | -37.8121774 |
| $Co^{26+}$ | -364.5061582 | -91.4122438 | -40.7662813 |
| $Ni^{27+}$ | -392.0061447 | -98.2976139 | -43.8314542 |
| $Cu^{28+}$ | -420.5061314 | -105.4329238 | -47.0076777 |
| $Zn^{29+}$ | -450.0061184 | -112.8183202 | -50.2951480 |
| $Ga^{30+}$ | -480.5061055 | -120.4536938 | -53.6936042 |
| $Ge^{31+}$ | -512.0060928 | -128.3390538 | -57.2032551 |
| $As^{32+}$ | -544.5060803 | -136.4744137 | -60.8239828 |
| $Se^{33+}$ | -578.0060680 | -144.8597736 | -64.5557569 |
| $Br^{34+}$ | -612.5060558 | -153.4951336 | -68.3987300 |
| $Kr^{35+}$ | -648.0060437 | -162.3804801 | -72.3528321 |

Table S41. Total energies for BLOC for the $1s$, $2p$, and $3d$ states calculated with PySCF using exponents from the AHGBSP3-9 basis set.

| System | $E_{\mathrm{tot}}^{1s}$ [$E_{\mathrm{h}}$] | $E_{\mathrm{tot}}^{2p}$ [$E_{\mathrm{h}}$] | $E_{\mathrm{tot}}^{3d}$ [$E_{\mathrm{h}}$] |
|---|---|---|---|
| $H^{0}$ | -0.5002353 | -0.1370239 | -0.0672642 |
| $He^{+}$ | -2.0002197 | -0.5236688 | -0.2447027 |
| $Li^{2+}$ | -4.5002152 | -1.1603164 | -0.5333050 |
| $Be^{3+}$ | -8.0002130 | -2.0469672 | -0.9330047 |
| $B^{4+}$ | -12.5002118 | -3.1836160 | -1.4438195 |
| $C^{5+}$ | -18.0002111 | -4.5702644 | -2.0657821 |
| $N^{6+}$ | -24.5002105 | -6.2069145 | -2.7987910 |
| $O^{7+}$ | -32.0002101 | -8.0935647 | -3.6429529 |
| $F^{8+}$ | -40.5002098 | -10.2302157 | -4.5981995 |
| $Ne^{9+}$ | -50.0002095 | -12.6168673 | -5.6533367 |
| $Na^{10+}$ | -60.5002094 | -15.2535266 | -6.8420809 |
| $Mg^{11+}$ | -72.0002092 | -18.1401741 | -8.1307443 |
| $Al^{12+}$ | -84.5002091 | -21.2768293 | -9.5303956 |
| $Si^{13+}$ | -98.0002091 | -24.6634516 | -11.0412017 |
| $P^{14+}$ | -112.5002089 | -28.3001227 | -12.6631026 |
| $S^{15+}$ | -128.0002089 | -32.1867834 | -14.3961556 |
| $Cl^{16+}$ | -144.5002088 | -36.3234343 | -16.2403080 |
| $Ar^{17+}$ | -162.0002088 | -40.7100862 | -18.1955934 |
| $K^{18+}$ | -180.5002087 | -45.3467995 | -20.2620685 |
| $Ca^{19+}$ | -200.0002087 | -50.2333732 | -22.4171850 |
| $Sc^{20+}$ | -220.5002087 | -55.3700222 | -24.7280587 |
| $Ti^{21+}$ | -242.0002086 | -60.7566461 | -27.1278141 |
| $V^{22+}$ | -264.5002086 | -66.3933431 | -29.6385870 |
| $Cr^{23+}$ | -288.0002086 | -72.2799856 | -32.2605896 |
| $Mn^{24+}$ | -312.5002086 | -78.4166459 | -34.9936166 |
| $Fe^{25+}$ | -338.0002085 | -84.8032717 | -37.8377181 |
| $Co^{26+}$ | -364.5002085 | -91.4399366 | -40.7930405 |
| $Ni^{27+}$ | -392.0002084 | -98.3266000 | -43.8594192 |
| $Cu^{28+}$ | -420.5002084 | -105.4631914 | -47.0368341 |
| $Zn^{29+}$ | -450.0002084 | -112.8498865 | -50.3255341 |
| $Ga^{30+}$ | -480.5002084 | -120.4865542 | -53.7251753 |
| $Ge^{31+}$ | -512.0002083 | -128.3732056 | -57.2360449 |
| $As^{32+}$ | -544.5002083 | -136.5098569 | -60.8579791 |
| $Se^{33+}$ | -578.0002082 | -144.8965083 | -64.5909607 |
| $Br^{34+}$ | -612.5002083 | -153.5331597 | -68.4351330 |
| $Kr^{35+}$ | -648.0002082 | -162.4197950 | -72.3904484 |

Table S42. Total energies for CAM-QTP00 for the $1s$, $2p$, and $3d$ states calculated with PySCF using exponents from the AHGBSP3-9 basis set.

| System | $E_{\rm tot}^{1s}$ [$E_{\rm h}$] | $E_{\rm tot}^{2p}$ [$E_{\rm h}$] | $E_{\rm tot}^{3d}$ [$E_{\rm h}$] |
|---|---|---|---|
| $H^{0}$ | -0.5000690 | -0.1295158 | -0.0587234 |
| $He^{+}$ | -1.9939831 | -0.5088687 | -0.2288851 |
| $Li^{2+}$ | -4.4898251 | -1.1376532 | -0.5110779 |
| $Be^{3+}$ | -7.9868398 | -2.0163722 | -0.9045963 |
| $B^{4+}$ | -12.4844814 | -3.1453506 | -1.4091785 |
| $C^{5+}$ | -17.9824837 | -4.5246350 | -2.0248584 |
| $N^{6+}$ | -24.4807089 | -6.1541908 | -2.7516905 |
| $O^{7+}$ | -31.9790799 | -8.0339694 | -3.5897212 |
| $F^{8+}$ | -40.4775506 | -10.1639296 | -4.5389657 |
| $Ne^{9+}$ | -49.9760919 | -12.5440333 | -5.5943513 |
| $Na^{10+}$ | -60.4746847 | -15.1742432 | -6.7711138 |
| $Mg^{11+}$ | -71.9733159 | -18.0545761 | -8.0540108 |
| $Al^{12+}$ | -84.4719763 | -21.1849596 | -9.4480916 |
| $Si^{13+}$ | -97.9706592 | -24.5654235 | -10.9533699 |
| $P^{14+}$ | -112.4693599 | -28.1959542 | -12.5698376 |
| $S^{15+}$ | -127.9680745 | -32.0765083 | -14.2974799 |
| $Cl^{16+}$ | -144.4668003 | -36.2071139 | -16.1362613 |
| $Ar^{17+}$ | -161.9655352 | -40.5877536 | -18.0862321 |
| $K^{18+}$ | -180.4642774 | -45.2184809 | -20.1474024 |
| $Ca^{19+}$ | -199.9630256 | -50.0991247 | -22.3196884 |
| $Sc^{20+}$ | -220.4617787 | -55.2298374 | -24.6030650 |
| $Ti^{21+}$ | -241.9605359 | -60.6105479 | -26.9975956 |
| $V^{22+}$ | -264.4592964 | -66.2413255 | -29.5033337 |
| $Cr^{23+}$ | -287.9580596 | -72.1221022 | -32.1201799 |
| $Mn^{24+}$ | -312.4568251 | -78.2528778 | -34.8481459 |
| $Fe^{25+}$ | -337.9555925 | -84.6336581 | -37.6872903 |
| $Co^{26+}$ | -364.4543615 | -91.2644805 | -40.6375199 |
| $Ni^{27+}$ | -391.9531318 | -98.1452946 | -43.6989031 |
| $Cu^{28+}$ | -420.4519030 | -105.2760861 | -46.8714154 |
| $Zn^{29+}$ | -449.9506752 | -112.6569475 | -50.1550736 |
| $Ga^{30+}$ | -480.4494480 | -120.2877914 | -53.5498092 |
| $Ge^{31+}$ | -511.9482213 | -128.1686376 | -57.0557073 |
| $As^{32+}$ | -544.4469951 | -136.2994899 | -60.6727203 |
| $Se^{33+}$ | -577.9457692 | -144.6803475 | -64.4008283 |
| $Br^{34+}$ | -612.4445435 | -153.3112101 | -68.2400944 |
| $Kr^{35+}$ | -647.9433179 | -162.1920614 | -72.1904919 |

Table S43. Total energies for GAM for the $1s$, $2p$, and $3d$ states calculated with PySCF using exponents from the AHGBSP3-9 basis set.

| System | $E_{\mathrm{tot}}^{1s}$ [$E_{\mathrm{h}}$] | $E_{\mathrm{tot}}^{2p}$ [$E_{\mathrm{h}}$] | $E_{\mathrm{tot}}^{3d}$ [$E_{\mathrm{h}}$] |
|---|---|---|---|
| $H^{0}$ | -0.5013928 | -0.1426035 | -0.0750319 |
| $He^{+}$ | -2.0146402 | -0.5316592 | -0.2547607 |
| $Li^{2+}$ | -4.5276946 | -1.1760966 | -0.5468447 |
| $Be^{3+}$ | -8.0331271 | -2.0737710 | -0.9521381 |
| $B^{4+}$ | -12.5300327 | -3.2226013 | -1.4705470 |
| $C^{5+}$ | -18.0191394 | -4.6211609 | -2.1012874 |
| $N^{6+}$ | -24.5014911 | -6.2686420 | -2.8440999 |
| $O^{7+}$ | -31.9780860 | -8.1646043 | -3.6985269 |
| $F^{8+}$ | -40.4497869 | -10.3087951 | -4.6640520 |
| $Ne^{9+}$ | -49.9173163 | -12.7011740 | -5.7280538 |
| $Na^{10+}$ | -60.3812715 | -15.3417153 | -6.9279199 |
| $Mg^{11+}$ | -71.8421465 | -18.2304357 | -8.2259283 |
| $Al^{12+}$ | -84.3003509 | -21.3674515 | -9.6341730 |
| $Si^{13+}$ | -97.7562259 | -24.7527253 | -11.1529499 |
| $P^{14+}$ | -112.2100577 | -28.3865941 | -12.7821975 |
| $S^{15+}$ | -127.6620875 | -32.2689630 | -14.5216607 |
| $Cl^{16+}$ | -144.1125203 | -36.3999320 | -16.3715029 |
| $Ar^{17+}$ | -161.5615307 | -40.7796121 | -18.3318211 |
| $K^{18+}$ | -180.0092689 | -45.4082596 | -20.4027994 |
| $Ca^{19+}$ | -199.4558645 | -50.2853906 | -22.5606321 |
| $Sc^{20+}$ | -219.9014301 | -55.4116502 | -24.8745748 |
| $Ti^{21+}$ | -241.3460635 | -60.7868658 | -27.2763526 |
| $V^{22+}$ | -263.7898508 | -66.4113457 | -29.7882990 |
| $Cr^{23+}$ | -287.2328674 | -72.2847977 | -32.4109980 |
| $Mn^{24+}$ | -311.6751801 | -78.4074837 | -35.1438072 |
| $Fe^{25+}$ | -337.1168482 | -84.7792989 | -37.9599292 |
| $Co^{26+}$ | -363.5579241 | -91.4004692 | -40.9410359 |
| $Ni^{27+}$ | -390.9984551 | -98.2710043 | -44.0053918 |
| $Cu^{28+}$ | -419.4384831 | -105.3906933 | -47.1807212 |
| $Zn^{29+}$ | -448.8780460 | -112.7600140 | -50.4657862 |
| $Ga^{30+}$ | -479.3171777 | -120.3787024 | -53.8615418 |
| $Ge^{31+}$ | -510.7559094 | -128.2468056 | -57.3682453 |
| $As^{32+}$ | -543.1942687 | -136.3643945 | -60.9854155 |
| $Se^{33+}$ | -576.6322816 | -144.7314965 | -64.7130733 |
| $Br^{34+}$ | -611.0699697 | -153.3481368 | -68.5514602 |
| $Kr^{35+}$ | -646.5073555 | -162.2142986 | -72.5007191 |

Table S44. Total energies for CHACHIYO for the $1s$, $2p$, and $3d$ states calculated with PySCF using exponents from the AHGBSP3-9 basis set.

| System | $E_{\mathrm{tot}}^{1s}$ [$E_{\mathrm{h}}$] | $E_{\mathrm{tot}}^{2p}$ [$E_{\mathrm{h}}$] | $E_{\mathrm{tot}}^{3d}$ [$E_{\mathrm{h}}$] |
|---|---|---|---|
| $H^{0}$ | -0.4787475 | -0.1324260 | -0.0655627 |
| $He^{+}$ | -1.9415401 | -0.5067955 | -0.2369185 |
| $Li^{2+}$ | -4.4017776 | -1.1293920 | -0.5181465 |
| $Be^{3+}$ | -7.8608434 | -2.0011441 | -0.9098202 |
| $B^{4+}$ | -12.3192210 | -3.1223802 | -1.4122009 |
| $C^{5+}$ | -17.7771412 | -4.4932699 | -2.0254158 |
| $N^{6+}$ | -24.2347339 | -6.1139092 | -2.7495381 |
| $O^{7+}$ | -31.6920798 | -7.9843567 | -3.5846113 |
| $F^{8+}$ | -40.1492328 | -10.1046527 | -4.5306736 |
| $Ne^{9+}$ | -49.6062306 | -12.4748276 | -5.5780716 |
| $Na^{10+}$ | -60.0631008 | -15.0949004 | -6.7558446 |
| $Mg^{11+}$ | -71.5198641 | -17.9648815 | -8.0350244 |
| $Al^{12+}$ | -83.9765365 | -21.0847928 | -9.4251805 |
| $Si^{13+}$ | -97.4331308 | -24.4546206 | -10.9264147 |
| $P^{14+}$ | -111.8896570 | -28.0744207 | -12.5387110 |
| $S^{15+}$ | -127.3461235 | -31.9441637 | -14.2620872 |
| $Cl^{16+}$ | -143.8025371 | -36.0638573 | -16.0965347 |
| $Ar^{17+}$ | -161.2589036 | -40.4335111 | -18.0420728 |
| $K^{18+}$ | -179.7152278 | -45.0531643 | -20.0987321 |
| $Ca^{19+}$ | -199.1715137 | -49.9227048 | -22.2664339 |
| $Sc^{20+}$ | -219.6277651 | -55.0422588 | -24.5451438 |
| $Ti^{21+}$ | -241.0839850 | -60.4117712 | -26.9350318 |
| $V^{22+}$ | -263.5401759 | -66.0313004 | -29.4359580 |
| $Cr^{23+}$ | -286.9963404 | -71.9007752 | -32.0480377 |
| $Mn^{24+}$ | -311.4524804 | -78.0202390 | -34.7711665 |
| $Fe^{25+}$ | -336.9085978 | -84.3896632 | -37.6053683 |
| $Co^{26+}$ | -363.3646943 | -91.0090913 | -40.5507231 |
| $Ni^{27+}$ | -390.8207713 | -97.8785013 | -43.6071449 |
| $Cu^{28+}$ | -419.2768301 | -104.9978542 | -46.7746227 |
| $Zn^{29+}$ | -448.7328719 | -112.3672510 | -50.0532626 |
| $Ga^{30+}$ | -479.1888978 | -119.9866182 | -53.4429726 |
| $Ge^{31+}$ | -510.6449088 | -127.8559627 | -56.9438102 |
| $As^{32+}$ | -543.1009057 | -135.9752946 | -60.5557247 |
| $Se^{33+}$ | -576.5568894 | -144.3446146 | -64.2787053 |
| $Br^{34+}$ | -611.0128606 | -152.9639234 | -68.1128361 |
| $Kr^{35+}$ | -646.4688199 | -161.8332124 | -72.0580740 |

Table S45. Total energies for B97M-V for the 1$s$, 2$p$, and 3$d$ states calculated with PySCF using exponents from the AHGBSP3-9 basis set.

| System | $E_{\text{tot}}^{1s}$ $[E_{\text{h}}]$ | $E_{\text{tot}}^{2p}$ $[E_{\text{h}}]$ | $E_{\text{tot}}^{3d}$ $[E_{\text{h}}]$ |
|---|---|---|---|
| $H^{0}$ | -0.5015715 | -0.1308329 | -0.0655328 |
| $He^{+}$ | -2.0013747 | -0.5111412 | -0.2387801 |
| $Li^{2+}$ | -4.5010302 | -1.1421934 | -0.5227331 |
| $Be^{3+}$ | -8.0002899 | -2.0232376 | -0.9173978 |
| $B^{4+}$ | -12.4992160 | -3.1541572 | -1.4229787 |
| $C^{5+}$ | -17.9978806 | -4.5349506 | -2.0392099 |
| $N^{6+}$ | -24.4963393 | -6.1656313 | -2.7663929 |
| $O^{7+}$ | -31.9946331 | -8.0462131 | -3.6045592 |
| $F^{8+}$ | -40.4927920 | -10.1767100 | -4.5536016 |
| $Ne^{9+}$ | -49.9908390 | -12.5571351 | -5.6031070 |
| $Na^{10+}$ | -60.4887916 | -15.1874962 | -6.7846072 |
| $Mg^{11+}$ | -71.9866634 | -18.0677956 | -8.0666058 |
| $Al^{12+}$ | -84.4844655 | -21.1980498 | -9.4596747 |
| $Si^{13+}$ | -97.9822068 | -24.5782416 | -10.9638492 |
| $P^{14+}$ | -112.4798944 | -28.2084201 | -12.5789139 |
| $S^{15+}$ | -127.9775345 | -32.0885567 | -14.3051596 |
| $Cl^{16+}$ | -144.4751320 | -36.2186563 | -16.1423241 |
| $Ar^{17+}$ | -161.9726914 | -40.5987265 | -18.0907055 |
| $K^{18+}$ | -180.4702162 | -45.2288009 | -20.1501470 |
| $Ca^{19+}$ | -199.9677097 | -50.1087804 | -22.3016544 |
| $Sc^{20+}$ | -220.4651746 | -55.2387754 | -24.6019182 |
| $Ti^{21+}$ | -241.9626132 | -60.6187375 | -26.9945032 |
| $V^{22+}$ | -264.4600278 | -66.2487163 | -29.4982671 |
| $Cr^{23+}$ | -287.9574201 | -72.1286496 | -32.1130488 |
| $Mn^{24+}$ | -312.4547918 | -78.2585757 | -34.8387365 |
| $Fe^{25+}$ | -337.9521444 | -84.6384686 | -37.6757512 |
| $Co^{26+}$ | -364.4494792 | -91.2683652 | -40.6236460 |
| $Ni^{27+}$ | -391.9467974 | -98.1482501 | -43.6827320 |
| $Cu^{28+}$ | -420.4441000 | -105.2780859 | -46.8530373 |
| $Zn^{29+}$ | -449.9413881 | -112.6579593 | -50.1342725 |
| $Ga^{30+}$ | -480.4386625 | -120.2878082 | -53.5264766 |
| $Ge^{31+}$ | -511.9359240 | -128.1676384 | -57.0299830 |
| $As^{32+}$ | -544.4331734 | -136.2974585 | -60.6445280 |
| $Se^{33+}$ | -577.9304113 | -144.6772688 | -64.3703458 |
| $Br^{34+}$ | -612.4276383 | -153.3070699 | -68.2069794 |
| $Kr^{35+}$ | -647.9248551 | -162.1868545 | -72.1547354 |

Table S46. Total energies for TM for the 1$s$, 2$p$, and 3$d$ states calculated with PySCF using exponents from the AHGBSP3-9 basis set.

| System | $E_{\mathrm{tot}}^{1s}$ [$E_\mathrm{h}$] | $E_{\mathrm{tot}}^{2p}$ [$E_\mathrm{h}$] | $E_{\mathrm{tot}}^{3d}$ [$E_\mathrm{h}$] |
|---|---|---|---|
| $H^{0}$ | -0.5003412 | -0.1361547 | -0.0667734 |
| $He^{+}$ | -2.0003205 | -0.5225102 | -0.2438326 |
| $Li^{2+}$ | -4.5003142 | -1.1586146 | -0.5320396 |
| $Be^{3+}$ | -8.0003111 | -2.0447196 | -0.9313549 |
| $B^{4+}$ | -12.5003093 | -3.1808247 | -1.4417832 |
| $C^{5+}$ | -18.0003080 | -4.5669299 | -2.0633235 |
| $N^{6+}$ | -24.5003071 | -6.2030352 | -2.7959755 |
| $O^{7+}$ | -32.0003064 | -8.0891405 | -3.6397389 |
| $F^{8+}$ | -40.5003058 | -10.2252458 | -4.5946136 |
| $Ne^{9+}$ | -50.0003053 | -12.6113512 | -5.6605998 |
| $Na^{10+}$ | -60.5003049 | -15.2474566 | -6.8376969 |
| $Mg^{11+}$ | -72.0003045 | -18.1335619 | -8.1259055 |
| $Al^{12+}$ | -84.5003042 | -21.2696673 | -9.5252249 |
| $Si^{13+}$ | -98.0003039 | -24.6557726 | -11.0356557 |
| $P^{14+}$ | -112.5003036 | -28.2918781 | -12.6571976 |
| $S^{15+}$ | -128.0003033 | -32.1779834 | -14.3898503 |
| $Cl^{16+}$ | -144.5003031 | -36.3140888 | -16.2336145 |
| $Ar^{17+}$ | -162.0003028 | -40.7001942 | -18.1884901 |
| $K^{18+}$ | -180.5003026 | -45.3362997 | -20.2544766 |
| $Ca^{19+}$ | -200.0003024 | -50.2224050 | -22.4315744 |
| $Sc^{20+}$ | -220.5003021 | -55.3585103 | -24.7197826 |
| $Ti^{21+}$ | -242.0003019 | -60.7446156 | -27.1191026 |
| $V^{22+}$ | -264.5003017 | -66.3807210 | -29.6295335 |
| $Cr^{23+}$ | -288.0003015 | -72.2668265 | -32.2510754 |
| $Mn^{24+}$ | -312.5003013 | -78.4029318 | -34.9837287 |
| $Fe^{25+}$ | -338.0003011 | -84.7890372 | -37.8274928 |
| $Co^{26+}$ | -364.5003009 | -91.4251426 | -40.7823684 |
| $Ni^{27+}$ | -392.0003007 | -98.3112479 | -43.8483549 |
| $Cu^{28+}$ | -420.5003005 | -105.4473532 | -47.0254524 |
| $Zn^{29+}$ | -450.0003003 | -112.8334586 | -50.3136609 |
| $Ga^{30+}$ | -480.5003001 | -120.4695640 | -53.7129810 |
| $Ge^{31+}$ | -512.0002999 | -128.3556694 | -57.2234121 |
| $As^{32+}$ | -544.5002997 | -136.4917747 | -60.8449541 |
| $Se^{33+}$ | -578.0002995 | -144.8778801 | -64.5775980 |
| $Br^{34+}$ | -612.5002992 | -153.5139854 | -68.4213715 |
| $Kr^{35+}$ | -648.0002990 | -162.4000908 | -72.3762470 |

Table S47. Total energies for $\omega$B97M-V for the $1s$, $2p$, and $3d$ states calculated with PySCF using exponents from the AHGBSP3-9 basis set.

| System | $E_{\mathrm{tot}}^{1s}$ [$E_{\mathrm{h}}$] | $E_{\mathrm{tot}}^{2p}$ [$E_{\mathrm{h}}$] | $E_{\mathrm{tot}}^{3d}$ [$E_{\mathrm{h}}$] |
|---|---|---|---|
| $H^{0}$ | -0.4946779 | -0.1212856 | -0.0538435 |
| $He^{+}$ | -1.9892213 | -0.5051133 | -0.2256243 |
| $Li^{2+}$ | -4.4882141 | -1.1395341 | -0.5127037 |
| $Be^{3+}$ | -7.9897531 | -2.0237246 | -0.9118772 |
| $B^{4+}$ | -12.4926226 | -3.1581600 | -1.4219932 |
| $C^{5+}$ | -17.9962519 | -4.5429960 | -2.0429091 |
| $N^{6+}$ | -24.5003510 | -6.1782231 | -2.7746952 |
| $O^{7+}$ | -32.0047597 | -8.0637855 | -3.6174768 |
| $F^{8+}$ | -40.5093823 | -10.1996176 | -4.5713487 |
| $Ne^{9+}$ | -50.0141588 | -12.5856760 | -5.6264953 |
| $Na^{10+}$ | -60.5190496 | -15.2219165 | -6.8124955 |
| $Mg^{11+}$ | -72.0240274 | -18.1082992 | -8.0998462 |
| $Al^{12+}$ | -84.5290730 | -21.2448077 | -9.4982747 |
| $Si^{13+}$ | -98.0341723 | -24.6313918 | -11.0079034 |
| $P^{14+}$ | -112.5393149 | -28.2681009 | -12.6286990 |
| $S^{15+}$ | -128.0444930 | -32.1548705 | -14.3606442 |
| $Cl^{16+}$ | -144.5497003 | -36.2916950 | -16.2037591 |
| $Ar^{17+}$ | -162.0549321 | -40.6785717 | -18.1580363 |
| $K^{18+}$ | -180.5601845 | -45.3155478 | -20.2235086 |
| $Ca^{19+}$ | -200.0654545 | -50.2024418 | -22.4000891 |
| $Sc^{20+}$ | -220.5707396 | -55.3394351 | -24.6877113 |
| $Ti^{21+}$ | -242.0760377 | -60.7264358 | -27.0865851 |
| $V^{22+}$ | -264.5813472 | -66.3635280 | -29.5965103 |
| $Cr^{23+}$ | -288.0866665 | -72.2505967 | -32.2176746 |
| $Mn^{24+}$ | -312.5919945 | -78.3877010 | -34.9499087 |
| $Fe^{25+}$ | -338.0973302 | -84.7747946 | -37.7932249 |
| $Co^{26+}$ | -364.6026728 | -91.4119393 | -40.7477745 |
| $Ni^{27+}$ | -392.1080214 | -98.2990978 | -43.8133974 |
| $Cu^{28+}$ | -420.6133754 | -105.4362059 | -46.9900747 |
| $Zn^{29+}$ | -450.1187343 | -112.8234199 | -50.2779400 |
| $Ga^{30+}$ | -480.6240975 | -120.4606202 | -53.6769690 |
| $Ge^{31+}$ | -512.1294648 | -128.3478166 | -57.1871251 |
| $As^{32+}$ | -544.6348356 | -136.4850225 | -60.8083609 |
| $Se^{33+}$ | -578.1402097 | -144.8722372 | -64.5406446 |
| $Br^{34+}$ | -612.6455867 | -153.5094599 | -68.3841204 |
| $Kr^{35+}$ | -648.1509665 | -162.3966757 | -72.3387844 |

Table S48. Total energies for CAM-QTP01 for the 1$s$, 2$p$, and 3$d$ states calculated with PySCF using exponents from the AHGBSP3-9 basis set.

| System | $E_{\mathrm{tot}}^{1s}$ [$E_{\mathrm{h}}$] | $E_{\mathrm{tot}}^{2p}$ [$E_{\mathrm{h}}$] | $E_{\mathrm{tot}}^{3d}$ [$E_{\mathrm{h}}$] |
|---|---|---|---|
| $H^{0}$ | -0.4966515 | -0.1289352 | -0.0576005 |
| $He^{+}$ | -1.9824170 | -0.5093794 | -0.2277726 |
| $Li^{2+}$ | -4.4725481 | -1.1390626 | -0.5113699 |
| $Be^{3+}$ | -7.9655612 | -2.0186355 | -0.9067963 |
| $B^{4+}$ | -12.4601713 | -3.1487476 | -1.4133828 |
| $C^{5+}$ | -17.9557264 | -4.5295395 | -2.0310821 |
| $N^{6+}$ | -24.4518807 | -6.1609569 | -2.7599883 |
| $O^{7+}$ | -31.9484369 | -8.0429011 | -3.6001832 |
| $F^{8+}$ | -40.4452750 | -10.1752763 | -4.5517064 |
| $Ne^{9+}$ | -49.9423181 | -12.5580038 | -5.6063126 |
| $Na^{10+}$ | -60.4395145 | -15.1910202 | -6.7887949 |
| $Mg^{11+}$ | -71.9368286 | -18.0742765 | -8.0744072 |
| $Al^{12+}$ | -84.4342347 | -21.2077231 | -9.4712025 |
| $Si^{13+}$ | -97.9317141 | -24.5912823 | -10.9793636 |
| $P^{14+}$ | -112.4292527 | -28.2250885 | -12.5987592 |
| $S^{15+}$ | -127.9268398 | -32.1089674 | -14.3294207 |
| $Cl^{16+}$ | -144.4244671 | -36.2429436 | -16.1713358 |
| $Ar^{17+}$ | -161.9221279 | -40.6270080 | -18.1245238 |
| $K^{18+}$ | -180.4198171 | -45.2613402 | -20.1890773 |
| $Ca^{19+}$ | -199.9175303 | -50.1453176 | -22.3647189 |
| $Sc^{20+}$ | -220.4152643 | -55.2795700 | -24.6512858 |
| $Ti^{21+}$ | -241.9130160 | -60.6638026 | -27.0493131 |
| $V^{22+}$ | -264.4107831 | -66.2983107 | -29.5584268 |
| $Cr^{23+}$ | -287.9085638 | -72.1826869 | -32.1789049 |
| $Mn^{24+}$ | -312.4063562 | -78.3171622 | -34.9103623 |
| $Fe^{25+}$ | -337.9041591 | -84.7015364 | -37.7529901 |
| $Co^{26+}$ | -364.4019711 | -91.3360925 | -40.7069065 |
| $Ni^{27+}$ | -391.8997912 | -98.2206816 | -43.7719178 |
| $Cu^{28+}$ | -420.3976187 | -105.3550418 | -46.9479647 |
| $Zn^{29+}$ | -449.8954526 | -112.7397681 | -50.2348323 |
| $Ga^{30+}$ | -480.3932923 | -120.3744242 | -53.6337575 |
| $Ge^{31+}$ | -511.8911372 | -128.2590448 | -57.1434737 |
| $As^{32+}$ | -544.3889868 | -136.3936826 | -60.7642257 |
| $Se^{33+}$ | -577.8868407 | -144.7783361 | -64.4959980 |
| $Br^{34+}$ | -612.3846984 | -153.4130041 | -68.3389395 |
| $Kr^{35+}$ | -647.8825596 | -162.2975861 | -72.2933156 |

Table S49. Total energies for MN15 for the $1s$, $2p$, and $3d$ states calculated with PySCF using exponents from the AHGBSP3-9 basis set.

| System | $E^{1s}_{\mathrm{tot}}$ [$E_\mathrm{h}$] | $E^{2p}_{\mathrm{tot}}$ [$E_\mathrm{h}$] | $E^{3d}_{\mathrm{tot}}$ [$E_\mathrm{h}$] |
|---|---|---|---|
| $H^{0}$ | -0.4997444 | -0.1174902 | -0.0520838 |
| $He^{+}$ | -2.0070924 | -0.5044978 | -0.2219852 |
| $Li^{2+}$ | -4.5087299 | -1.1500047 | -0.5116759 |
| $Be^{3+}$ | -8.0082191 | -2.0459546 | -0.9174525 |
| $B^{4+}$ | -12.5069983 | -3.1907169 | -1.4371555 |
| $C^{5+}$ | -18.0055718 | -4.5841792 | -2.0695579 |
| $N^{6+}$ | -24.5041247 | -6.2265510 | -2.8141232 |
| $O^{7+}$ | -32.0027292 | -8.1180654 | -3.6703878 |
| $F^{8+}$ | -40.5014073 | -10.2589033 | -4.6383881 |
| $Ne^{9+}$ | -50.0001673 | -12.6492346 | -5.7049315 |
| $Na^{10+}$ | -60.4990067 | -15.2891823 | -6.9086963 |
| $Mg^{11+}$ | -71.9979188 | -18.1788010 | -8.2109852 |
| $Al^{12+}$ | -84.4968994 | -21.3181889 | -9.6244724 |
| $Si^{13+}$ | -97.9959424 | -24.7075250 | -11.1492098 |
| $P^{14+}$ | -112.4950415 | -28.3463958 | -12.7855372 |
| $S^{15+}$ | -127.9941915 | -32.2353319 | -14.5329173 |
| $Cl^{16+}$ | -144.4933883 | -36.3741497 | -16.3915261 |
| $Ar^{17+}$ | -161.9926278 | -40.7628884 | -18.3614490 |
| $K^{18+}$ | -180.4919065 | -45.4018079 | -20.4425523 |
| $Ca^{19+}$ | -199.9912208 | -50.2901512 | -22.6348774 |
| $Sc^{20+}$ | -220.4905688 | -55.4287289 | -24.9384104 |
| $Ti^{21+}$ | -241.9899467 | -60.8172742 | -27.3533239 |
| $V^{22+}$ | -264.4893530 | -66.4558331 | -29.8791691 |
| $Cr^{23+}$ | -287.9887843 | -72.3443013 | -32.5163433 |
| $Mn^{24+}$ | -312.4882409 | -78.4828083 | -35.2647981 |
| $Fe^{25+}$ | -337.9877199 | -84.8712393 | -38.1242974 |
| $Co^{26+}$ | -364.4872191 | -91.5096777 | -41.0950487 |
| $Ni^{27+}$ | -391.9867393 | -98.3981680 | -44.1769411 |
| $Cu^{28+}$ | -420.4862778 | -105.5365417 | -47.3698153 |
| $Zn^{29+}$ | -449.9858335 | -112.9249693 | -50.6742435 |
| $Ga^{30+}$ | -480.4854042 | -120.5634618 | -54.0894161 |
| $Ge^{31+}$ | -511.9849916 | -128.4518860 | -57.6162092 |
| $As^{32+}$ | -544.4845940 | -136.5903088 | -61.2539356 |
| $Se^{33+}$ | -577.9842114 | -144.9787308 | -65.0025585 |
| $Br^{34+}$ | -612.4838384 | -153.6171525 | -68.8625609 |
| $Kr^{35+}$ | -647.9834787 | -162.5055016 | -72.8340562 |

Table S50. Total energies for MN15-L for the 1$s$, 2$p$, and 3$d$ states calculated with PySCF using exponents from the AHGBSP3-9 basis set.

| System | $E^{1s}_{\mathrm{tot}}$ [$E_\mathrm{h}$] | $E^{2p}_{\mathrm{tot}}$ [$E_\mathrm{h}$] | $E^{3d}_{\mathrm{tot}}$ [$E_\mathrm{h}$] |
|---|---|---|---|
| $H^{0}$ | -0.4965965 | -0.1350988 | -0.0689992 |
| $He^{+}$ | -1.9941064 | -0.5144107 | -0.2421750 |
| $Li^{2+}$ | -4.4974954 | -1.1400581 | -0.5239951 |
| $Be^{3+}$ | -8.0066222 | -2.0125898 | -0.9149182 |
| $B^{4+}$ | -12.5203601 | -3.1331778 | -1.4156179 |
| $C^{5+}$ | -18.0376607 | -4.5026976 | -2.0263054 |
| $N^{6+}$ | -24.5577196 | -6.1217069 | -2.7475911 |
| $O^{7+}$ | -32.0799398 | -7.9905470 | -3.5790684 |
| $F^{8+}$ | -40.6038827 | -10.1094225 | -4.5220043 |
| $Ne^{9+}$ | -50.1292160 | -12.4784548 | -5.5655772 |
| $Na^{10+}$ | -60.6556895 | -15.0977115 | -6.7401775 |
| $Mg^{11+}$ | -72.1831105 | -17.9672287 | -8.0162066 |
| $Al^{12+}$ | -84.7113246 | -21.0870240 | -9.4032172 |
| $Si^{13+}$ | -98.2402116 | -24.4571086 | -10.9016456 |
| $P^{14+}$ | -112.7696763 | -28.0774514 | -12.5111837 |
| $S^{15+}$ | -128.2996374 | -31.9480678 | -14.2320625 |
| $Cl^{16+}$ | -144.8300308 | -36.0689416 | -16.0643076 |
| $Ar^{17+}$ | -162.3608016 | -40.4400585 | -18.0078478 |
| $K^{18+}$ | -180.8919060 | -45.0613838 | -20.0626261 |
| $Ca^{19+}$ | -200.4233039 | -49.9329719 | -22.2286592 |
| $Sc^{20+}$ | -220.9549659 | -55.0547413 | -24.5058676 |
| $Ti^{21+}$ | -242.4868611 | -60.4267102 | -26.8946836 |
| $V^{22+}$ | -265.0189668 | -66.0488355 | -29.3940804 |
| $Cr^{23+}$ | -288.5512628 | -71.9211467 | -32.0056641 |
| $Mn^{24+}$ | -313.0837303 | -78.0436113 | -34.7282919 |
| $Fe^{25+}$ | -338.6163544 | -84.4162327 | -37.5616708 |
| $Co^{26+}$ | -365.1491194 | -91.0389890 | -40.5070454 |
| $Ni^{27+}$ | -392.6820160 | -97.9118731 | -43.5633089 |
| $Cu^{28+}$ | -421.2150312 | -105.0348998 | -46.7307761 |
| $Zn^{29+}$ | -450.7481552 | -112.4080195 | -50.0089548 |
| $Ga^{30+}$ | -481.2813797 | -120.0312551 | -53.3995653 |
| $Ge^{31+}$ | -512.8146982 | -127.9045989 | -56.9008110 |
| $As^{32+}$ | -545.3481022 | -136.0280407 | -60.5132719 |
| $Se^{33+}$ | -578.8815886 | -144.4015754 | -64.2363344 |
| $Br^{34+}$ | -613.4151454 | -153.0251978 | -68.0714329 |
| $Kr^{35+}$ | -648.9487733 | -161.8989050 | -72.0179817 |

Table S51. Total energies for LC-QTP for the $1s$, $2p$, and $3d$ states calculated with PySCF using exponents from the AHGBSP3-9 basis set.

| System | $E_{\mathrm{tot}}^{1s}$ [$E_{\mathrm{h}}$] | $E_{\mathrm{tot}}^{2p}$ [$E_{\mathrm{h}}$] | $E_{\mathrm{tot}}^{3d}$ [$E_{\mathrm{h}}$] |
|---|---|---|---|
| $H^{0}$ | -0.4951915 | -0.1256064 | -0.0556271 |
| $He^{+}$ | -1.9739964 | -0.5050029 | -0.2235535 |
| $Li^{2+}$ | -4.4542883 | -1.1357779 | -0.5052809 |
| $Be^{3+}$ | -7.9390887 | -2.0159934 | -0.9004392 |
| $B^{4+}$ | -12.4271828 | -3.1459462 | -1.4079025 |
| $C^{5+}$ | -17.9174894 | -4.5261597 | -2.0269085 |
| $N^{6+}$ | -24.4093095 | -6.1569185 | -2.7571358 |
| $O^{7+}$ | -31.9022002 | -8.0383177 | -3.5985085 |
| $F^{8+}$ | -40.3958726 | -10.1703525 | -4.5510504 |
| $Ne^{9+}$ | -49.8901327 | -12.5529751 | -5.6056382 |
| $Na^{10+}$ | -60.3848453 | -15.1861233 | -6.7898391 |
| $Mg^{11+}$ | -71.8799138 | -18.0697375 | -8.0761771 |
| $Al^{12+}$ | -84.3752673 | -21.2037545 | -9.4738083 |
| $Si^{13+}$ | -97.8708527 | -24.5881033 | -10.9828130 |
| $P^{14+}$ | -112.3666292 | -28.2228120 | -12.6030671 |
| $S^{15+}$ | -127.8625653 | -32.1077708 | -14.3346863 |
| $Cl^{16+}$ | -144.3586361 | -36.2429686 | -16.1776018 |
| $Ar^{17+}$ | -161.8548214 | -40.6283786 | -18.1318775 |
| $K^{18+}$ | -180.3511052 | -45.2641402 | -20.1975429 |
| $Ca^{19+}$ | -199.8474742 | -50.1497310 | -22.3744022 |
| $Sc^{20+}$ | -220.3439175 | -55.2856429 | -24.6623432 |
| $Ti^{21+}$ | -241.8404258 | -60.6715904 | -27.0617127 |
| $V^{22+}$ | -264.3369916 | -66.3078805 | -29.5723239 |
| $Cr^{23+}$ | -287.8336083 | -72.1941605 | -32.1943578 |
| $Mn^{24+}$ | -312.3302703 | -78.3305409 | -34.9273110 |
| $Fe^{25+}$ | -337.8269730 | -84.7169409 | -37.7716203 |
| $Co^{26+}$ | -364.3237121 | -91.3535451 | -40.7272001 |
| $Ni^{27+}$ | -391.8204842 | -98.2401893 | -43.7939685 |
| $Cu^{28+}$ | -420.3172861 | -105.3766659 | -46.9718747 |
| $Zn^{29+}$ | -449.8141150 | -112.7636114 | -50.2610808 |
| $Ga^{30+}$ | -480.3109686 | -120.4004601 | -53.6614683 |
| $Ge^{31+}$ | -511.8078447 | -128.2873305 | -57.1730516 |
| $As^{32+}$ | -544.3047415 | -136.4242504 | -60.7957973 |
| $Se^{33+}$ | -577.8016572 | -144.8112162 | -64.5300241 |
| $Br^{34+}$ | -612.2985904 | -153.4482247 | -68.3747123 |
| $Kr^{35+}$ | -647.7955398 | -162.3352029 | -72.3311007 |

Table S52. Total energies for CAM-QTP02 for the $1s$, $2p$, and $3d$ states calculated with PySCF using exponents from the AHGBSP3-9 basis set.

| System | $E_{\mathrm{tot}}^{1s}$ [$E_{\mathrm{h}}$] | $E_{\mathrm{tot}}^{2p}$ [$E_{\mathrm{h}}$] | $E_{\mathrm{tot}}^{3d}$ [$E_{\mathrm{h}}$] |
|---|---|---|---|
| $H^{0}$ | -0.4934067 | -0.1260133 | -0.0557254 |
| $He^{+}$ | -1.9782734 | -0.5050078 | -0.2244802 |
| $Li^{2+}$ | -4.4674118 | -1.1337609 | -0.5067923 |
| $Be^{3+}$ | -7.9596271 | -2.0123896 | -0.9012296 |
| $B^{4+}$ | -12.4536126 | -3.1414869 | -1.4069867 |
| $C^{5+}$ | -17.9486720 | -4.5212328 | -2.0238968 |
| $N^{6+}$ | -24.4444260 | -6.1516036 | -2.7520031 |
| $O^{7+}$ | -31.9406541 | -8.0325164 | -3.5913734 |
| $F^{8+}$ | -40.4372203 | -10.1638820 | -4.5420508 |
| $Ne^{9+}$ | -49.9340359 | -12.5456233 | -5.5965461 |
| $Na^{10+}$ | -60.4310411 | -15.1776743 | -6.7774027 |
| $Mg^{11+}$ | -71.9281938 | -18.0599873 | -8.0621198 |
| $Al^{12+}$ | -84.4254635 | -21.1925106 | -9.4580525 |
| $Si^{13+}$ | -97.9228279 | -24.5751745 | -10.9653275 |
| $P^{14+}$ | -112.4202697 | -28.2080828 | -12.5838717 |
| $S^{15+}$ | -127.9177759 | -32.0910837 | -14.3136648 |
| $Cl^{16+}$ | -144.4153361 | -36.2241977 | -16.1547239 |
| $Ar^{17+}$ | -161.9129421 | -40.6074119 | -18.1070464 |
| $K^{18+}$ | -180.4105874 | -45.2408867 | -20.1707302 |
| $Ca^{19+}$ | -199.9082665 | -50.1240615 | -22.3455193 |
| $Sc^{20+}$ | -220.4059751 | -55.2574966 | -24.6312763 |
| $Ti^{21+}$ | -241.9037093 | -60.6409202 | -27.0284577 |
| $V^{22+}$ | -264.4014662 | -66.2746080 | -29.5367597 |
| $Cr^{23+}$ | -287.8992432 | -72.1581949 | -32.1564037 |
| $Mn^{24+}$ | -312.3970379 | -78.2918706 | -34.8870393 |
| $Fe^{25+}$ | -337.8948486 | -84.6754735 | -37.7288653 |
| $Co^{26+}$ | -364.3926735 | -91.3092470 | -40.6819639 |
| $Ni^{27+}$ | -391.8905113 | -98.1930506 | -43.7461724 |
| $Cu^{28+}$ | -420.3883607 | -105.3266543 | -46.9214409 |
| $Zn^{29+}$ | -449.8862207 | -112.7106107 | -50.2080942 |
| $Ga^{30+}$ | -480.3840903 | -120.3444973 | -53.6056524 |
| $Ge^{31+}$ | -511.8819686 | -128.2283608 | -57.1145590 |
| $As^{32+}$ | -544.3798550 | -136.3622452 | -60.7345282 |
| $Se^{33+}$ | -577.8777487 | -144.7461488 | -64.4655501 |
| $Br^{34+}$ | -612.3756492 | -153.3800702 | -68.3077189 |
| $Kr^{35+}$ | -647.8735560 | -162.2639193 | -72.2612897 |

Table S53. Total energies for QTP17 for the 1$s$, 2$p$, and 3$d$ states calculated with PySCF using exponents from the AHGBSP3-9 basis set.

| System | $E_{\mathrm{tot}}^{1s}$ $[E_{\mathrm{h}}]$ | $E_{\mathrm{tot}}^{2p}$ $[E_{\mathrm{h}}]$ | $E_{\mathrm{tot}}^{3d}$ $[E_{\mathrm{h}}]$ |
|---|---|---|---|
| $H^{0}$ | -0.4912732 | -0.1282177 | -0.0599372 |
| $He^{+}$ | -1.9762300 | -0.5024978 | -0.2281370 |
| $Li^{2+}$ | -4.4604668 | -1.1261934 | -0.5069804 |
| $Be^{3+}$ | -7.9443923 | -1.9996270 | -0.8967055 |
| $B^{4+}$ | -12.4281422 | -3.1229059 | -1.3974085 |
| $C^{5+}$ | -17.9117790 | -4.4960842 | -2.0091343 |
| $N^{6+}$ | -24.3953367 | -6.1191919 | -2.7319075 |
| $O^{7+}$ | -31.8788359 | -7.9922470 | -3.5657442 |
| $F^{8+}$ | -40.3622900 | -10.1152602 | -4.5106513 |
| $Ne^{9+}$ | -49.8457083 | -12.4882410 | -5.5630085 |
| $Na^{10+}$ | -60.3290976 | -15.1111967 | -6.7337245 |
| $Mg^{11+}$ | -71.8124626 | -17.9841274 | -8.0119048 |
| $Al^{12+}$ | -84.2958073 | -21.1070408 | -9.4011495 |
| $Si^{13+}$ | -97.7791346 | -24.4799307 | -10.9015107 |
| $P^{14+}$ | -112.2624469 | -28.1028174 | -12.5129592 |
| $S^{15+}$ | -127.7457460 | -31.9756890 | -14.2355165 |
| $Cl^{16+}$ | -144.2290336 | -36.0985479 | -16.0691683 |
| $Ar^{17+}$ | -161.7123109 | -40.4713971 | -18.0139307 |
| $K^{18+}$ | -180.1955790 | -45.0942510 | -20.0697709 |
| $Ca^{19+}$ | -199.6788388 | -49.9670669 | -22.2367784 |
| $Sc^{20+}$ | -220.1620912 | -55.0898920 | -24.5148256 |
| $Ti^{21+}$ | -241.6453369 | -60.4627052 | -26.9040087 |
| $V^{22+}$ | -264.1285763 | -66.0855283 | -29.4042782 |
| $Cr^{23+}$ | -287.6118101 | -71.9583342 | -32.0156614 |
| $Mn^{24+}$ | -312.0950386 | -78.0811390 | -34.7381658 |
| $Fe^{25+}$ | -337.5782624 | -84.4539317 | -37.5717530 |
| $Co^{26+}$ | -364.0614817 | -91.0767282 | -40.5164701 |
| $Ni^{27+}$ | -391.5446969 | -97.9495213 | -43.5722832 |
| $Cu^{28+}$ | -420.0279082 | -105.0722947 | -46.7391878 |
| $Zn^{29+}$ | -449.5111160 | -112.4450870 | -50.0172158 |
| $Ga^{30+}$ | -479.9943204 | -120.0678702 | -53.4063600 |
| $Ge^{31+}$ | -511.4775216 | -127.9406469 | -56.9066133 |
| $As^{32+}$ | -543.9607199 | -136.0634207 | -60.5179664 |
| $Se^{33+}$ | -577.4439155 | -144.4361918 | -64.2404143 |
| $Br^{34+}$ | -611.9271084 | -153.0589604 | -68.0739879 |
| $Kr^{35+}$ | -647.4102988 | -161.9317232 | -72.0186773 |

Table S54. Total energies for rSCAN for the 1$s$, 2$p$, and 3$d$ states calculated with PySCF using exponents from the AHGBSP3-9 basis set.

| System | $E_{\mathrm{tot}}^{1s}$ [$E_{\mathrm{h}}$] | $E_{\mathrm{tot}}^{2p}$ [$E_{\mathrm{h}}$] | $E_{\mathrm{tot}}^{3d}$ [$E_{\mathrm{h}}$] |
|---|---|---|---|
| $H^{0}$ | -0.5001732 | -0.1338407 | -0.0636703 |
| $He^{+}$ | -2.0001627 | -0.5174778 | -0.2378732 |
| $Li^{2+}$ | -4.5001585 | -1.1511154 | -0.5232174 |
| $Be^{3+}$ | -8.0001557 | -2.0347561 | -0.9196681 |
| $B^{4+}$ | -12.5001534 | -3.1683952 | -1.4272325 |
| $C^{5+}$ | -18.0001513 | -4.5520336 | -2.0459082 |
| $N^{6+}$ | -24.5001495 | -6.1856732 | -2.7756970 |
| $O^{7+}$ | -32.0001477 | -8.0693142 | -3.6166012 |
| $F^{8+}$ | -40.5001460 | -10.2029524 | -4.5686019 |
| $Ne^{9+}$ | -50.0001443 | -12.5865924 | -5.6207392 |
| $Na^{10+}$ | -60.5001426 | -15.2202350 | -6.8059680 |
| $Mg^{11+}$ | -72.0001410 | -18.1038741 | -8.0913504 |
| $Al^{12+}$ | -84.5001394 | -21.2375147 | -9.4877743 |
| $Si^{13+}$ | -98.0001378 | -24.6211412 | -10.9953565 |
| $P^{14+}$ | -112.5001362 | -28.2547919 | -12.6140074 |
| $S^{15+}$ | -128.0001346 | -32.1384343 | -14.3437903 |
| $Cl^{16+}$ | -144.5001330 | -36.2720742 | -16.1846883 |
| $Ar^{17+}$ | -162.0001314 | -40.6557140 | -18.1367122 |
| $K^{18+}$ | -180.5001299 | -45.2893852 | -20.1998934 |
| $Ca^{19+}$ | -200.0001283 | -50.1729884 | -22.3741377 |
| $Sc^{20+}$ | -220.5001267 | -55.3066275 | -24.6594135 |
| $Ti^{21+}$ | -242.0001251 | -60.6902525 | -27.0558873 |
| $V^{22+}$ | -264.5001236 | -66.3239134 | -29.5634379 |
| $Cr^{23+}$ | -288.0001220 | -72.2075511 | -32.1821528 |
| $Mn^{24+}$ | -312.5001204 | -78.3411931 | -34.9119247 |
| $Fe^{25+}$ | -338.0001188 | -84.7248234 | -37.7528058 |
| $Co^{26+}$ | -364.5001172 | -91.3584693 | -40.7048385 |
| $Ni^{27+}$ | -392.0001157 | -98.2421126 | -43.7679621 |
| $Cu^{28+}$ | -420.5001141 | -105.3757249 | -46.9421659 |
| $Zn^{29+}$ | -450.0001125 | -112.7593860 | -50.2274543 |
| $Ga^{30+}$ | -480.5001109 | -120.3930322 | -53.6239825 |
| $Ge^{31+}$ | -512.0001093 | -128.2766720 | -57.1315675 |
| $As^{32+}$ | -544.5001077 | -136.4103118 | -60.7502467 |
| $Se^{33+}$ | -578.0001062 | -144.7939517 | -64.4800193 |
| $Br^{34+}$ | -612.5001046 | -153.4275915 | -68.3209136 |
| $Kr^{35+}$ | -648.0001030 | -162.3112278 | -72.2729508 |

Table S55. Total energies for TASK for the 1$s$, 2$p$, and 3$d$ states calculated with PySCF using exponents from the AHGBSP3-9 basis set.

| System | $E^{1s}_{\rm tot}$ [$E_{\rm h}$] | $E^{2p}_{\rm tot}$ [$E_{\rm h}$] | $E^{3d}_{\rm tot}$ [$E_{\rm h}$] |
|---|---|---|---|
| $H^{0}$ | -0.5223243 | -0.1475022 | -0.0733635 |
| $He^{+}$ | -2.0296319 | -0.5365586 | -0.2517057 |
| $Li^{2+}$ | -4.5343689 | -1.1739581 | -0.5400952 |
| $Be^{3+}$ | -8.0379096 | -2.0605132 | -0.9389760 |
| $B^{4+}$ | -12.5407481 | -3.1965431 | -1.4485747 |
| $C^{5+}$ | -18.0431220 | -4.5822148 | -2.0690055 |
| $N^{6+}$ | -24.5451645 | -6.2176268 | -2.8003411 |
| $O^{7+}$ | -32.0469583 | -8.1028408 | -3.6426310 |
| $F^{8+}$ | -40.5485583 | -10.2378939 | -4.5958833 |
| $Ne^{9+}$ | -50.0500028 | -12.6228210 | -5.6488548 |
| $Na^{10+}$ | -60.5513198 | -15.2576446 | -6.8354614 |
| $Mg^{11+}$ | -72.0525302 | -18.1423747 | -8.1218296 |
| $Al^{12+}$ | -84.5536501 | -21.2770302 | -9.5191706 |
| $Si^{13+}$ | -98.0546923 | -24.6616042 | -11.0276156 |
| $P^{14+}$ | -112.5556670 | -28.2961459 | -12.6470769 |
| $S^{15+}$ | -128.0565824 | -32.1806279 | -14.3776274 |
| $Cl^{16+}$ | -144.5574455 | -36.3150616 | -16.2192537 |
| $Ar^{17+}$ | -162.0582619 | -40.6994546 | -18.1719710 |
| $K^{18+}$ | -180.5590365 | -45.3338436 | -20.2358152 |
| $Ca^{19+}$ | -200.0597733 | -50.2181286 | -22.4106919 |
| $Sc^{20+}$ | -220.5604759 | -55.3524208 | -24.6965697 |
| $Ti^{21+}$ | -242.0611474 | -60.7366711 | -27.0936252 |
| $V^{22+}$ | -264.5617904 | -66.3709332 | -29.6017326 |
| $Cr^{23+}$ | -288.0624072 | -72.2551478 | -32.2209862 |
| $Mn^{24+}$ | -312.5629999 | -78.3893456 | -34.9512761 |
| $Fe^{25+}$ | -338.0635704 | -84.7735110 | -37.7926561 |
| $Co^{26+}$ | -364.5641202 | -91.4076742 | -40.7451739 |
| $Ni^{27+}$ | -392.0646507 | -98.2918176 | -43.8087656 |
| $Cu^{28+}$ | -420.5651634 | -105.4259125 | -46.9834212 |
| $Zn^{29+}$ | -450.0656593 | -112.8100429 | -50.2691889 |
| $Ga^{30+}$ | -480.5661396 | -120.4441436 | -53.6661054 |
| $Ge^{31+}$ | -512.0666052 | -128.3282244 | -57.1741068 |
| $As^{32+}$ | -544.5670569 | -136.4622927 | -60.7931896 |
| $Se^{33+}$ | -578.0674956 | -144.8463491 | -64.5233526 |
| $Br^{34+}$ | -612.5679219 | -153.4803942 | -68.3646305 |
| $Kr^{35+}$ | -648.0683367 | -162.3644238 | -72.3170422 |

Table S56. Total energies for r$^2$SCAN for the 1$s$, 2$p$, and 3$d$ states calculated with PySCF using exponents from the AHGBSP3-9 basis set.

| System | $E_{\mathrm{tot}}^{1s}$ [$E_{\mathrm{h}}$] | $E_{\mathrm{tot}}^{2p}$ [$E_{\mathrm{h}}$] | $E_{\mathrm{tot}}^{3d}$ [$E_{\mathrm{h}}$] |
|---|---|---|---|
| $H^{0}$ | -0.5001732 | -0.1338407 | -0.0636703 |
| $He^{+}$ | -2.0001627 | -0.5174778 | -0.2378734 |
| $Li^{2+}$ | -4.5001585 | -1.1511140 | -0.5232174 |
| $Be^{3+}$ | -8.0001557 | -2.0347561 | -0.9196681 |
| $B^{4+}$ | -12.5001534 | -3.1683952 | -1.4272327 |
| $C^{5+}$ | -18.0001513 | -4.5520336 | -2.0459082 |
| $N^{6+}$ | -24.5001495 | -6.1856732 | -2.7756969 |
| $O^{7+}$ | -32.0001477 | -8.0693142 | -3.6165966 |
| $F^{8+}$ | -40.5001460 | -10.2029524 | -4.5686015 |
| $Ne^{9+}$ | -50.0001443 | -12.5865924 | -5.6207392 |
| $Na^{10+}$ | -60.5001426 | -15.2202350 | -6.8059679 |
| $Mg^{11+}$ | -72.0001410 | -18.1038741 | -8.0913505 |
| $Al^{12+}$ | -84.5001394 | -21.2375147 | -9.4877743 |
| $Si^{13+}$ | -98.0001378 | -24.6211412 | -10.9953393 |
| $P^{14+}$ | -112.5001362 | -28.2547919 | -12.6140071 |
| $S^{15+}$ | -128.0001346 | -32.1384343 | -14.3437935 |
| $Cl^{16+}$ | -144.5001330 | -36.2720742 | -16.1846761 |
| $Ar^{17+}$ | -162.0001314 | -40.6557140 | -18.1367098 |
| $K^{18+}$ | -180.5001299 | -45.2893852 | -20.1998815 |
| $Ca^{19+}$ | -200.0001283 | -50.1729884 | -22.3741306 |
| $Sc^{20+}$ | -220.5001267 | -55.3066275 | -24.6594137 |
| $Ti^{21+}$ | -242.0001251 | -60.6902525 | -27.0558873 |
| $V^{22+}$ | -264.5001236 | -66.3239134 | -29.5634359 |
| $Cr^{23+}$ | -288.0001220 | -72.2075511 | -32.1821120 |
| $Mn^{24+}$ | -312.5001204 | -78.3411931 | -34.9119247 |
| $Fe^{25+}$ | -338.0001188 | -84.7248234 | -37.7528069 |
| $Co^{26+}$ | -364.5001172 | -91.3584693 | -40.7048385 |
| $Ni^{27+}$ | -392.0001157 | -98.2421126 | -43.7679621 |
| $Cu^{28+}$ | -420.5001141 | -105.3757249 | -46.9421673 |
| $Zn^{29+}$ | -450.0001125 | -112.7593860 | -50.2275494 |
| $Ga^{30+}$ | -480.5001109 | -120.3930322 | -53.6239597 |
| $Ge^{31+}$ | -512.0001093 | -128.2766720 | -57.1315675 |
| $As^{32+}$ | -544.5001077 | -136.4103118 | -60.7502467 |
| $Se^{33+}$ | -578.0001062 | -144.7939517 | -64.4800188 |
| $Br^{34+}$ | -612.5001046 | -153.4275915 | -68.3209117 |
| $Kr^{35+}$ | -648.0001030 | -162.3112266 | -72.2729508 |

Table S57. Total energies for DM21 for the 1$s$, 2$p$, and 3$d$ states calculated with PySCF using exponents from the AHGBSP3-9 basis set.

| System | $E_{\mathrm{tot}}^{1s}$ [$E_\mathrm{h}$] | $E_{\mathrm{tot}}^{2p}$ [$E_\mathrm{h}$] | $E_{\mathrm{tot}}^{3d}$ [$E_\mathrm{h}$] |
|---|---|---|---|
| $H^{0}$ | -0.5011876 | -0.1320135 | -0.0639673 |
| $He^{+}$ | -1.9999601 | -0.5071767 | -0.2310236 |
| $Li^{2+}$ | -4.5021871 | -1.1373114 | -0.5076555 |
| $Be^{3+}$ | -8.0029936 | -2.0220282 | -0.8980597 |
| $B^{4+}$ | -12.4911113 | -3.1553557 | -1.4005737 |
| $C^{5+}$ | -17.9659502 | -4.5391287 | -2.0202475 |
| $N^{6+}$ | -24.4320855 | -6.1746442 | -2.7509151 |
| $O^{7+}$ | -31.8942217 | -8.0615975 | -3.5932504 |
| $F^{8+}$ | -40.3556196 | -10.1995875 | -4.5466867 |
| $Ne^{9+}$ | -49.8180703 | -12.5876166 | -5.6046141 |
| $Na^{10+}$ | -60.2823698 | -15.2241983 | -6.7868173 |
| $Mg^{11+}$ | -71.7487852 | -18.1085999 | -8.0749376 |
| $Al^{12+}$ | -84.2172697 | -21.2407955 | -9.4744370 |
| $Si^{13+}$ | -97.6875700 | -24.6208470 | -10.9852006 |
| $P^{14+}$ | -112.1593159 | -28.2488021 | -12.6072357 |
| $S^{15+}$ | -127.6321323 | -32.1248837 | -14.3406907 |
| $Cl^{16+}$ | -144.1056875 | -36.2491795 | -16.1855155 |
| $Ar^{17+}$ | -161.5797248 | -40.6218770 | -18.1413586 |
| $K^{18+}$ | -180.0540587 | -45.2431364 | -20.2078993 |
| $Ca^{19+}$ | -199.5285681 | -50.1135563 | -22.3855945 |
| $Sc^{20+}$ | -220.0031773 | -55.2330792 | -24.6732144 |
| $Ti^{21+}$ | -241.4778422 | -60.6020416 | -27.0713804 |
| $V^{22+}$ | -263.9525327 | -66.2205108 | -29.5797922 |
| $Cr^{23+}$ | -287.4272312 | -72.0888109 | -32.1986313 |
| $Mn^{24+}$ | -311.9019225 | -78.2069723 | -34.9274676 |
| $Fe^{25+}$ | -337.3765968 | -84.5751803 | -37.7669579 |
| $Co^{26+}$ | -363.8512499 | -91.1934342 | -40.7167385 |
| $Ni^{27+}$ | -391.3258783 | -98.0618412 | -43.7770916 |
| $Cu^{28+}$ | -419.8004773 | -105.1805901 | -46.9480899 |
| $Zn^{29+}$ | -449.2750441 | -112.5495253 | -50.2295918 |
| $Ga^{30+}$ | -479.7495813 | -120.1687922 | -53.6215500 |
| $Ge^{31+}$ | -511.2240872 | -128.0383724 | -57.1241977 |
| $As^{32+}$ | -543.6985619 | -136.1582506 | -60.7375283 |
| $Se^{33+}$ | -577.1730077 | -144.5284292 | -64.4617008 |
| $Br^{34+}$ | -611.6474240 | -153.1488793 | -68.2963236 |
| $Kr^{35+}$ | -647.1218121 | -162.0196491 | -72.2416375 |

Table S58. Total energies for rSCANh for the 1$s$, 2$p$, and 3$d$ states calculated with PySCF using exponents from the AHGBSP3-9 basis set.

| System | $E^{1s}_{\mathrm{tot}}$ [$E_{\mathrm{h}}$] | $E^{2p}_{\mathrm{tot}}$ [$E_{\mathrm{h}}$] | $E^{3d}_{\mathrm{tot}}$ [$E_{\mathrm{h}}$] |
|---|---|---|---|
| $H^{0}$ | -0.5001386 | -0.1329381 | -0.0628054 |
| $He^{+}$ | -2.0001308 | -0.5157120 | -0.2362593 |
| $Li^{2+}$ | -4.5001275 | -1.1484847 | -0.5208482 |
| $Be^{3+}$ | -8.0001252 | -2.0312627 | -0.9165435 |
| $B^{4+}$ | -12.5001233 | -3.1640379 | -1.4233518 |
| $C^{5+}$ | -18.0001216 | -4.5468125 | -2.0412713 |
| $N^{6+}$ | -24.5001200 | -6.1795882 | -2.7703036 |
| $O^{7+}$ | -32.0001184 | -8.0623651 | -3.6104509 |
| $F^{8+}$ | -40.5001169 | -10.1951395 | -4.5616960 |
| $Ne^{9+}$ | -50.0001154 | -12.5779155 | -5.6141845 |
| $Na^{10+}$ | -60.5001139 | -15.2106938 | -6.7975479 |
| $Mg^{11+}$ | -72.0001125 | -18.0934690 | -8.0821699 |
| $Al^{12+}$ | -84.5001110 | -21.2262455 | -9.4778404 |
| $Si^{13+}$ | -98.0001096 | -24.6090094 | -10.9846433 |
| $P^{14+}$ | -112.5001082 | -28.2417950 | -12.6025613 |
| $S^{15+}$ | -128.0001068 | -32.1245732 | -14.3315882 |
| $Cl^{16+}$ | -144.5001053 | -36.2573491 | -16.1717298 |
| $Ar^{17+}$ | -162.0001039 | -40.6401250 | -18.1229957 |
| $K^{18+}$ | -180.5001025 | -45.2729290 | -20.1854143 |
| $Ca^{19+}$ | -200.0001011 | -50.1556719 | -22.3588987 |
| $Sc^{20+}$ | -220.5000997 | -55.2884470 | -24.6434270 |
| $Ti^{21+}$ | -242.0000982 | -60.6712096 | -27.0391423 |
| $V^{22+}$ | -264.5000968 | -66.3040043 | -29.5459360 |
| $Cr^{23+}$ | -288.0000954 | -72.1867723 | -32.1638666 |
| $Mn^{24+}$ | -312.5000940 | -78.3195561 | -34.8929092 |
| $Fe^{25+}$ | -338.0000926 | -84.7023234 | -37.7330356 |
| $Co^{26+}$ | -364.5000911 | -91.3351046 | -40.6843095 |
| $Ni^{27+}$ | -392.0000897 | -98.2178836 | -43.7466763 |
| $Cu^{28+}$ | -420.5000883 | -105.3506347 | -46.9201264 |
| $Zn^{29+}$ | -450.0000869 | -112.7334297 | -50.2047666 |
| $Ga^{30+}$ | -480.5000854 | -120.3662112 | -53.6004280 |
| $Ge^{31+}$ | -512.0000840 | -128.2489871 | -57.1072545 |
| $As^{32+}$ | -544.5000825 | -136.3817629 | -60.7251768 |
| $Se^{33+}$ | -578.0000811 | -144.7645387 | -64.4540869 |
| $Br^{34+}$ | -612.5000797 | -153.3973146 | -68.2943272 |
| $Kr^{35+}$ | -648.0000782 | -162.2800859 | -72.2456105 |

Table S59. Total energies for r$^2$SCANh for the 1$s$, 2$p$, and 3$d$ states calculated with PySCF using exponents from the AHGBSP3-9 basis set.

| System | $E^{1s}_{\mathrm{tot}}$ [$E_\mathrm{h}$] | $E^{2p}_{\mathrm{tot}}$ [$E_\mathrm{h}$] | $E^{3d}_{\mathrm{tot}}$ [$E_\mathrm{h}$] |
|---|---|---|---|
| $H^{0}$ | -0.5001386 | -0.1329381 | -0.0628054 |
| $He^{+}$ | -2.0001308 | -0.5157120 | -0.2362595 |
| $Li^{2+}$ | -4.5001275 | -1.1484847 | -0.5208482 |
| $Be^{3+}$ | -8.0001252 | -2.0312627 | -0.9165435 |
| $B^{4+}$ | -12.5001233 | -3.1640379 | -1.4233523 |
| $C^{5+}$ | -18.0001216 | -4.5468125 | -2.0412713 |
| $N^{6+}$ | -24.5001200 | -6.1795882 | -2.7703035 |
| $O^{7+}$ | -32.0001184 | -8.0623651 | -3.6104472 |
| $F^{8+}$ | -40.5001169 | -10.1951395 | -4.5616956 |
| $Ne^{9+}$ | -50.0001154 | -12.5779155 | -5.6141845 |
| $Na^{10+}$ | -60.5001139 | -15.2106938 | -6.7975478 |
| $Mg^{11+}$ | -72.0001125 | -18.0934690 | -8.0821701 |
| $Al^{12+}$ | -84.5001110 | -21.2262455 | -9.4778404 |
| $Si^{13+}$ | -98.0001096 | -24.6090094 | -10.9846487 |
| $P^{14+}$ | -112.5001082 | -28.2417950 | -12.6025617 |
| $S^{15+}$ | -128.0001068 | -32.1245732 | -14.3315912 |
| $Cl^{16+}$ | -144.5001053 | -36.2573491 | -16.1717424 |
| $Ar^{17+}$ | -162.0001039 | -40.6401250 | -18.1229935 |
| $K^{18+}$ | -180.5001025 | -45.2729290 | -20.1854143 |
| $Ca^{19+}$ | -200.0001011 | -50.1556719 | -22.3588945 |
| $Sc^{20+}$ | -220.5000997 | -55.2884470 | -24.6434271 |
| $Ti^{21+}$ | -242.0000982 | -60.6712096 | -27.0391423 |
| $V^{22+}$ | -264.5000968 | -66.3040043 | -29.5459378 |
| $Cr^{23+}$ | -288.0000954 | -72.1867783 | -32.1638534 |
| $Mn^{24+}$ | -312.5000940 | -78.3195561 | -34.8929092 |
| $Fe^{25+}$ | -338.0000926 | -84.7023234 | -37.7330364 |
| $Co^{26+}$ | -364.5000911 | -91.3351046 | -40.6843095 |
| $Ni^{27+}$ | -392.0000897 | -98.2178836 | -43.7466763 |
| $Cu^{28+}$ | -420.5000883 | -105.3506347 | -46.9201275 |
| $Zn^{29+}$ | -450.0000869 | -112.7334297 | -50.2047459 |
| $Ga^{30+}$ | -480.5000854 | -120.3662112 | -53.6004099 |
| $Ge^{31+}$ | -512.0000840 | -128.2489871 | -57.1072545 |
| $As^{32+}$ | -544.5000825 | -136.3817629 | -60.7251768 |
| $Se^{33+}$ | -578.0000811 | -144.7645387 | -64.4541940 |
| $Br^{34+}$ | -612.5000797 | -153.3973146 | -68.2943323 |
| $Kr^{35+}$ | -648.0000782 | -162.2800862 | -72.2456105 |

Table S60. Total energies for rSCAN0 for the $1s$, $2p$, and $3d$ states calculated with PySCF using exponents from the AHGBSP3-9 basis set.

| System | $E_{\mathrm{tot}}^{1s}$ [$E_\mathrm{h}$] | $E_{\mathrm{tot}}^{2p}$ [$E_\mathrm{h}$] | $E_{\mathrm{tot}}^{3d}$ [$E_\mathrm{h}$] |
|---|---|---|---|
| $H^{0}$ | -0.5000945 | -0.1315921 | -0.0615319 |
| $He^{+}$ | -2.0000898 | -0.5130709 | -0.2338592 |
| $Li^{2+}$ | -4.5000876 | -1.1445483 | -0.5173147 |
| $Be^{3+}$ | -8.0000859 | -2.0260300 | -0.9118763 |
| $B^{4+}$ | -12.5000844 | -3.1575094 | -1.4175504 |
| $C^{5+}$ | -18.0000831 | -4.5389883 | -2.0343354 |
| $N^{6+}$ | -24.5000818 | -6.1704680 | -2.7622328 |
| $O^{7+}$ | -32.0000805 | -8.0519488 | -3.6012446 |
| $F^{8+}$ | -40.5000793 | -10.1834274 | -4.5513564 |
| $Ne^{9+}$ | -50.0000781 | -12.5649075 | -5.6043678 |
| $Na^{10+}$ | -60.5000769 | -15.1963894 | -6.7849368 |
| $Mg^{11+}$ | -72.0000757 | -18.0778687 | -8.0684182 |
| $Al^{12+}$ | -84.5000745 | -21.2093492 | -9.4629585 |
| $Si^{13+}$ | -98.0000733 | -24.5908191 | -10.9686326 |
| $P^{14+}$ | -112.5000722 | -28.2223071 | -12.5854113 |
| $S^{15+}$ | -128.0000710 | -32.1037889 | -14.3133040 |
| $Cl^{16+}$ | -144.5000698 | -36.2352688 | -16.1523109 |
| $Ar^{17+}$ | -162.0000686 | -40.6167487 | -18.1024382 |
| $K^{18+}$ | -180.5000674 | -45.2482520 | -20.1637147 |
| $Ca^{19+}$ | -200.0000662 | -50.1297048 | -22.3360609 |
| $Sc^{20+}$ | -220.5000651 | -55.2611841 | -24.6194663 |
| $Ti^{21+}$ | -242.0000639 | -60.6426525 | -27.0140436 |
| $V^{22+}$ | -264.5000627 | -66.2741481 | -29.5197065 |
| $Cr^{23+}$ | -288.0000615 | -72.1556264 | -32.1364950 |
| $Mn^{24+}$ | -312.5000603 | -78.2871079 | -34.8644050 |
| $Fe^{25+}$ | -338.0000591 | -84.6685806 | -37.7033991 |
| $Co^{26+}$ | -364.5000579 | -91.3000650 | -40.6535348 |
| $Ni^{27+}$ | -392.0000567 | -98.1815475 | -43.7147664 |
| $Cu^{28+}$ | -420.5000555 | -105.3130067 | -46.8870867 |
| $Zn^{29+}$ | -450.0000543 | -112.6945025 | -50.1705824 |
| $Ga^{30+}$ | -480.5000531 | -120.3259871 | -53.5651150 |
| $Ge^{31+}$ | -512.0000519 | -128.2074670 | -57.0708038 |
| $As^{32+}$ | -544.5000507 | -136.3389468 | -60.6875909 |
| $Se^{33+}$ | -578.0000495 | -144.7204267 | -64.4154758 |
| $Br^{34+}$ | -612.5000483 | -153.3519065 | -68.2544755 |
| $Kr^{35+}$ | -648.0000471 | -162.2333820 | -72.2046190 |

Table S61. Total energies for r$^2$SCAN0 for the 1$s$, 2$p$, and 3$d$ states calculated with PySCF using exponents from the AHGBSP3-9 basis set.

| System | $E_{\mathrm{tot}}^{1s}$ [$E_{\mathrm{h}}$] | $E_{\mathrm{tot}}^{2p}$ [$E_{\mathrm{h}}$] | $E_{\mathrm{tot}}^{3d}$ [$E_{\mathrm{h}}$] |
|---|---|---|---|
| $H^{0}$ | -0.5000945 | -0.1315921 | -0.0615319 |
| $He^{+}$ | -2.0000898 | -0.5130709 | -0.2338595 |
| $Li^{2+}$ | -4.5000876 | -1.1445483 | -0.5173147 |
| $Be^{3+}$ | -8.0000859 | -2.0260300 | -0.9118763 |
| $B^{4+}$ | -12.5000844 | -3.1575094 | -1.4175507 |
| $C^{5+}$ | -18.0000831 | -4.5389883 | -2.0343354 |
| $N^{6+}$ | -24.5000818 | -6.1704680 | -2.7622328 |
| $O^{7+}$ | -32.0000805 | -8.0519483 | -3.6012398 |
| $F^{8+}$ | -40.5000793 | -10.1834275 | -4.5513560 |
| $Ne^{9+}$ | -50.0000781 | -12.5649077 | -5.6043678 |
| $Na^{10+}$ | -60.5000769 | -15.1963894 | -6.7849368 |
| $Mg^{11+}$ | -72.0000757 | -18.0778687 | -8.0684182 |
| $Al^{12+}$ | -84.5000745 | -21.2093492 | -9.4629585 |
| $Si^{13+}$ | -98.0000733 | -24.5908191 | -10.9686319 |
| $P^{14+}$ | -112.5000722 | -28.2223071 | -12.5854110 |
| $S^{15+}$ | -128.0000710 | -32.1037889 | -14.3133065 |
| $Cl^{16+}$ | -144.5000698 | -36.2352688 | -16.1523211 |
| $Ar^{17+}$ | -162.0000686 | -40.6167487 | -18.1024379 |
| $K^{18+}$ | -180.5000674 | -45.2482520 | -20.1637154 |
| $Ca^{19+}$ | -200.0000662 | -50.1297045 | -22.3360593 |
| $Sc^{20+}$ | -220.5000651 | -55.2611837 | -24.6194661 |
| $Ti^{21+}$ | -242.0000639 | -60.6426525 | -27.0140436 |
| $V^{22+}$ | -264.5000627 | -66.2741481 | -29.5197051 |
| $Cr^{23+}$ | -288.0000615 | -72.1556264 | -32.1364873 |
| $Mn^{24+}$ | -312.5000603 | -78.2871079 | -34.8644050 |
| $Fe^{25+}$ | -338.0000591 | -84.6685806 | -37.7033995 |
| $Co^{26+}$ | -364.5000579 | -91.3000650 | -40.6535348 |
| $Ni^{27+}$ | -392.0000567 | -98.1815475 | -43.7147664 |
| $Cu^{28+}$ | -420.5000555 | -105.3130067 | -46.8870867 |
| $Zn^{29+}$ | -450.0000543 | -112.6945025 | -50.1705581 |
| $Ga^{30+}$ | -480.5000531 | -120.3259871 | -53.5651219 |
| $Ge^{31+}$ | -512.0000519 | -128.2074670 | -57.0708038 |
| $As^{32+}$ | -544.5000507 | -136.3389468 | -60.6875909 |
| $Se^{33+}$ | -578.0000495 | -144.7204267 | -64.4154754 |
| $Br^{34+}$ | -612.5000483 | -153.3519065 | -68.2544755 |
| $Kr^{35+}$ | -648.0000471 | -162.2333829 | -72.2046190 |

Table S62. Total energies for rSCAN50 for the $1s$, $2p$, and $3d$ states calculated with PySCF using exponents from the AHGBSP3-9 basis set.

| System | $E_{\rm tot}^{1s}$ [$E_{\rm h}$] | $E_{\rm tot}^{2p}$ [$E_{\rm h}$] | $E_{\rm tot}^{3d}$ [$E_{\rm h}$] |
|---|---|---|---|
| $H^{0}$ | -0.5000407 | -0.1293695 | -0.0594700 |
| $He^{+}$ | -2.0000389 | -0.5086891 | -0.2299147 |
| $Li^{2+}$ | -4.5000378 | -1.1380075 | -0.5114785 |
| $Be^{3+}$ | -8.0000369 | -2.0173287 | -0.9041498 |
| $B^{4+}$ | -12.5000361 | -3.1466483 | -1.4079343 |
| $C^{5+}$ | -18.0000353 | -4.5259676 | -2.0228269 |
| $N^{6+}$ | -24.5000344 | -6.1552875 | -2.7488324 |
| $O^{7+}$ | -32.0000337 | -8.0346077 | -3.5859498 |
| $F^{8+}$ | -40.5000329 | -10.1639271 | -4.5341744 |
| $Ne^{9+}$ | -50.0000321 | -12.5432473 | -5.5880469 |
| $Na^{10+}$ | -60.5000313 | -15.1725684 | -6.7639691 |
| $Mg^{11+}$ | -72.0000305 | -18.0518879 | -8.0455492 |
| $Al^{12+}$ | -84.5000297 | -21.1812082 | -9.4382058 |
| $Si^{13+}$ | -98.0000289 | -24.5605215 | -10.9419882 |
| $P^{14+}$ | -112.5000281 | -28.1898468 | -12.5568780 |
| $S^{15+}$ | -128.0000273 | -32.0691680 | -14.2828835 |
| $Cl^{16+}$ | -144.5000265 | -36.1984879 | -16.1199946 |
| $Ar^{17+}$ | -162.0000257 | -40.5778078 | -18.0682292 |
| $K^{18+}$ | -180.5000249 | -45.2071434 | -20.1276015 |
| $Ca^{19+}$ | -200.0000241 | -50.0864450 | -22.2980515 |
| $Sc^{20+}$ | -220.5000233 | -55.2157645 | -24.5795813 |
| $Ti^{21+}$ | -242.0000225 | -60.5950770 | -26.9722626 |
| $V^{22+}$ | -264.5000217 | -66.2244074 | -29.4760370 |
| $Cr^{23+}$ | -288.0000209 | -72.1037262 | -32.0909296 |
| $Mn^{24+}$ | -312.5000201 | -78.2330472 | -34.8169480 |
| $Fe^{25+}$ | -338.0000193 | -84.6123623 | -37.6540549 |
| $Co^{26+}$ | -364.5000185 | -91.2416852 | -40.6022938 |
| $Ni^{27+}$ | -392.0000177 | -98.1210069 | -43.6616333 |
| $Cu^{28+}$ | -420.5000168 | -105.2503130 | -46.8320689 |
| $Zn^{29+}$ | -450.0000160 | -112.6296435 | -50.1136426 |
| $Ga^{30+}$ | -480.5000152 | -120.2589665 | -53.5063102 |
| $Ge^{31+}$ | -512.0000144 | -128.1382864 | -57.0101027 |
| $As^{32+}$ | -544.5000135 | -136.2676063 | -60.6249978 |
| $Se^{33+}$ | -578.0000127 | -144.6469262 | -64.3509948 |
| $Br^{34+}$ | -612.5000118 | -153.2762460 | -68.1881060 |
| $Kr^{35+}$ | -648.0000110 | -162.1555634 | -72.1363498 |

Table S63. Total energies for r$^2$SCAN50 for the 1$s$, 2$p$, and 3$d$ states calculated with PySCF using exponents from the AHGBSP3-9 basis set.

| System | $E_{\text{tot}}^{1s}$ [$E_\text{h}$] | $E_{\text{tot}}^{2p}$ [$E_\text{h}$] | $E_{\text{tot}}^{3d}$ [$E_\text{h}$] |
|---|---|---|---|
| $H^{0}$ | -0.5000407 | -0.1293695 | -0.0594700 |
| $He^{+}$ | -2.0000389 | -0.5086891 | -0.2299147 |
| $Li^{2+}$ | -4.5000378 | -1.1380075 | -0.5114785 |
| $Be^{3+}$ | -8.0000369 | -2.0173287 | -0.9041498 |
| $B^{4+}$ | -12.5000361 | -3.1466483 | -1.4079328 |
| $C^{5+}$ | -18.0000353 | -4.5259676 | -2.0228269 |
| $N^{6+}$ | -24.5000344 | -6.1552875 | -2.7488328 |
| $O^{7+}$ | -32.0000337 | -8.0346077 | -3.5859499 |
| $F^{8+}$ | -40.5000329 | -10.1639271 | -4.5341741 |
| $Ne^{9+}$ | -50.0000321 | -12.5432473 | -5.5880469 |
| $Na^{10+}$ | -60.5000313 | -15.1725684 | -6.7639691 |
| $Mg^{11+}$ | -72.0000305 | -18.0518879 | -8.0455493 |
| $Al^{12+}$ | -84.5000297 | -21.1812082 | -9.4382058 |
| $Si^{13+}$ | -98.0000289 | -24.5605215 | -10.9419878 |
| $P^{14+}$ | -112.5000281 | -28.1898468 | -12.5568778 |
| $S^{15+}$ | -128.0000273 | -32.0691680 | -14.2828960 |
| $Cl^{16+}$ | -144.5000265 | -36.1984879 | -16.1199942 |
| $Ar^{17+}$ | -162.0000257 | -40.5778078 | -18.0682289 |
| $K^{18+}$ | -180.5000249 | -45.2071434 | -20.1275565 |
| $Ca^{19+}$ | -200.0000241 | -50.0864450 | -22.2980507 |
| $Sc^{20+}$ | -220.5000233 | -55.2157645 | -24.5795814 |
| $Ti^{21+}$ | -242.0000225 | -60.5950770 | -26.9722626 |
| $V^{22+}$ | -264.5000217 | -66.2244074 | -29.4760370 |
| $Cr^{23+}$ | -288.0000209 | -72.1037262 | -32.0909284 |
| $Mn^{24+}$ | -312.5000201 | -78.2330472 | -34.8169480 |
| $Fe^{25+}$ | -338.0000193 | -84.6123623 | -37.6540549 |
| $Co^{26+}$ | -364.5000185 | -91.2416852 | -40.6022938 |
| $Ni^{27+}$ | -392.0000177 | -98.1210069 | -43.6616333 |
| $Cu^{28+}$ | -420.5000168 | -105.2503130 | -46.8320686 |
| $Zn^{29+}$ | -450.0000160 | -112.6296435 | -50.1136215 |
| $Ga^{30+}$ | -480.5000152 | -120.2589665 | -53.5063101 |
| $Ge^{31+}$ | -512.0000144 | -128.1382864 | -57.0101027 |
| $As^{32+}$ | -544.5000135 | -136.2676063 | -60.6249978 |
| $Se^{33+}$ | -578.0000127 | -144.6469262 | -64.3509944 |
| $Br^{34+}$ | -612.5000118 | -153.2762460 | -68.1881089 |
| $Kr^{35+}$ | -648.0000110 | -162.1555635 | -72.1363498 |

Table S64. Total energies for UHF for the $1s$, $2p$, and $3d$ states calculated with PySCF using exponents from the AHGBSP3-9 basis set.

| System | $E_{\mathrm{tot}}^{1s}$ $[E_{\mathrm{h}}]$ | $E_{\mathrm{tot}}^{2p}$ $[E_{\mathrm{h}}]$ | $E_{\mathrm{tot}}^{3d}$ $[E_{\mathrm{h}}]$ |
|---|---|---|---|
| $H^{0}$ | -0.5000000 | -0.1250000 | -0.0555556 |
| $He^{+}$ | -2.0000000 | -0.5000000 | -0.2222222 |
| $Li^{2+}$ | -4.5000000 | -1.1250000 | -0.5000000 |
| $Be^{3+}$ | -8.0000000 | -2.0000000 | -0.8888889 |
| $B^{4+}$ | -12.5000000 | -3.1250000 | -1.3888889 |
| $C^{5+}$ | -18.0000000 | -4.5000000 | -2.0000000 |
| $N^{6+}$ | -24.4999999 | -6.1249999 | -2.7222222 |
| $O^{7+}$ | -31.9999999 | -7.9999999 | -3.5555555 |
| $F^{8+}$ | -40.4999999 | -10.1249999 | -4.4999999 |
| $Ne^{9+}$ | -49.9999999 | -12.4999999 | -5.5555554 |
| $Na^{10+}$ | -60.4999998 | -15.1249998 | -6.7222221 |
| $Mg^{11+}$ | -71.9999998 | -17.9999998 | -7.9999998 |
| $Al^{12+}$ | -84.4999998 | -21.1249998 | -9.3888887 |
| $Si^{13+}$ | -97.9999997 | -24.4999997 | -10.8888887 |
| $P^{14+}$ | -112.4999997 | -28.1249997 | -12.4999997 |
| $S^{15+}$ | -127.9999997 | -31.9999997 | -14.2222219 |
| $Cl^{16+}$ | -144.4999996 | -36.1249996 | -16.0555552 |
| $Ar^{17+}$ | -161.9999996 | -40.4999996 | -17.9999996 |
| $K^{18+}$ | -180.4999995 | -45.1249995 | -20.0555551 |
| $Ca^{19+}$ | -199.9999995 | -49.9999995 | -22.2222218 |
| $Sc^{20+}$ | -220.4999994 | -55.1249994 | -24.4999995 |
| $Ti^{21+}$ | -241.9999993 | -60.4999994 | -26.8888883 |
| $V^{22+}$ | -264.4999993 | -66.1249993 | -29.3888883 |
| $Cr^{23+}$ | -287.9999992 | -71.9999992 | -31.9999994 |
| $Mn^{24+}$ | -312.4999991 | -78.1249992 | -34.7222215 |
| $Fe^{25+}$ | -337.9999991 | -84.4999991 | -37.5555548 |
| $Co^{26+}$ | -364.4999990 | -91.1249990 | -40.4999992 |
| $Ni^{27+}$ | -391.9999989 | -97.9999990 | -43.5555547 |
| $Cu^{28+}$ | -420.4999989 | -105.1249989 | -46.7222213 |
| $Zn^{29+}$ | -449.9999988 | -112.4999988 | -49.9999990 |
| $Ga^{30+}$ | -480.4999987 | -120.1249987 | -53.3888878 |
| $Ge^{31+}$ | -511.9999986 | -127.9999986 | -56.8888877 |
| $As^{32+}$ | -544.4999985 | -136.1249985 | -60.4999988 |
| $Se^{33+}$ | -577.9999984 | -144.4999985 | -64.2222209 |
| $Br^{34+}$ | -612.4999983 | -153.1249984 | -68.0555542 |
| $Kr^{35+}$ | -647.9999982 | -161.9999983 | -71.9999985 |
